# Supplementary material for: CalliReader: Contextualizing Chinese Calligraphy via an Embedding-Aligned Vision-Language Model
Source: arXiv:2503.06472 source file (2025-03-12)
Supplement: Supplementary file 1 [file X_supp.tex]

\section{\textit{OrderFormer}}
\subsection{Overview}
Recognizing the correct text sequence is critical for text comprehension and various applications. Previous methods primarily relied on rule-based approaches, such as assuming a top-to-bottom, left-to-right reading order. However, the reading sequences in Chinese calligraphy often deviate significantly from this structure, presenting challenges for purely rule-based methods. Observing that individuals can deduce the reading order of calligraphy pieces based solely on character layout—even without knowing the characters—we hypothesize that the reading order can be inferred from bounding box arrangements alone, without understanding the content. This problem aligns well with a sequence-to-sequence task, making a Transformer-based model an appropriate choice.

The \textit{OrderFormer} model in our \textit{CalliDecode} system is designed to sort columns of calligraphy rather than individual characters. Typically, a single piece contains fewer than 50 columns, though the character count may vary from a few to hundreds. Character bounding boxes have much greater variability than column bounding boxes, making direct sorting of characters challenging. Thus, we assume that within each column, characters follow a top-to-bottom order. For a given input of character bounding boxes, a rule-based algorithm clusters these into column boxes, which are then sequenced using OrderFormer. The character order is subsequently reconstructed based on this sorted column layout, effectively “downsampling” the problem to reduce complexity while retaining accuracy. This approach combines the advantages of learning-based and rule-based methods, optimizing both robustness and precision.

\subsection{Preprocessing}
Sorting bounding boxes according to the correct reading order is of great complexity since the distribution of bounding boxes can vary from one calligraphy work to another. Yet we have proposed multiple processing methods to reduce the complexity of the problem.

\textbf{Shifting} is utilized to eliminate the complexity caused by translation. In cases where the bounding boxes in one instance are merely translated in a specific direction compared to another instance, the classification results should remain unchanged. Therefore, for images that exhibit such translational relationships, it is unnecessary to learn from all of them. Learning from just one typical instance would suffice. 

In \textit{OrderFormer}, for each bounding box, we revise its coordinates from 
\begin{equation}
   (x_1,y_1,x_2,y_2) 
\end{equation}
to
\begin{equation}
   (x_1-x_{min},y_1-y_{min},x_2-x_{min},y_2-y_{min})
\end{equation} where $x_{min}$ denotes the minimum x-coordinate value of all the bounding boxes, and similarly $y_{min}$ represents the minimum y-coordinate value. This shifting method maps different images that have translational relationships to a same image, reducing the complexity of the model's hypothesis space.

\textbf{Scaling} is used for reducing the complexity caused by image resolutions. For one calligraphy artwork, different image sizes should not affect the ordering of its bounding boxes. At the same time, the resolution of different calligraphy artwork images may vary significantly. Directly inputting absolute coordinates could lead to instability in the results, Therefore, after shifting, we further revise the coordinates from \begin{equation}
    (x_1-x_{min},y_1-y_{min},x_2-x_{min},y_2-y_{min})
\end{equation}
to
\begin{equation}
    (\frac{x_1-x_{min}}{W},\frac{y_1-y_{min}}{H},\frac{x_2-x_{min}}{W},\frac{y_2-y_{min}}{H})
\end{equation}
where $W$ is the width of the image and $H$ is the height of the image. This technique maps the coordinate value range to [0,1], improving numerical stability and reducing variability in layout sizes, while preserving the correct reading order.

\textbf{Pre-sorting} is applied to boxes that have been transformed through shifting and scaling to eliminate the complexity of input ordering. Specifically, for the same sample, if the order of input boxes differs, the classification result should remain consistent. Therefore, a rule-based pre-sorting method is defined to ensure that the order of boxes for the same image is always identical during input. We utilize this method to ensure that the input sequence follows a specific ordering rule, and that neighboring boxes remain close to each other in the input.

After preprocessing, the input is transformed into a tensor with the shape of $(B,N,d)$, where $B$ represents the batch size, $N$ represents the maximum length of a single sample, and $d$ represents the feature vector dimension, and d represents the dimension of a feature vector. Specifically, $d=4$, representing the preprocessed bounding box coordinates.

%\begin{figure*}
%  \centering
%\includegraphics[width=0.8\linewidth]{preprocessing.JPG} % Adjust width as needed
%    \caption{An illustration of preprocessing. It performs shifting, scaling, presorting on the original input. It should be mentioned that presorting cannot perfectly sort the boxes, but it helps to reduce the complexity of the input, while also reducing the learning burden on the model. Through these operations, many different box layouts can be mapped to similar inputs.  }
%    \label{fig:order}
%\end{figure*}

The entire process can be visually represented in 
\cref{fig:order}. Along with the aforementioned three methods, this approach consolidates many seemingly different inputs into identical ones, reducing the complexity of the hypothesis space and alleviating the model's learning burden. This preprocessing step plays a crucial role in improving the model's performance and ensuring consistency across various bounding box sequences.

\subsection{Model Architecture}
The key component of \textit{OrderFormer} is an encoder-only Transformer model with four encoder layers, in which layer normalization is applied to ensure the stability. No decoder is used because this problem doesn't require autoregressive, step-by-step generation of the output sequence. Instead, it requires attention to all the bounding boxes to obtain the sorted result.

The output of the model is a tensor with the shape of $(B,N,1)$, with the last dimension representing the sorted index for every bounding box in a single sample. To be more specific, let $(B_1,B_2,\dots,B_n)$ denotes a sequence of bounding boxes, and $f$ represents the mapping learned by the model, and then the output can be represented as   
\begin{equation}
f((B_1,B_2,\dots,B_n))=(id_1,id_2,\dots,id_n)   
\end{equation}
where $id_j$ indicates the index in the correct reading order of the $j$-th box  order in the input sequence. 

\subsection{Training and Inference}

Due to the lack of authentic calligraphy data annotated with bounding boxes and correct reading orders, we generate synthetic data to train \textit{OrderFormer}. During training, we apply Mean Squared Error Loss (MSELoss) to approximate the correct reading order. MSELoss helps localize sorting errors, meaning that if a box is misordered, adjustments are often needed only for nearby boxes, making fine-tuning easier.

The model is optimized using AdamW with a learning rate of $2e^{-4}$, zero weight decay, and amsgrad set to true. We employ a CosineAnnealingWarmRestarts scheduler with $T_0=10$, $T_{mult}=2$, and $eta\_min=1e^{-6}$ for learning rate control. The batch size is set to 4, and the model is trained on 57,627 samples for 1000 epochs. These samples feature diverse calligraphy layouts to ensure comprehensive learning of the layout-to-order mapping.

We set the maximum sequence length $N = 50$, as most calligraphy works contain no more than 50 columns. For shorter sequences, padding is applied using the vector $[0, 0, 0, 0]$.

Since there lacks authentic calligraphy data annotated with both bounding boxes and correct reading orders, synthesized data is generated for training \textit{OrderFormer}. In training, Mean Squared Loss (MSELoss) is applied to ensure the output can approximate the correct order. MSELoss causes errors to tend toward localization, meaning that if the sorting of a particular box is incorrect, boxes that need adjustment in the sorted result are often near this box, making it convenient to further adjust the result. We use the AdamW optimizer with a learning rate of $2e^{-4}$ and weight decay of 0, setting amsgrad as true. CosineAnnealingWarmRestarts scheduler with a $T_0=10$, $T_{mult}=2$, $eta\_min=1e^{-6}$, is used for controlling the learning rate in training. We set the batch size as 4 and train the model on 57627 samples for 1000 epochs. These samples contain various types of calligraphy layouts to ensure that the model fully capture and learn the mapping between the layout and the reading order. 
We set N to 50, as most calligraphy works do not have more than 50 columns. For shorter sequences, we use $[0, 0, 0, 0]$ for padding.

During the inference stage, to recover the correct reading order from the model output, positions corresponding to padding tokens ($[0, 0, 0, 0]$) are removed. Then, the value at each position in the output sequence is mapped to its corresponding index in the sorted sequence. For example, if the output is $[2.1,0.3,1.2,4.4,0.1,-0.1]$, and the length of the original bounding boxes sequence is 4, then the result will be $[2,0,1,3]$, since the last two values are ignored. This process provides the model with a fault-tolerant margin, as it doesn't require the exact sorted indices to be output. It only needs to preserve the relative order of the values, allowing the model's output to vary within a certain range without affecting the final result.

\section{Detailed Experiments}
\begin{table}[t]
    \centering
    \begin{small}
    \begin{tabular}{lcc}
        \toprule
        Method & AR* & CR*\\
        \midrule
        Det + Recog & 94.50 & 95.29\\
        PageNet & 93.76 & 95.23 \\
        \rowcolor{lightgray} CalliReader & &\\
        FOTS & 87.97 &89.25 \\
        Start-Follow-Read & 69.54 & 73.11\\
        OrigamiNet & 9.72 & 9.83 \\
        \bottomrule
    \end{tabular}
    \end{small}
    \vspace{-3mm}
    \caption{MTHv2}
    \label{tab:mthv2_test}
    \vspace{-3mm}
\end{table}

\subsection{Test on Historical Document Dataset}
To further validate the generalizability of our method, we selected the test set of the historical document dataset MTHv2. This dataset comprises Buddhist scriptures and printed book pages, characterized by a high word count and small font size, which adds complexity. We tested CalliReader+e-IT and compared it with prevalent page-level OCR methods, using the widely-adopted AR* and CR* metrics; results are shown in Table~\ref{tab:mthv2_test}. Even without task-specific fine-tuning, our method demonstrates notable performance. We also note that MTHv2 contains a significant number of labels beyond those learned by \textit{CalliAlign}; targeted fine-tuning on MTHv2 would likely yield even better results.

\subsection{Ablation Studies}

\noindent\textbf{Ablation on CalliAlign.}
We evaluated several implementations of the CalliAlign framework, comparing configurations that utilized a two-layer resampler module, global normalization, and additional custom loss functions. Specifically, we designed a custom ratio\_loss (detailed below) and incorporated CRDLoss inspired by contrastive distillation~\cite{tian2019contrastive,khosla2020supervised}. The formulation are showned in Equation~\ref{eq:crd}.
\begin{equation} 
\begin{aligned}
\mathcal{L}_{\text{Ratio}}= w\cdot \frac{1}{N}\sum^{N}_{i=1}(\frac{|y_{i}-\hat{y}_{i}|}{|y_{i}|+eps})+\frac{1}{N}\sum^{N}_{i=1}(y_{i}-\hat{y}_{i})^{2}). \\
\mathcal{L}_{\text{CRD}}= \sum_{i \in I} \frac{-1}{|P(i)|} \sum_{p \in P(i)} \log \frac{\exp(z_i \cdot z_p / \tau)}{\sum_{a \in A(i)} \exp(z_i \cdot z_a / \tau)}.
\label{eq:crd}
\end{aligned}
\end{equation}

As for our custom ratio\_loss, we first define the deviation ratio as $\frac{1}{N}\sum^{N}_{i=1}(\frac{|y_{i}-\hat{y}_{i}|}{|y_{i}|+eps})$, where $\hat{y}$ is the output of the module and $y$ is the corresponding ground-truth, with $N$ respresenting the number of elements in tensor $y$ and eps representing a small positive value to avoid division by zero. We then define a weight $w=\frac{\tau}{T}\cdot (w_{max}-w_{min}) +w_{min}$, in which $T$ is the total iterations of the training process and $\tau$ is the current iteration number. $w_{min}$ and $w_{max}$ are pre-defined values such that $0 < w_{min} < w_{max} <1$.

In the training process, the weight for deviation ratio will linearly increase from $w_{min}$ to $w_{max}$. Thus at the early stage of training, module will converge coarsely yet rapidly with the MSELoss term. Later the module will learn to approximate more precisely since the deviation ratio will measure relative rather than absolute differences between $y$ and $\hat{y}$. Despite with layer-normalization, numeric values in embeddings still fluctuate, so a simple MSELoss will be likely to make the module to pay more attention to those regions with larger values, ignoring those with smaller ones. Deviation ratio is expected to force the module to pay more attention to those smaller values.

\section{More visualizations}
\subsection{Full-page ocr results}

\begin{figure*}[t!]
    \centering
    \includegraphics[width=\linewidth]{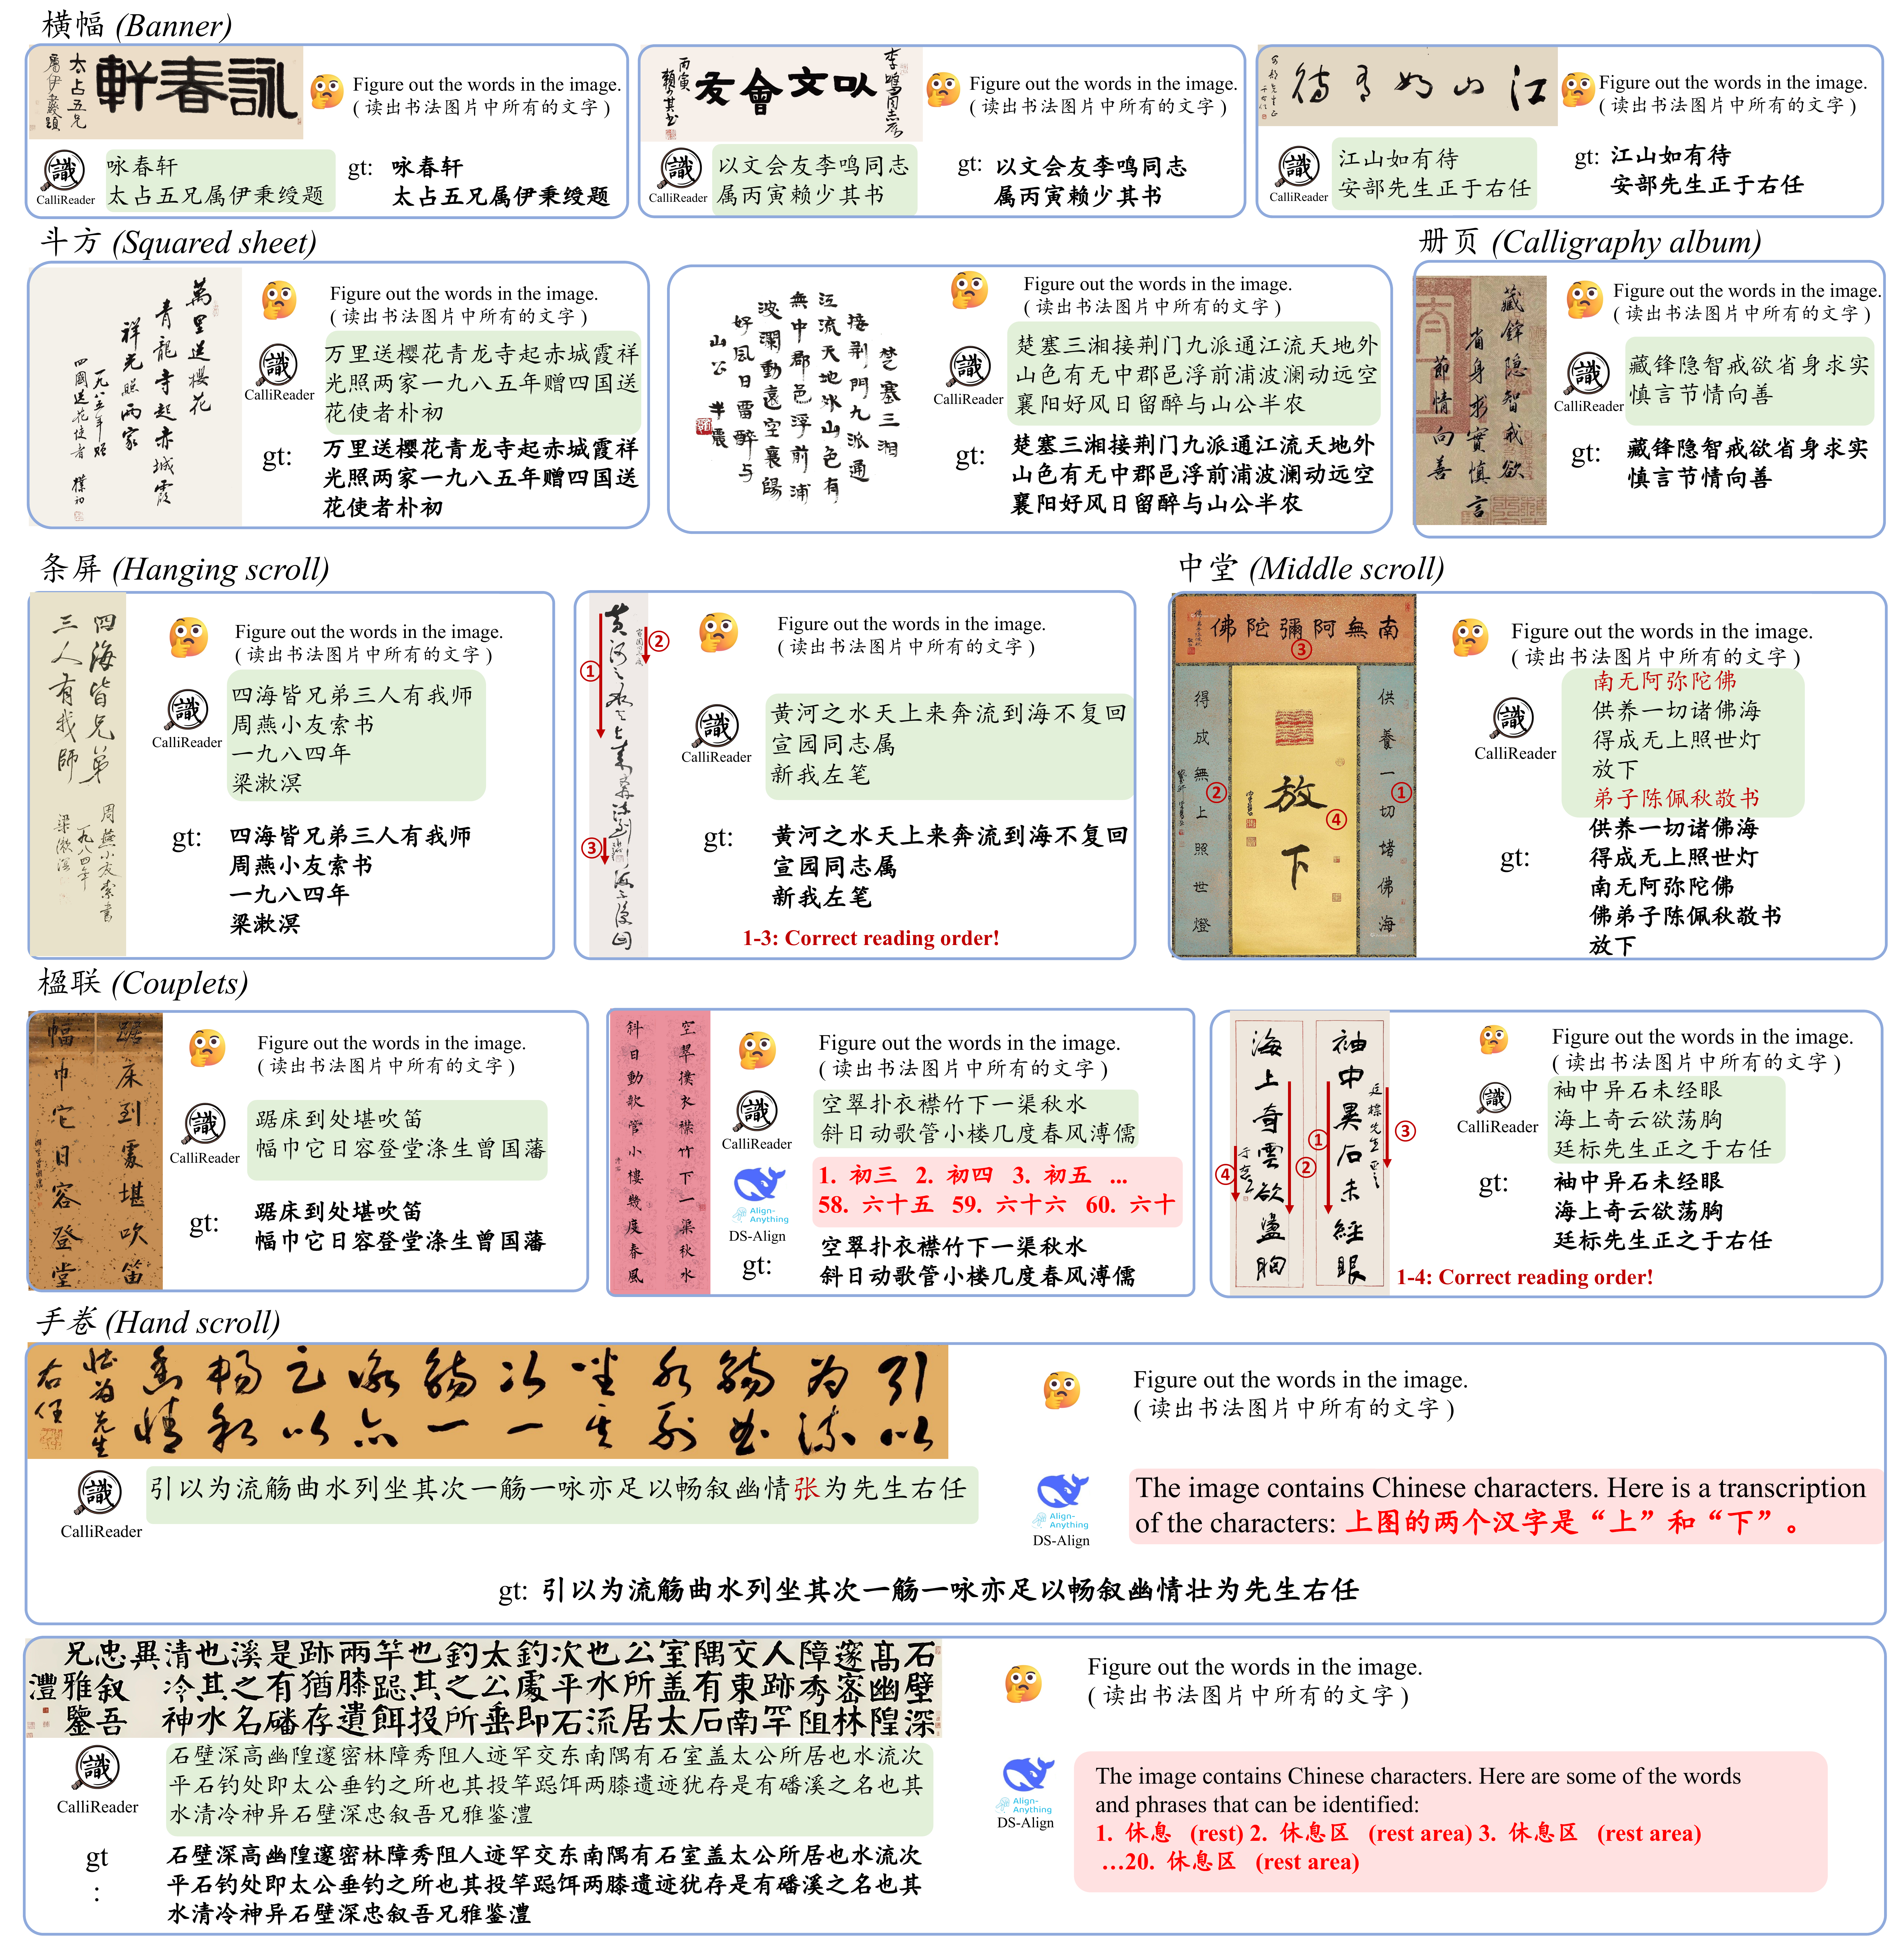}
    \vspace{-8mm}
    \caption{More full-page ocr results on diverse styles and layouts.}
    \label{fig:supp_styles}
\end{figure*}

\subsection{Region-wise ocr results}

\begin{figure*}[t!]
    \centering
    \includegraphics[width=\linewidth]{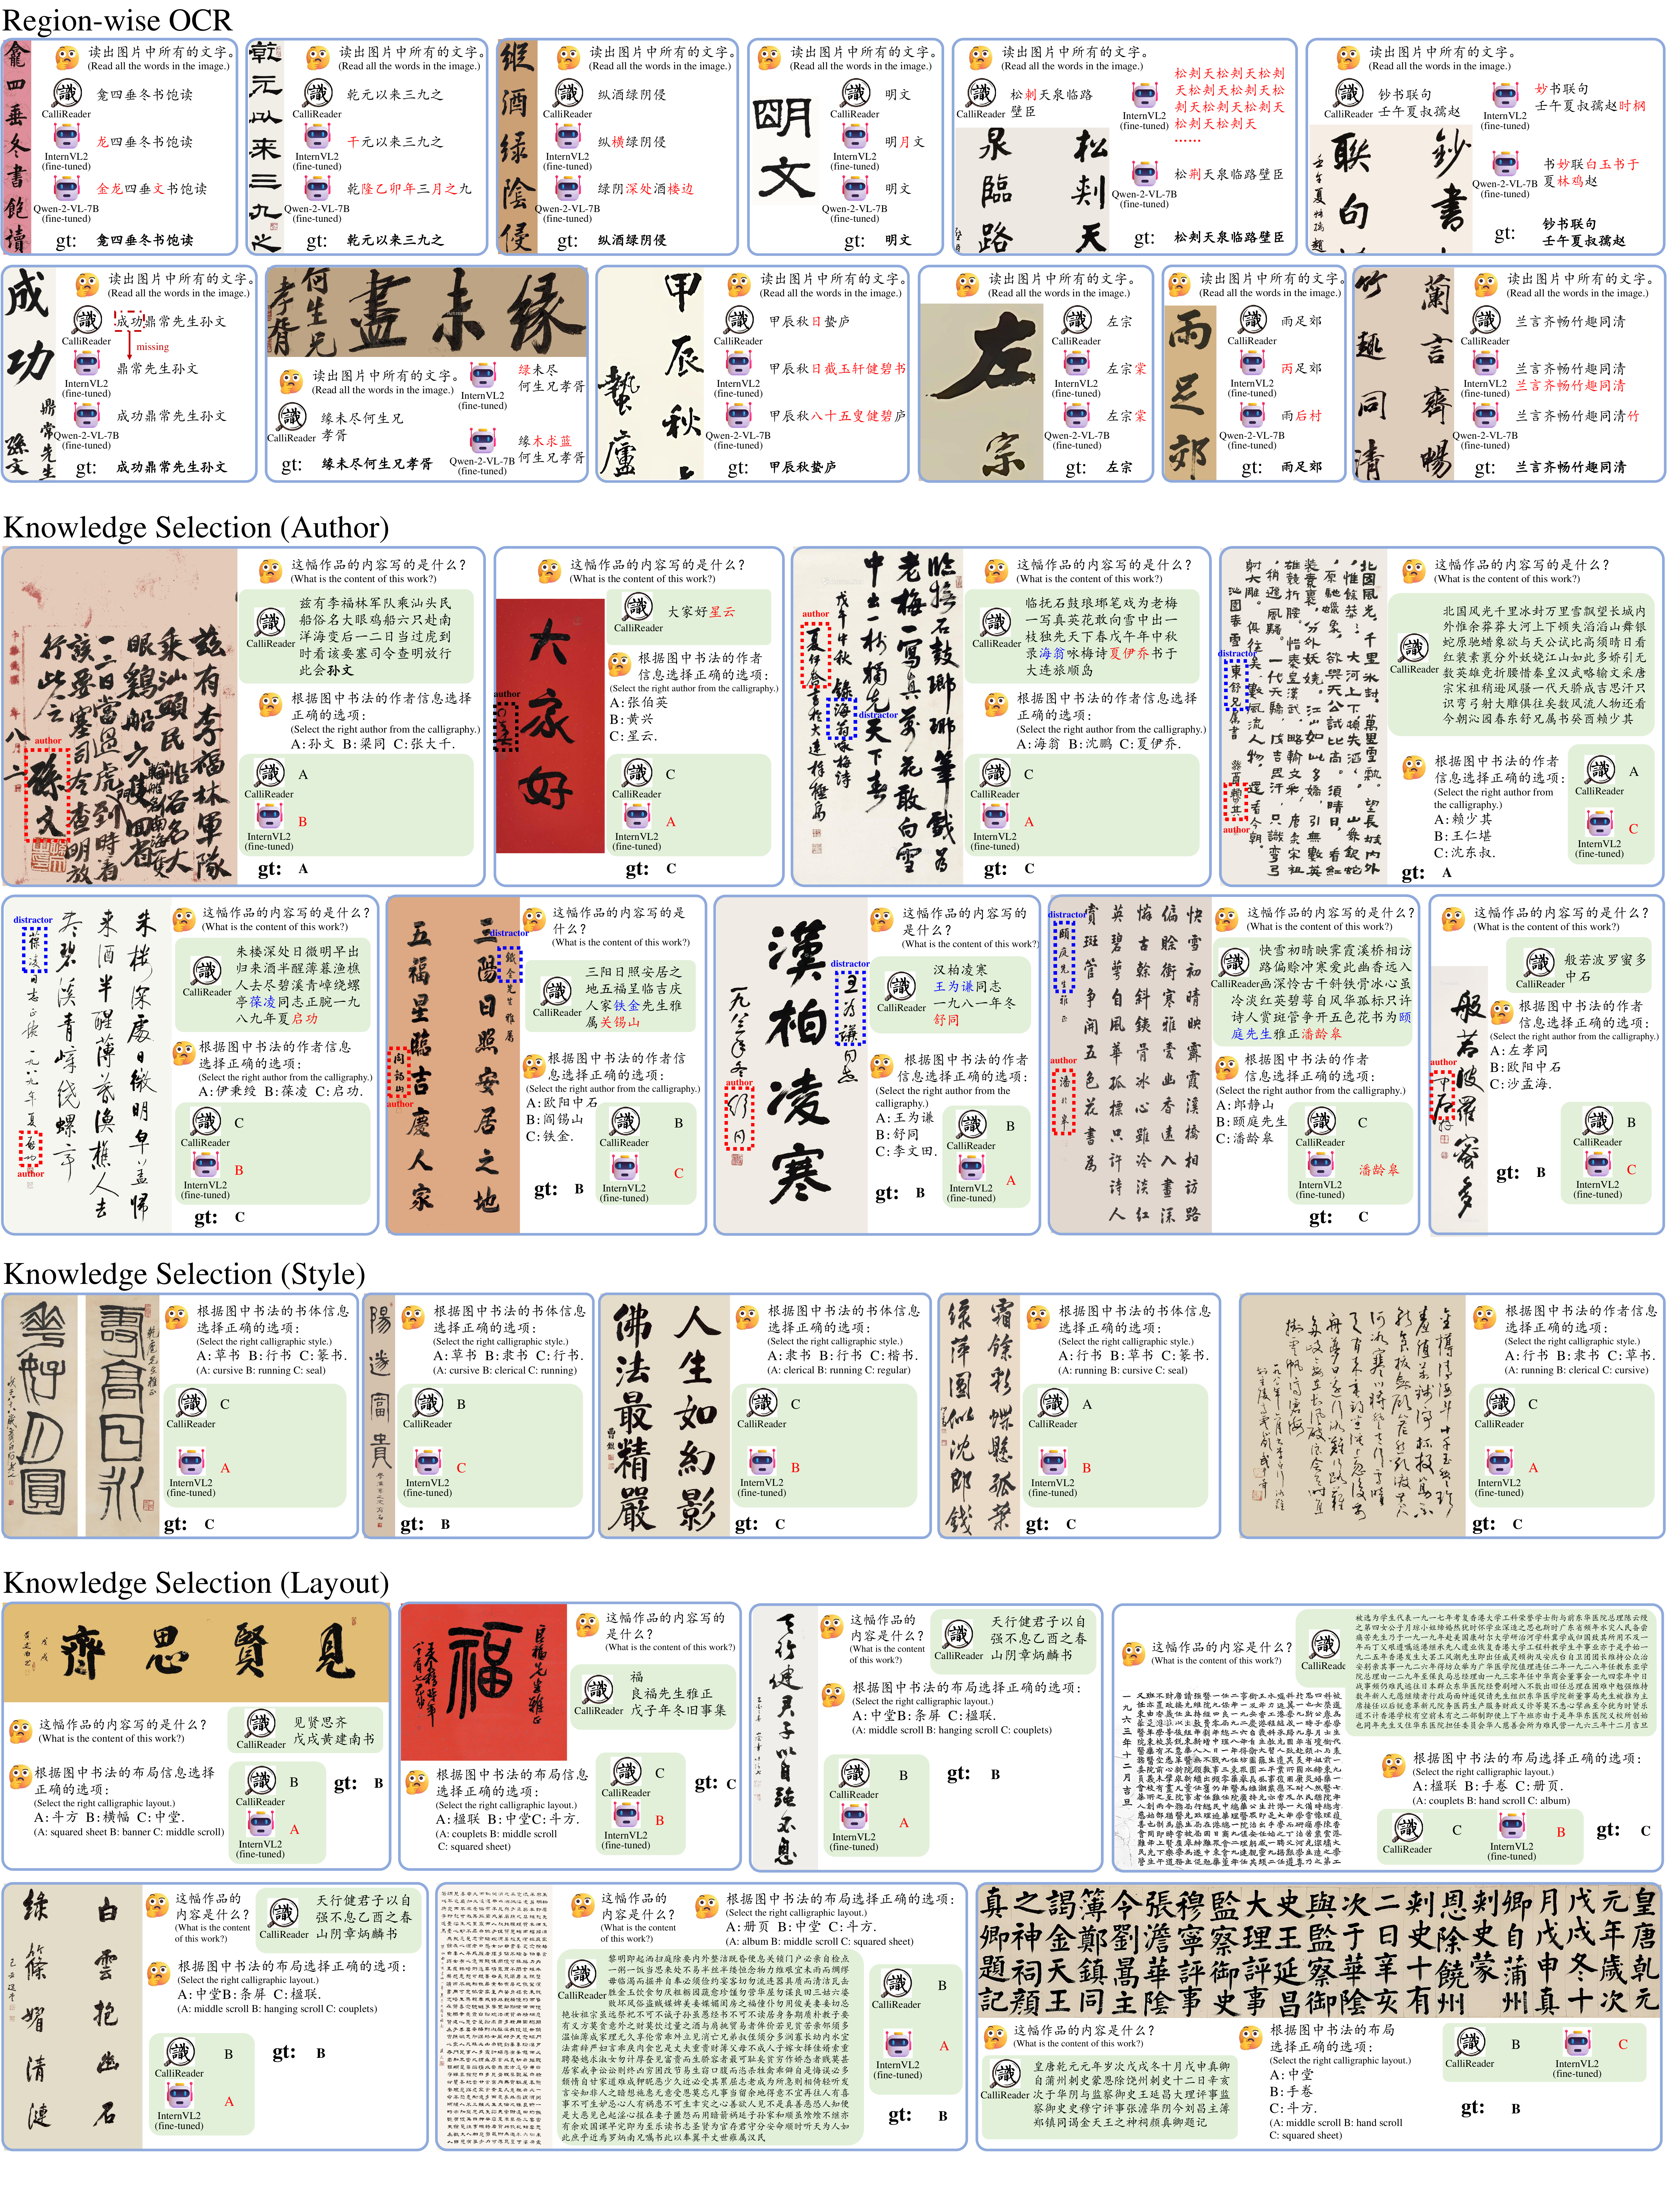}
    \vspace{-8mm}
    \caption{More .}
    \label{fig:supp_styles}
\end{figure*}
