# Supplementary material for: CalliReader: Contextualizing Chinese Calligraphy via an Embedding-Aligned Vision-Language Model
Source: arXiv:2503.06472 source file (2025-03-12)
Supplement: Supplementary file 2 [file X_suppl.tex]

\clearpage
\setcounter{page}{1}
\maketitlesupplementary

    % 修改表格标签
  % 修改图片标签

\section{Potential Questions}

We address potential reader concerns below.
\vspace{-1mm}
\subsection{Slicing is not Patchify}
\vspace{-1mm}
Patchify, introduced in ViT~\cite{dosovitskiy2021an}, divides images into non-overlapping patches for token embedding with positional encoding while slicing segments of high-resolution images into smaller pieces for a fixed-resolution backbone, typically without positional encoding.

Methods such as the sliding-window in Monkey and textMonkey~\cite{li2024monkey,liu2024textmonkey}, overlapping slices in GPT-4V~\cite{xu2024llava-uhd}, and non-overlapping slices in~\cite{liu2024llava1_5, li2024llava-next,xu2024llava-uhd, chen2024far}, often fail to preserve text semantics. Poor segmentation can split tokens with shared semantics, reducing attention scores and accuracy. We propose semantic-preserved slicing to enhance text recognition by maintaining visual character order.
\vspace{-1mm}
\subsection{Training Strategy for \textbf{\textit{CalliReader}}}
\vspace{-1mm}
\textit{CalliReader}, built on InternVL-8B~\cite{chen2024far}, incorporates character-wise slicing and \textit{CalliAlign}. Unlike typical approaches that fine-tune inserted modules with the VLM~\cite{alayrac2022flamingo, li2023blip-2}, we pre-train these modules separately and fine-tune the LLM using e-IT. This strategy is motivated by:

\begin{itemize}
    \item \textbf{Data Abundance.} While page-level calligraphic data is limited, single-character calligraphy datasets are abundant. Thus, pre-training \textit{CalliAlign} ensures effective mapping from character images to pseudo-text embeddings. 
    
    \item \textbf{Resource Efficiency.} Joint training increases parameter load and memory usage due to slicing operations, reducing batch sizes and GPU utilization. Thus we separate pre-training to alleviate these issues.
    
    \item \textbf{Effective Fine-Tuning.} e-IT enhances page-level data with character-level corpora, enabling efficient fine-tuning of the LLM with LoRA, and reducing memory usage compared to traditional image-text pair fine-tuning.
\end{itemize}
\vspace{-1mm}
\subsection{Input Format of \textbf{\textit{CalliAlign}}}
\vspace{-1mm}
\textit{CalliAlign} converts character images into pseudo-text embeddings, reducing computational costs by $98.8\%$, from 256 image tokens to just 3 textual tokens. This facilitates the recognition of long calligraphic scrolls with over 400 characters. An alternative approach is grouping $s$ characters per slice, but this introduces several challenges:

\begin{itemize}
    \item \textbf{Mapping Ambiguity.} Aligning grouped visual images with their textual semantics, i.e., learning many-to-many mappings, becomes difficult due to unclear semantic relationships, especially with varied fonts and backgrounds.
    
    \item \textbf{Redundant Spatial Information.} Grouping characters into a single slice may lead to redundant order patterns, complicating training and making it difficult to recover original spatial arrangements. In contrast, our method encodes bounding box information and inserts it into each pseudo-text embedding, preserving the original positional information~\cite{lu2024bounding}.
    
    \item \textbf{Loss of Characters.} Grouping is similar to the multi-slicing approach in Section 3.1, which suffers from reduced recall due to character omission.
\end{itemize}

\vspace{-2mm}
\section{More on \textbf{\textit{OrderFormer}}}  \vspace{-1.5mm}
\subsection{Architecture}
\vspace{-1.5mm}
This section elaborates on the design and training of \textit{OrderFormer} for interested readers.

Calligraphy layouts are complex but follow certain rules, such as characters arranged in columns read top-to-bottom. To simplify this, we designed an encoder-based \textit{OrderFormer} module to arrange the column order, reducing the sequence length to a maximum of 50. This improves sorting speed and ensures even simple models perform effectively.

\textit{OrderFormer} consists of four encoder layers that compute attention across bounding boxes in the sequence. A three-step pre-processing is applied to formulate the model's input:
\begin{enumerate}
    \item \textbf{Clustering} groups vertical line boxes based on spacing and character box sizes. This separates major content and signature lines.
    \item \textbf{Re-scaling} normalizes box coordinates to the top-left origin and scales by image dimensions $(W, H)$, enhancing numerical stability while preserving layout integrity.  
    \item \textbf{Pre-sorting} standardizes box order to approximate the reading sequence, consolidating varied inputs into consistent formats and improving training efficiency.
\end{enumerate}

After pre-processing, the input becomes a tensor of shape $(B, N, d)$, where $B$ is the batch size, $N=50$ is the maximum sequence length, and $d=4$ represents normalized bounding box coordinates. The model outputs a tensor of shape $(B, N, 1)$, with the final dimension indicating the sorted index for each bounding box.

Specifically, for an input sequence $(B_1, B_2, \dots, B_n)$, the model learns a mapping $f$ such that:\vspace{-3mm}
\begin{equation}
\vspace{-3mm}
f((B_1, B_2, \dots, B_n)) = (id_1, id_2, \dots, id_n),
\end{equation}
where $id_j$ is the position of the $j$-th bounding box in the correct reading order.

\vspace{-1.5mm}
\subsection{Training and Inference}  
\vspace{-1.5mm}
We synthesize 57,627 line-order samples, covering diverse layouts to train \textit{OrderFormer}. By applying $\mathcal{L}_{order}$, which is the Mean Squared Error Loss (MSELoss), the module learns to approximate the correct reading order. We adopt the AdamW optimizer with a learning rate of $\num{2e-4}$, zero weight decay, amsgrad and a CosineAnnealingWarmRestarts scheduler ($T_0=10$, $T_{\text{mult}}=2$, $\eta_{\text{min}}=\num{1e-6}$).  Shorter sequences are padded with $[0, 0, 0, 0]$, and the encoder is trained for 1000 epochs with a batch size of 4, ensuring robust learning of layout-to-order mappings. 

During inference, padding tokens are removed from the output. Each value is mapped to its index in the sorted sequence, maintaining the relative order. For example, given an output $[2.1, 0.3, 1.2, 4.4, 0.1, -0.1]$ and an original sequence of 4 boxes, the result is $[2, 0, 1, 3]$, ignoring padding values. This fault-tolerant approach allows small variations in output without affecting the final order.

\vspace{-3mm}
\section{Dataset Details}
\vspace{-2mm}
\subsection{Annotation Details}
\vspace{-1.5mm}
Our dataset is annotated using the LabelMe~\cite{russell2008labelme} format, with an example of the format shown in Figure \ref{fig:annotation_example}. The key \textit{flag} records information about the authority, layout, and style, while the \textit{shapes} stores individual character labels of calligraphy content, bounding boxes, column numbers, reading order, and other information. Additionally, it stores the image filename, image base64 encoding, and image height and width information. Leveraging this information enables comprehensive evaluations of tasks such as Chinese calligraphy recognition (CCR) and visual question answering (VQA) related to calligraphy works. This dataset not only facilitates these evaluations but also lays a strong foundation for future advancements in the fields of calligraphy recognition and understanding.

\begin{figure}
    \centering
    \includegraphics[width=\linewidth]{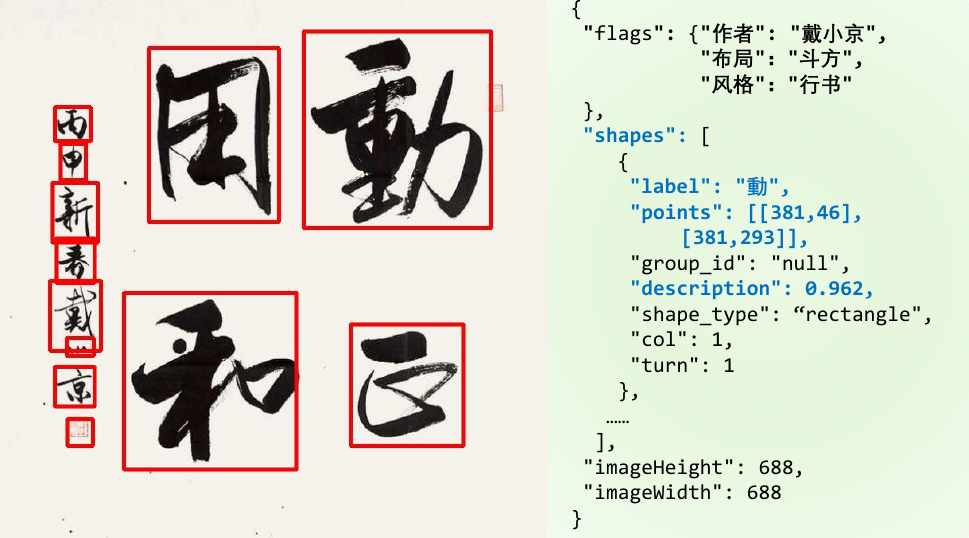}
    \vspace{-5mm}
    \caption{Annotation Format. Left: A piece of Chinese calligraphy. Right: We use the LabelMe format for annotation, recording authority, layout, and style in the \textit{flags} field, while the correct reading order is documented in \textit{row} and \textit{column}.}
    \label{fig:annotation_example}
    \vspace{-3mm}
\end{figure}
\vspace{-1.5mm}
\subsection{Visualization and Comparison}
\vspace{-1.5mm}
\begin{figure*}[t!]
    \centering
    \includegraphics[width=\linewidth]{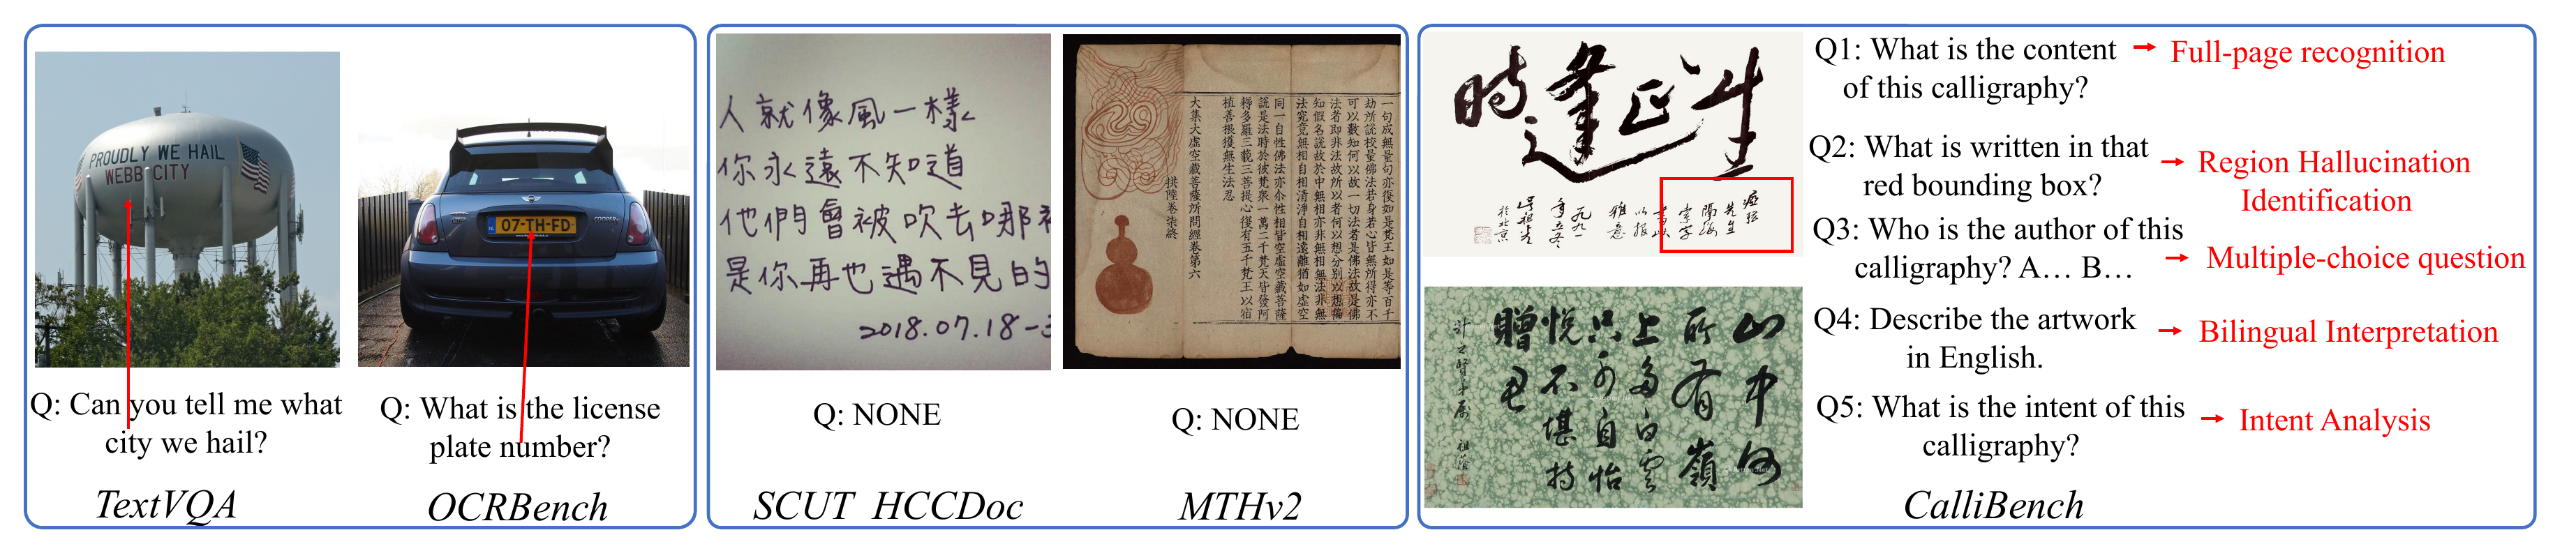}
    \vspace{-7mm}
    \caption{Dataset Visualization and Comparisons. Left 4 columns: Prevalent OCR-oriented datasets are primarily sourced from street signs, product images, exams, and printed ancient books, lacking diversity in writing styles, character size scales, and layout variations. Right column: Our page-level calligraphy dataset features diverse layouts, a wide variety of typefaces, complex backgrounds, and semantic completeness, supporting both OCR tasks and content-oriented Q$\&$A.}
    \label{fig:dataset_comparison}
    \vspace{-4mm}

\end{figure*}

Figure \ref{fig:dataset_comparison} compares our page-level dataset with prominent OCR-related datasets, emphasizing the distinct challenges posed by Chinese calligraphy recognition (CCR) tasks.

OCRBench~\cite{ocrbench2023} and ICDAR2019-ArT~\cite{chng2019icdar2019} primarily feature in-the-wild images where text regions may be rotated or affined. However, these datasets predominantly consist of standard printed typefaces and minimal variation in font size. As such, the primary challenge lies in scene-text detection rather than recognition. Moreover, they are mostly collected from street signs, slogans, and commodity pictures, which lack semantic completeness. This further restricts their applications in complex text-image question answering and deeper semantic exploration. SCUT\_HCCDoc~\cite{zhang2020scut} comprises handwritten text from examination papers and homework. While it provides variability in handwriting styles, its layout is highly structured with fixed reading orders and limited variation in character sizes within individual images, reducing its applicability to the diverse structural and stylistic challenges of CCR. MTHv2~\cite{mthv2}, curated from Chinese historical documents, predominantly features letterpress-printed characters arranged in vertical layouts. The dataset maintains uniform character counts and shapes per line, which fail to reflect the diverse spatial arrangements and typographic variability intrinsic to calligraphy artworks.

In contrast, calligraphy exhibits remarkable diversity in writing styles, spatial arrangements, font sizes, and background patterns. To address these, we curated a dataset of 10,549 page-level calligraphy images from ArtronNet~\cite{artronnet} and CAOD~\cite{CAOD}, featuring modern calligraphy artworks with diverse styles and layouts. Our dataset  is characterized by the following features:
\begin{itemize}
    \item \textbf{Diverse Layouts}. Featuring seven representative Chinese calligraphy layouts, our dataset captures the unique spatial structures and reading orders of various calligraphy forms, offering a wide spectrum of layout complexities.
    \item \textbf{Rich Typeface Variety}. Our dataset covers 5 major calligraphic styles with variants by hundreds of authors. It provides comprehensive stylistic coverage, from highly regular scripts to free-flowing cursive styles.
    \item \textbf{Complex Backgrounds}. Incorporating diverse paper textures and colors, including authentic calligraphy materials, our dataset bridges the gap between synthetic datasets and real-world scenarios, ensuring better generalization to practical applications.
    \item \textbf{Semantic Completeness}. Calligraphic artworks embody a wealth of interpretive potential, encompassing the textual content, author, recipient, location, and creation time. Our annotations meticulously preserve these latent details by annotating the major content with the accompanying inscriptions, enabling knowledge selection and comprehensive comprehension during multi-turn conversations.
\end{itemize}

\vspace{-2mm}
\section{More Experiments}
\vspace{-2mm}
% \subsection{Ablation Losses on \textbf{\textit{CalliAlign}}}
\subsection{Ablation experiments of \textbf{\textit{CalliAlign}} and its loss}
\vspace{-2mm}
In Section 6.5, we evaluated several implementations of the \textit{CalliAlign} framework, comparing the default model to configurations that utilized a two-layer resampler module, global normalization, and additional custom loss functions. Specifically, we designed a custom ratio\_loss $\mathcal{L}_{rat}$ and incorporated CRDLoss $\mathcal{L}_{CRD}$ inspired by contrastive distillation~\cite{tian2019contrastive,khosla2020supervised}. The formulations are shown in Equation~\ref{eq:crd}.
\begin{equation} 
\begin{aligned}
\mathcal{L}_{rat}= w\cdot \frac{1}{N}\sum^{N}_{i=1}(\frac{|y_{i}-\hat{y}_{i}|}{|y_{i}|+eps})+\frac{1}{N}\sum^{N}_{i=1}(y_{i}-\hat{y}_{i})^{2}). \\
\mathcal{L}_{CRD}= \sum_{i \in I} \frac{-1}{|P(i)|} \sum_{p \in P(i)} \log \frac{\exp(z_i \cdot z_p / \tau)}{\sum_{a \in A(i)} \exp(z_i \cdot z_a / \tau)}.
\label{eq:crd}
\end{aligned}
\end{equation}
In $\mathcal{L}_{rat}$, we first define the average deviation ratio as $\frac{1}{N}\sum^{N}_{i=1}(\frac{|y_{i}-\hat{y}_{i}|}{|y_{i}|+eps})$, where $\hat{y}$ is the output of the module and $y$ is the corresponding ground-truth, with $N$ respresenting the number of elements in tensor $y$ and eps representing a small positive value to avoid division by zero. We then define a weight $w=\frac{\tau}{T}\cdot (w_{max}-w_{min}) +w_{min}$, in which $T$ is the total iterations of the training process and $\tau$ is the current iteration number. $w_{min}$ and $w_{max}$ are pre-defined values such that $0 < w_{min} < w_{max} <1$. In the training process, the weight for deviation ratio will linearly increase from $w_{min}$ to $w_{max}$.

$\mathcal{L}_{rat}$ is designed to adapt the model to embedding variance, fitting smaller values more closely, while $\mathcal{L}_{CRD}$ aims to enhance feature distinction via contrastive learning. However, as shown in Figure.~\ref{fig:combined_plot}, $L_2$ loss with layer normalization suffices for fitting, as additional objectives distract training, reflected in early gradient spikes of $\mathcal{L}_{rat}$ (last layer) and $\mathcal{L}_{CRD}$ (first layer). Thus, we ultimately apply the original $L_2$ loss for training \textit{CalliAlign}.
\begin{figure}
    \centering
    \includegraphics[width=\linewidth]{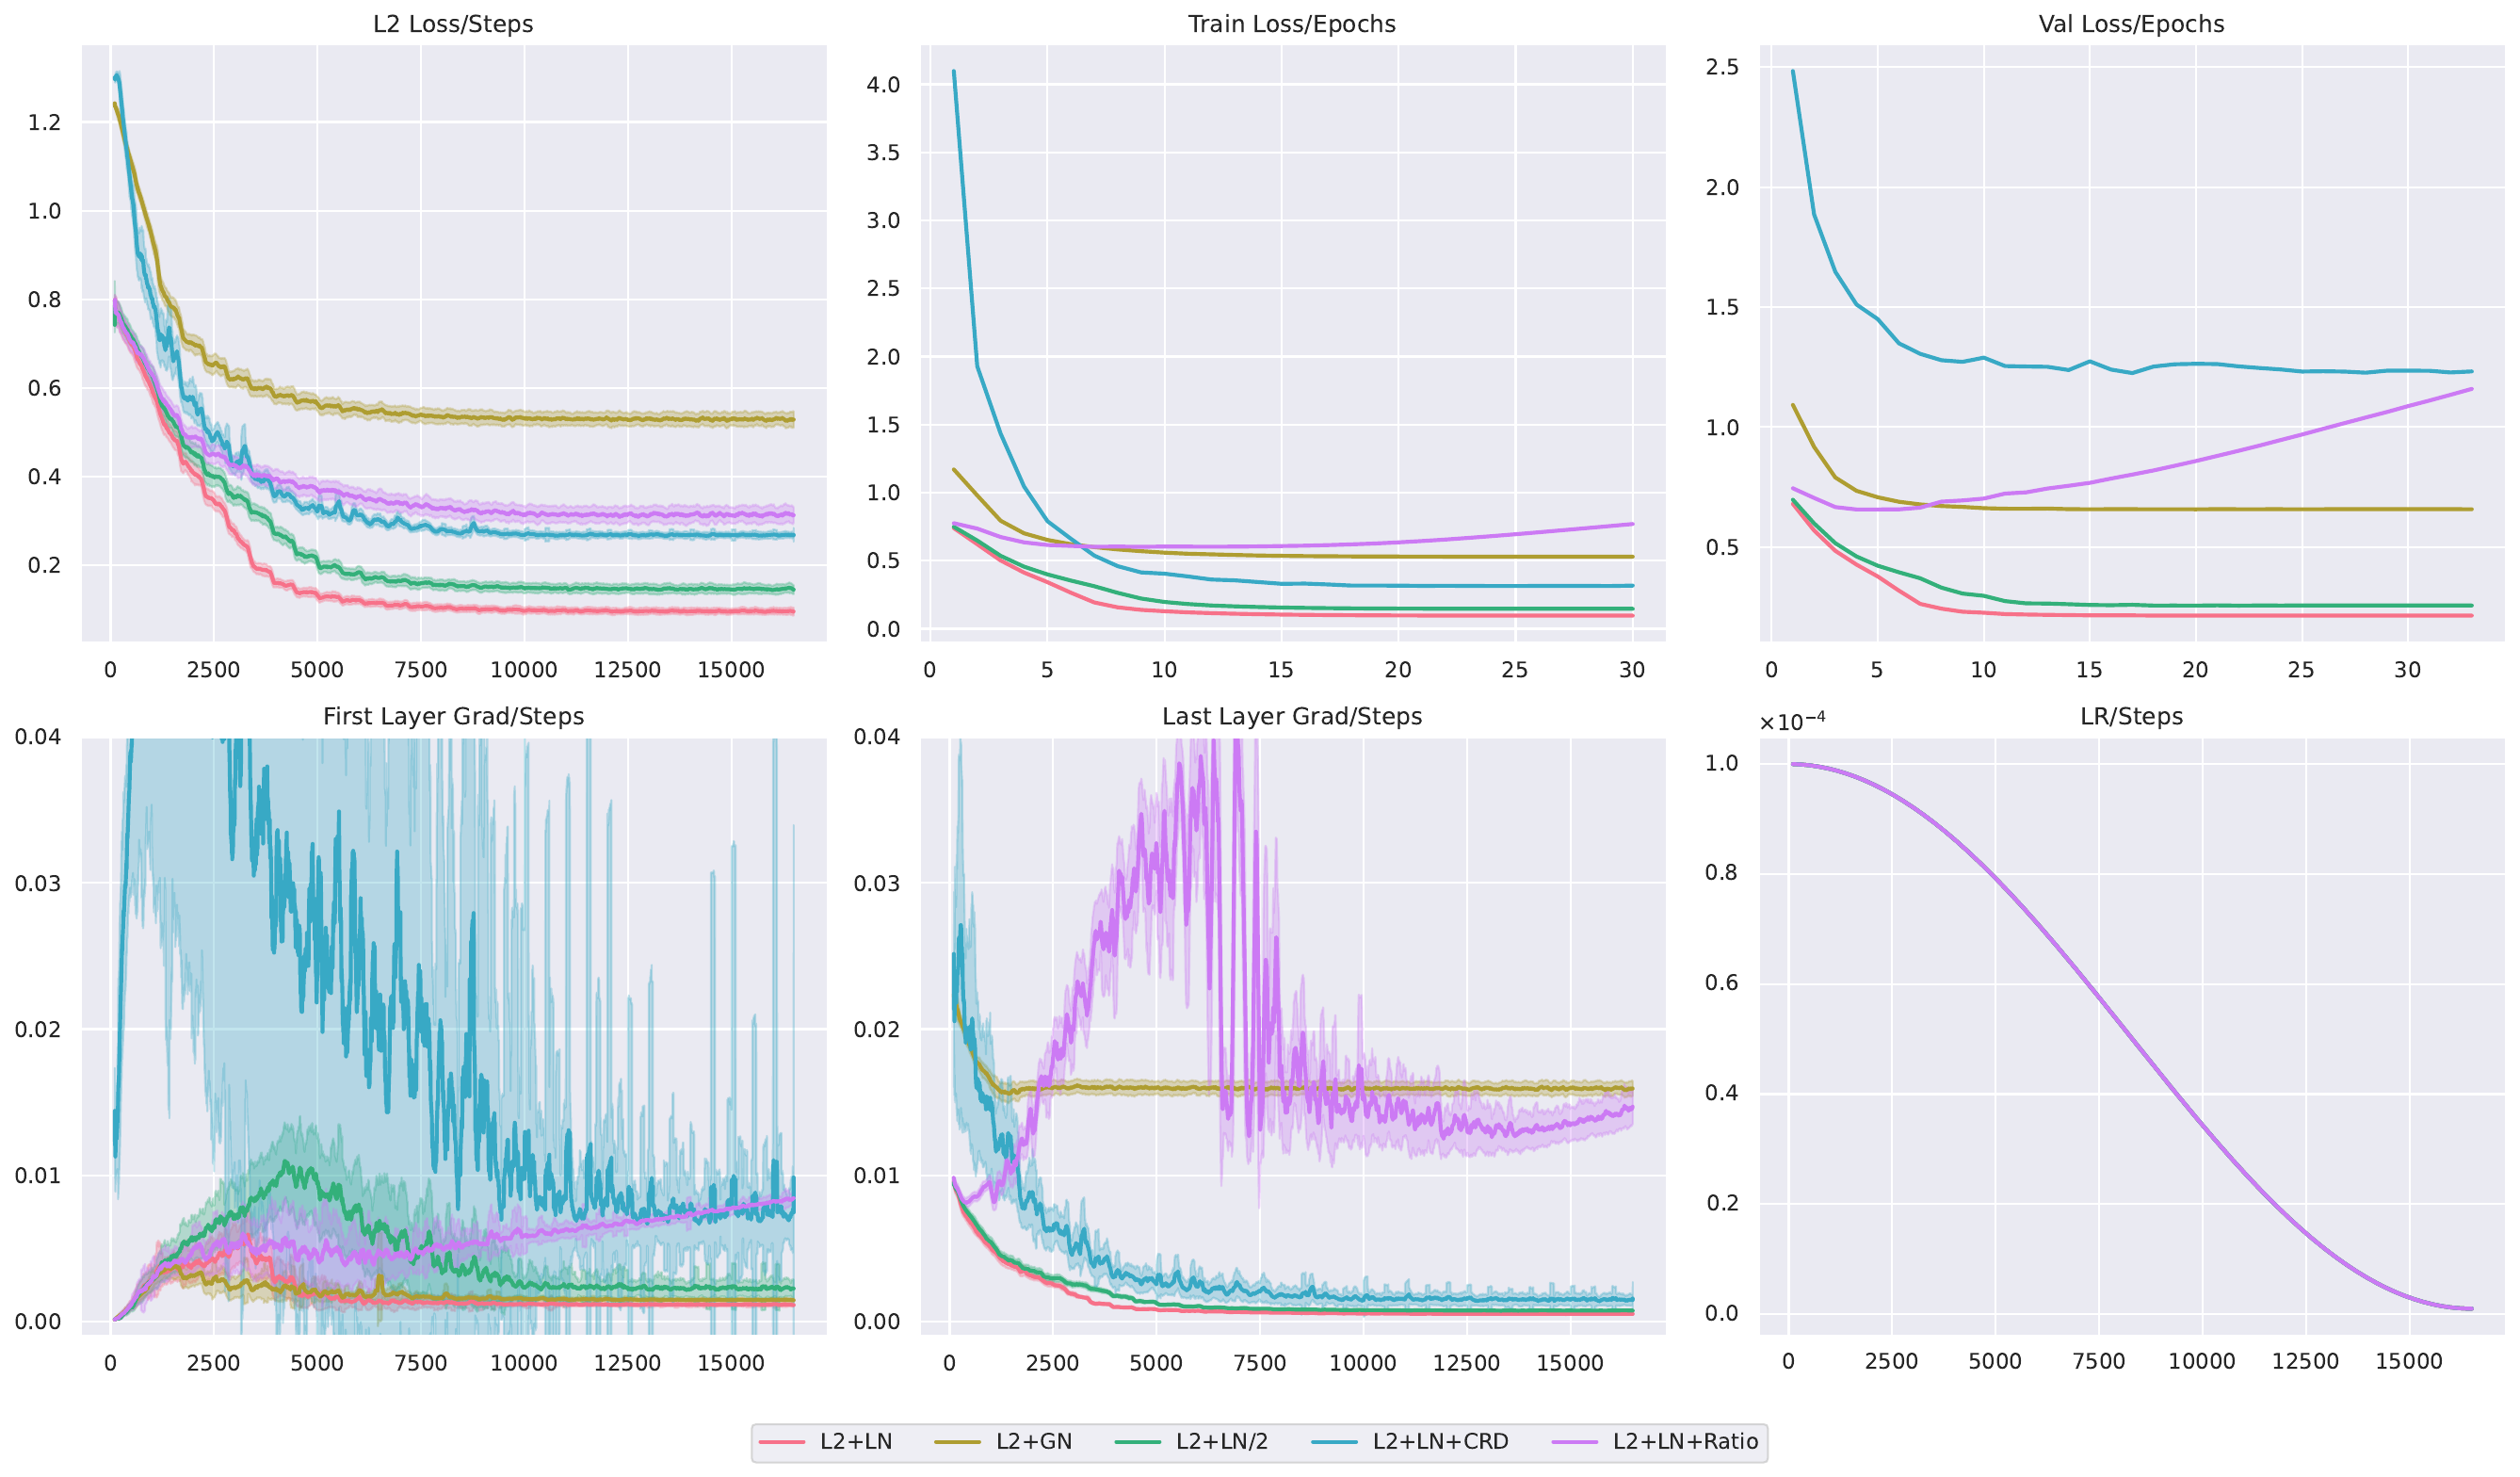}
    \vspace{-5mm}
    \caption{Visualization of the ablative study on \textit{CalliAlign}. Top row: Different settings are compared, showing the training $L_2$ loss (left), total loss (middle), and validation loss (right). It can be observed that \textit{CalliAlign} with 4 blocks and layer normalization, guided solely by $L_2$, achieves the least alignment deviation. Bottom row: Visualization of first layer gradient (left) and last layer gradient (mid) indicates the instability of adding $\mathcal{L}_{CRD}$ and $\mathcal{L}_{rat}$.}
    \label{fig:combined_plot}
    \vspace{-3mm}
\end{figure}

Meanwhile, our experimental proves that even with the size of each slice (character) set to 448×448, \textit{CalliAlign} in the \textit{CalliReader} architecture can even achieve higher efficiency in recognition. Table~\ref{tab:ablation_efficiency} compares the latency (second per page) of \textit{CalliReader} with and without \textit{CalliAlign} on the page-level hard tier. \textit{CalliReader} outperforms due to fewer hallucinations and repetitions. While accuracy and efficiency are often seen as trade-offs, \textit{CalliReader} improves both simultaneously.

\begin{table}[h]
    \centering
    \begin{small}
    \begin{tabular}{lcc}
        \toprule
        CalliReader +e-IT & w/ CalliAlign & w/o CalliAlign\\
        \midrule
        Latency (s/page)$\downarrow$ & \textbf{33.5} & 41.29 \\
        \bottomrule
    \end{tabular}
    \end{small}
    \vspace{-3mm}
    \caption{Quantitative analysis of efficiency on hard tier. \textit{CalliReader} outperforms solely LoRA fine-tuning on page-level inference latency, with less hallucination.}
    \label{tab:ablation_efficiency}
    \vspace{-3mm}
\end{table}

\vspace{-2mm}
\subsection{Character Detection Accuracy}
\vspace{-2mm}
During the training of our character detection model, YOLOv10, we adopt a uniform labeling approach by assigning all bounding boxes the label to \textit{char}. This is made to minimize the classification complexity for the model, allowing it to focus primarily on accurately detecting and localizing the bounding boxes around characters.

Furthermore, we implemented an iterative detection procedure to prevent exceeding the maximum detection number. For each iteration $i$, we detect a set of bounding boxes $\mathbf{B_i}$ and apply mean-filling to the text regions until $\mathbf{B_i} = \emptyset$. Thus, we obtain the final character bounding box set $\mathbf{B} = \bigcup_i \mathbf{B_i}$. This approach enables comprehensive detection of artworks with dense characters, extending \textit{CalliReader}'s compatibility to recognize and interpret lengthy calligraphy pieces and historical documents.

We conducted character detection experiments on our hierarchical full-page OCR dataset and MTHv2~\cite{mthv2} dataset to evaluate our character detection model. The average intersection of union (IoU), precision (P), recall (R), and macro-F1 score (F1) serve as evaluation metrics.

\begin{table}[h]
    \centering
    \begin{small}
    \begin{tabular}{lcccc}
        \toprule
        Datasets & IoU & P & R &F1\\
        \midrule
        Easy & 0.926 & 0.981 & 0.995 & 0.988\\
        Medium & 0.929 & 0.976 & 0.993 & 0.984\\
        Hard & 0.898 & 0.978 & 0.830 & 0.898\\
        MTHv2 & 0.802 & 0.961 & 0.972 & 0.967\\
        \bottomrule
    \end{tabular}
    \end{small}
    \vspace{-3mm}
    \caption{Character detection results on our hierarchical full-page OCR dataset and MTHv2 dataset. Our trained YOLO model shows remarkable character detection ability. The average recall is relatively low on the hard-level full-page OCR data due to cursive writings, diverse layouts, texts of varying lengths, etc. The average IoU on the MTHv2 is slightly lower since it has a large number of small and dense texts. Nevertheless, the overall performance is totally acceptable.}
    \label{tab:YOLO_test}
    \vspace{-3mm}
\end{table}
As shown in Table~\ref{tab:YOLO_test}, our trained YOLO has demonstrated powerful character detection ability. Moreover, it achieves remarkable performance on unseen MTHv2 datasets, proofing the model's adaptability.
\vspace{-1.5mm}

\subsection{Comparison with OCR models}
\vspace{-2mm}

There are many OCR models available that can handle OCR well, but experiments have shown that these models do not perform satisfactory in dealing with the complex scenarios of CCR. We fine-tune PP-OCRv4 and EasyOCR for 40 epochs on our 7k-page dataset and test on full-page OCR hard tier(see Table~\ref{tab:ablation_compare} and Figure~\ref{fig:fuck-reviewers}), which highlights the recognition performance of \textit{CalliReader}, which far exceeds that of other OCR models.

\begin{table}[h]
    \centering
    \begin{small}
    \begin{tabular}{lcc}
        \toprule
        Model & F1$\uparrow$ & NED$\downarrow$\\
        \midrule
        CalliReader+e-IT & \textbf{0.609} & \textbf{0.512}\\
        PP-OCR+ft & 0.293 & 0.937\\
        EasyOCR+ft & 0.061 & 0.985\\
        \bottomrule
    \end{tabular}
    \end{small}
    \vspace{-3mm}
    \caption{Comparison between \textit{Calli-Reader+e-IT} and fine-tuned OCR m-odels on the hard tier. None of the latter can handle CCR tasks.}
    \label{tab:ablation_compare}
    \vspace{-3mm}
\end{table}

\begin{figure}
    \centering
    \includegraphics[width=\linewidth]{CalliDecode Deciphering Chinese Calligraphy Artworks with Vision Language Model/rebuttal_ocr_comp.pdf}
    \vspace{-7mm}
    \caption{Visualization of OCR on the hard tier: \textit{CalliReader} demonstrates the highest accuracy, whereas fine-tuned InternVL2 generates hallucinations, while fine-tuned PP-OCR and Open-OCR fails to produce coherent content.}
    \label{fig:fuck-reviewers}
    \vspace{-1mm}
\end{figure}

We also tested the performance of \textit{CalliReader} as well as fine-tuned InternVL2 and OCR models on some OCR benchmarks including SCUT-HCCDoc, MTHv2, and OCRBench (dataset visualized in Figure \ref{fig:dataset_comparison}). Table \ref{tab:generalization} further demonstrates \textit{CalliReader}'s strong performance across diverse datasets and confirms the effectiveness of e-IT and \textit{CalliAlign}.

\begin{table}[t]
    \vspace{-2mm}
    \centering
    \setlength{\tabcolsep}{2pt} % Reduce space between columns
    \begin{scriptsize}
    \begin{tabular}{l|ccc|ccc|ccc}
        \hline
        \multirow{2}{*}{Model} & \multicolumn{3}{c|}{SCUT-HCCDoc}  & \multicolumn{3}{c|}{MTHV2} & \multicolumn{3}{c}{OCRBench-cn} \\ \cline{2-10} 
         & P↑ & R↑ & F1↑ & P↑ & R↑ & F1↑ & P↑ & R↑ & F1↑  \\ \hline
        CalliReader+e-IT & \textbf{0.766} & \textbf{0.578} & \textbf{0.650}  & 0.791 & \textbf{0.706} & \textbf{0.716} & \textbf{0.788} & \textbf{0.796} & \textbf{0.781} \\
        InternVL2-8B+ft & 0.528 & 0.513 & 0.467& 0.746 & 0.674 &0.669& 0.780 & 0.796 & 0.778   \\
        PP-OCR+ft & 0.662 & 0.392  &  0.478 & \textbf{0.819} & 0.609 & 0.696 & 0.280 & 0.203 & 0.222 \\
        EasyOCR+ft & 0.021 & 0.008  &  0.011 & 0.053 & 0.015 & 0.023  & 0.004 & 0.004 & 0.003 \\
        \bottomrule
    \end{tabular}
    \end{scriptsize}
    \vspace{-3mm}

    \caption{Ablations on handwriting (SCUT-HCCDoc), Document (MTHv2), and General (OCRBench-cn) OCR benchmarks. Evaluations across fine-tuned OCR models and VLMs prove the superiority of our model.}
    \label{tab:generalization}
    \vspace{-5mm}
\end{table}

YOLO, as the tool for detecting character boxes in \textit{CalliReader}, also demonstrates significant advantages compared to OCR models. Its lightweight architecture lowers complexity and ensures fast inference (11.1 FPS in Table~\ref{tab:ablationca1}), crucial for real-time use. Its output supports character-wise slicing, enabling efficient extraction and subsequent processing by the VLM. This allows us to leverage the VLM's visual understanding capabilities while maintaining practical processing speeds.

\begin{table}[h]
    \centering
    \begin{small}
    \begin{tabular}{lcc}
        \toprule
        Model & IoU $\uparrow$ & FPS $\uparrow$\\
        \midrule
        YOLO & \textbf{0.861} & \textbf{11.1}\\
        PP-OCR+ft & 0.774 & 4.1\\
        OpenOCR & 0.390 & 5.4 \\
        EasyOCR+ft & 0.163 & 1.1\\
        \bottomrule
    \end{tabular}
    \end{small}
    \vspace{-3mm}
    \caption{Comparison between YOLO and OCR tools on detecting box. YOLO outperforms all competitors on better accuracy (IoU) and higher speed (FPS).}
    \label{tab:ablationca1}
    \vspace{-3mm}
\end{table}

\section{More Visualizations}
\vspace{-1.5mm}
\begin{figure*}[t!]
    \centering
    \includegraphics[width=\linewidth]{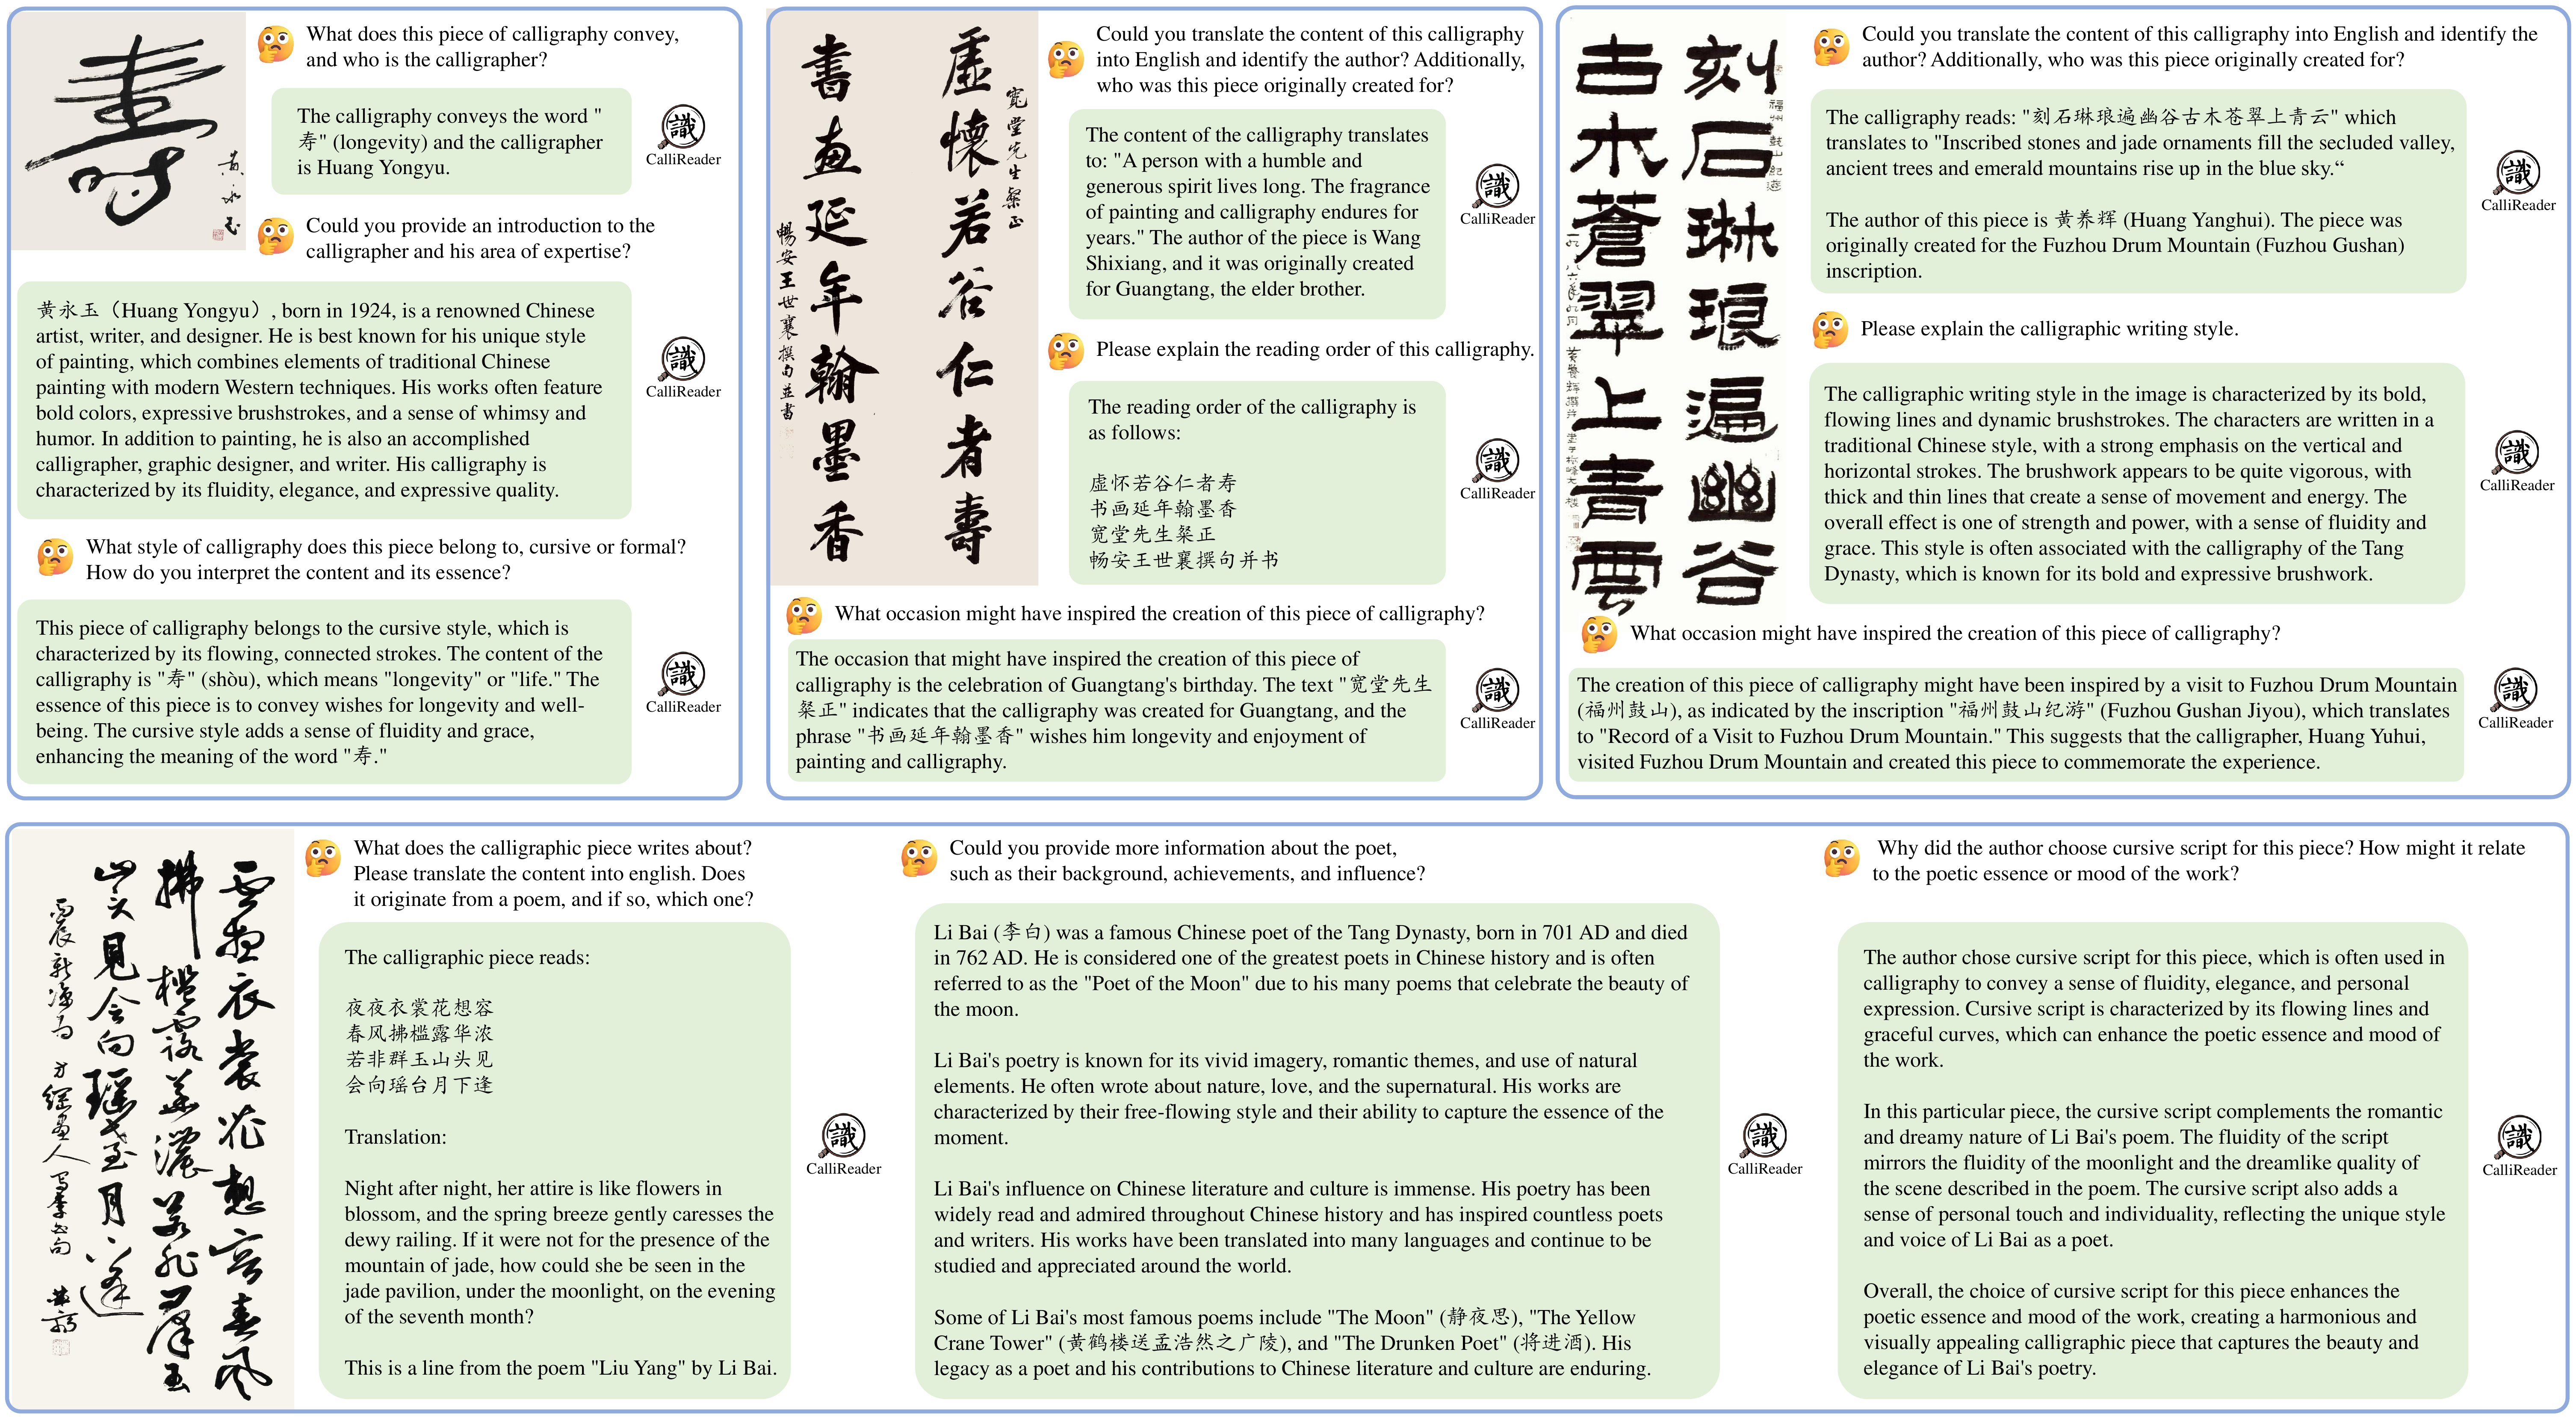}
    \vspace{-8mm}
    \caption{More results of text-centric, multi-turn conversations. \textit{CalliReader} can provide in-depth explanations of calligraphy and understand the complex creative background and aesthetic significance.}
    \label{fig:supp_free}
    \vspace{-3mm}
\end{figure*}

\begin{figure*}[t!]
    \centering
    \includegraphics[width=\linewidth]{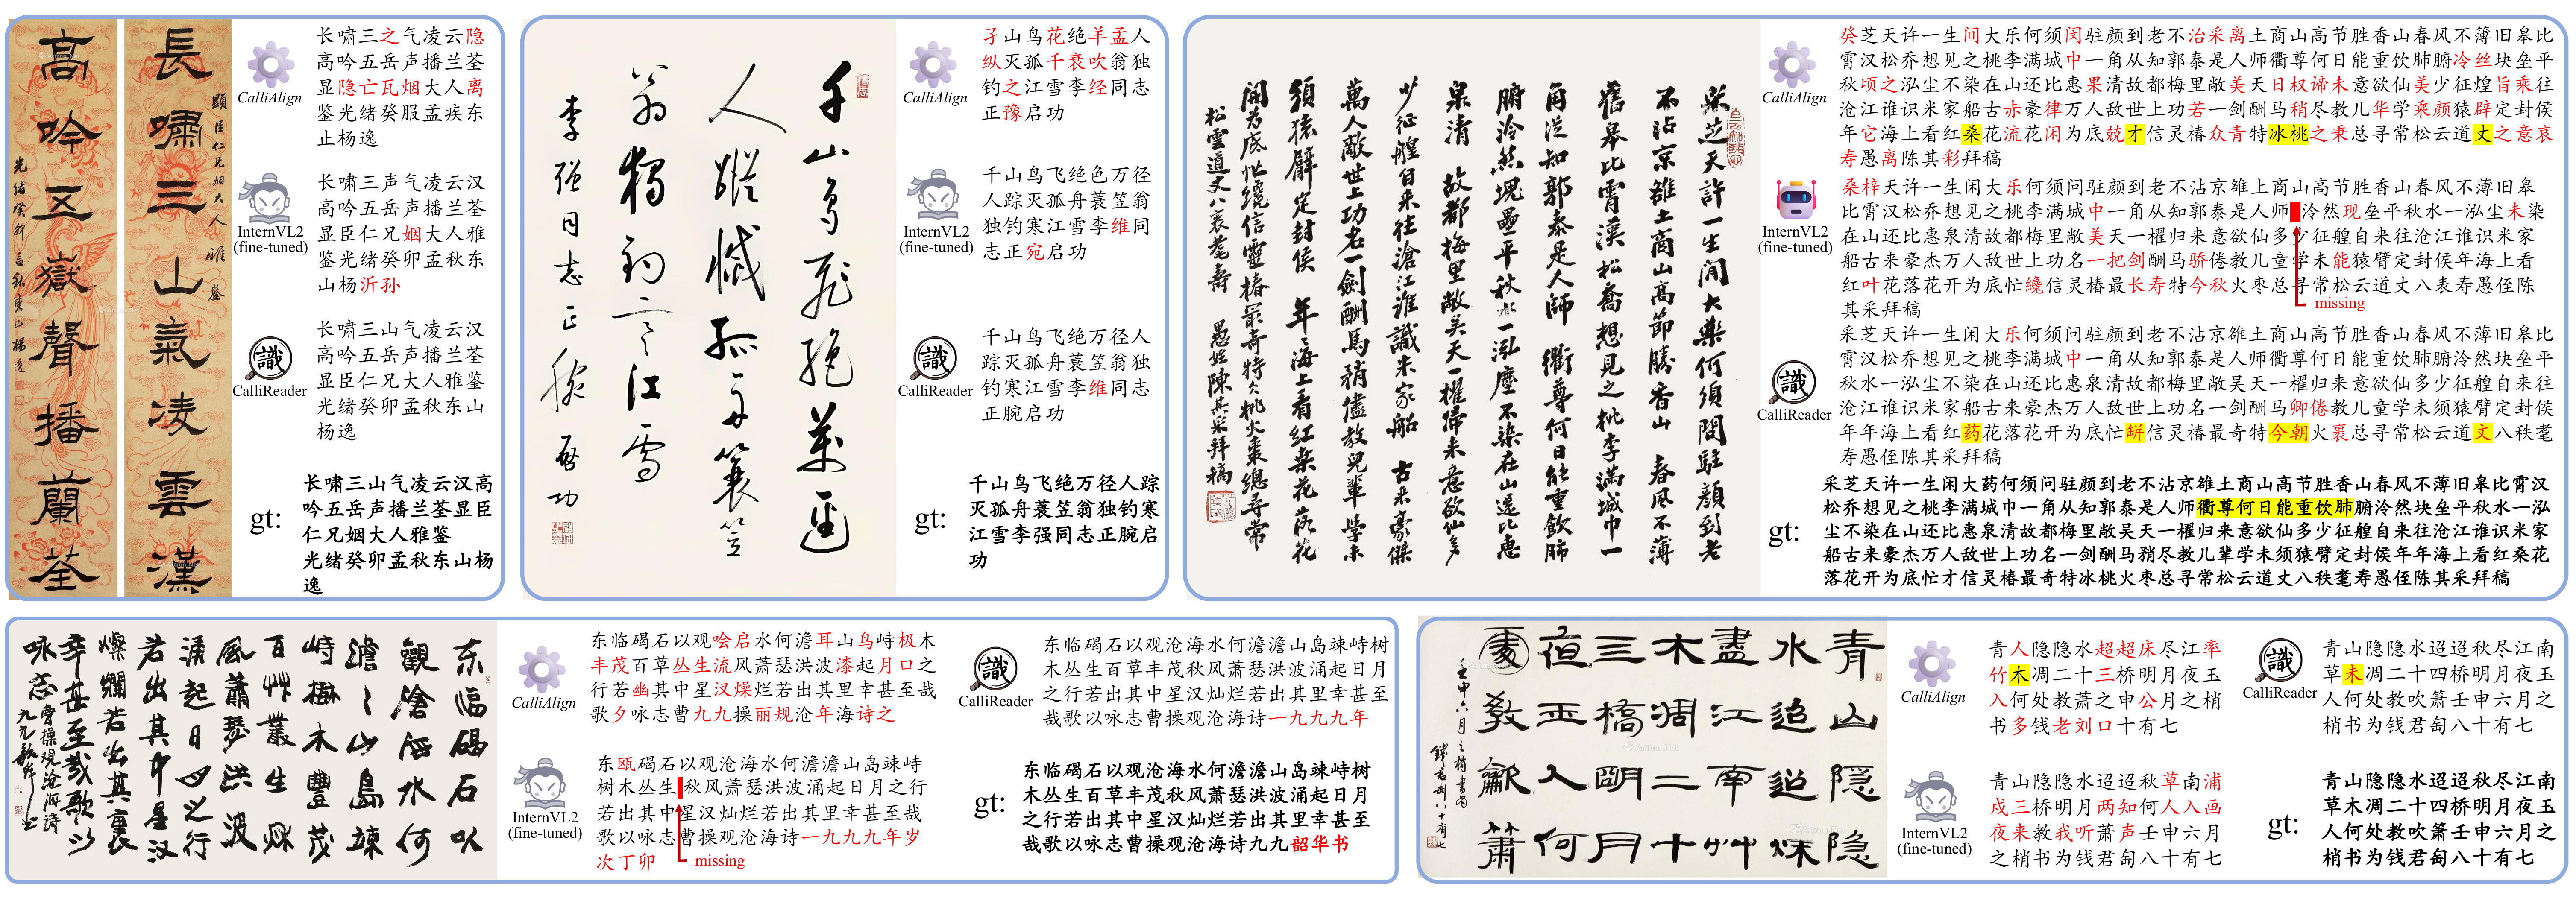}
    \vspace{-8mm}
    \caption{Visualizations of LLM mitigating misalignment. Compared to directly decoding \textit{CalliAlign}, \textit{CalliReader} shows better compatibility with pseudo-text embeddings.}
    \label{fig:supp_comp}
    \vspace{-3mm}
\end{figure*}

\subsection{Text-centric Conversations}
\vspace{-1.5mm}
Unlike traditional OCR methods which focus on detecting text and providing accurate transcriptions, the VLM-based \textit{CalliReader} leverages pre-trained knowledge to engage in flexible, multi-turn, text-centric conversations, addressing diverse user needs. Figure~\ref{fig:supp_free} exemplifies \textit{CalliReader} handling calligraphy in various styles and layouts.

For example, in the dialogue involving a squared-sheet calligraphic piece \textbf{(top-left in Figure~\ref{fig:supp_free})}, \textit{CalliReader} identifies the content, translates it, provides context about the author, and explains the script style. \textbf{In the top-right examples}, the system recognizes the artists and interprets their motivations: the left couplet celebrates Mr. Guangtang’s birthday, while the right commemorates a calligrapher’s visit to Fuzhou's scenic spots. In another example \textbf{(second column)}, \textit{CalliReader} translates the poem into English and introduces the poet, Li Bai, offering historical and cultural context. These examples highlight the versatility of \textit{CalliReader}, transforming complex calligraphic works into accessible interpretations. It bridges language and cultural barriers, allowing anyone interested in calligraphy to explore and appreciate the art.

\begin{figure*}[t!]
    \centering
    \includegraphics[width=\linewidth]{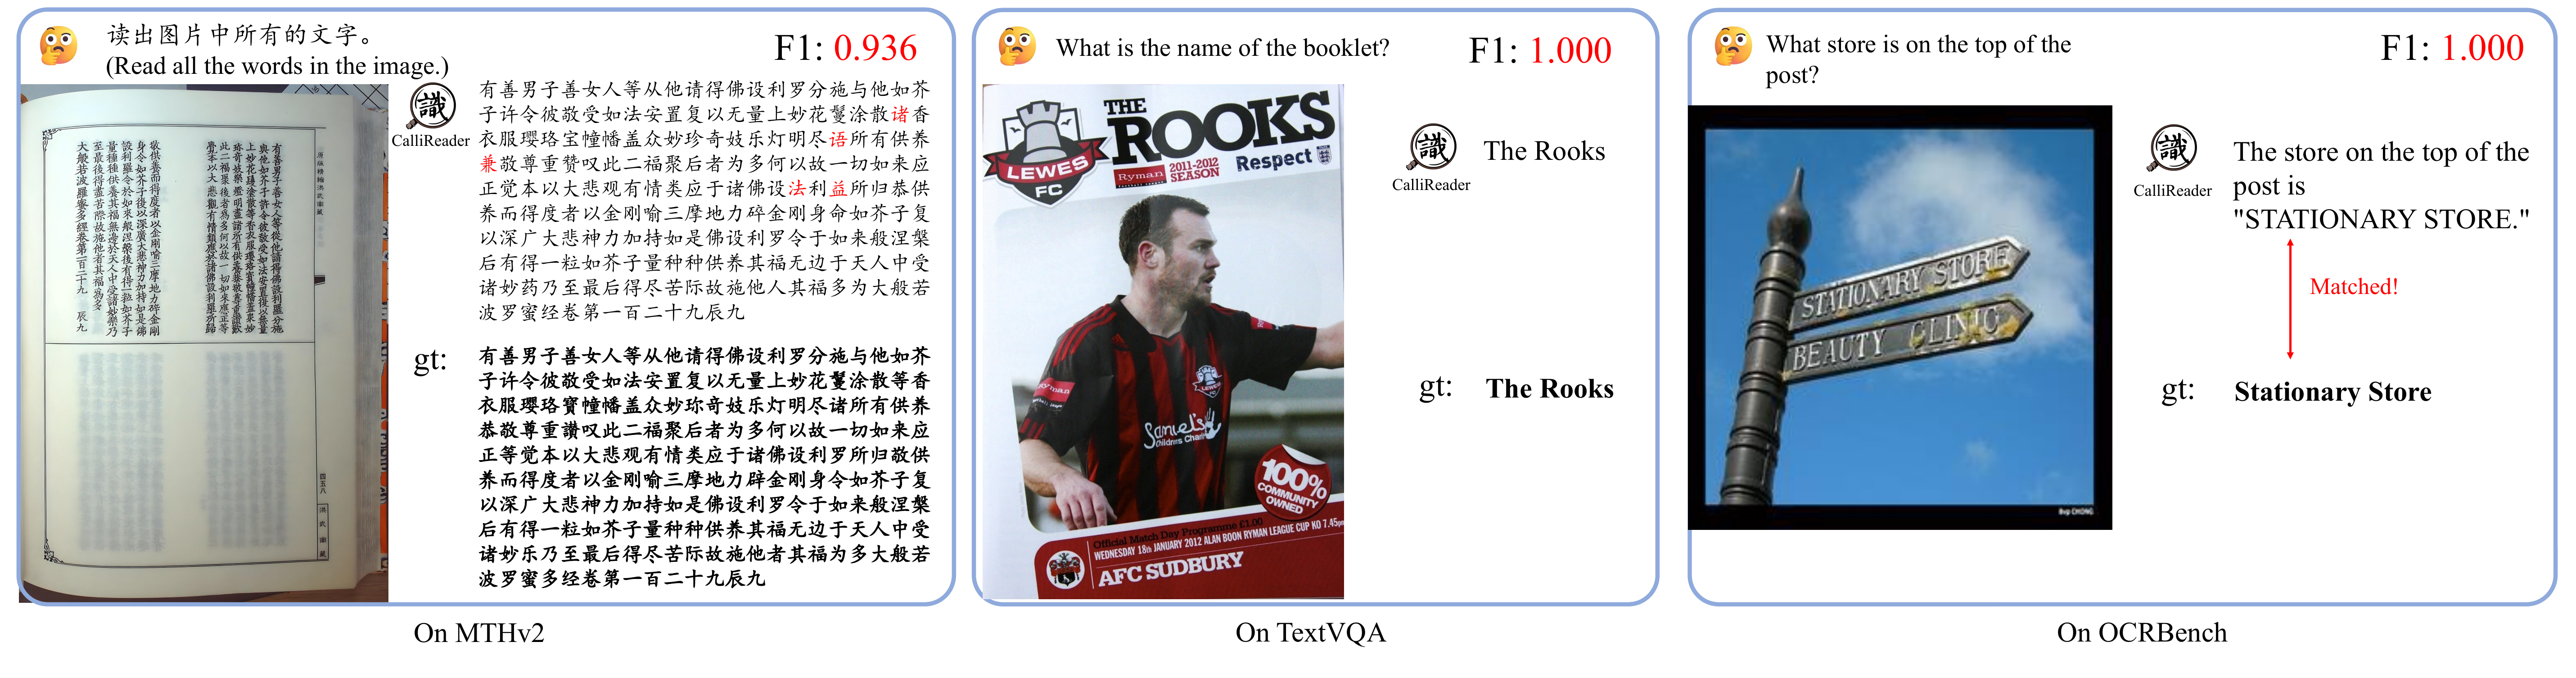}
    \vspace{-8mm}
    \caption{Recognition results on MTHv2. \textit{CalliReader} has the potential to extend to the recognition of ancient texts.}
    \label{fig:supp_mthv2}
\end{figure*}

\begin{figure*}[t!]
    \centering
    \includegraphics[width=0.975\linewidth]{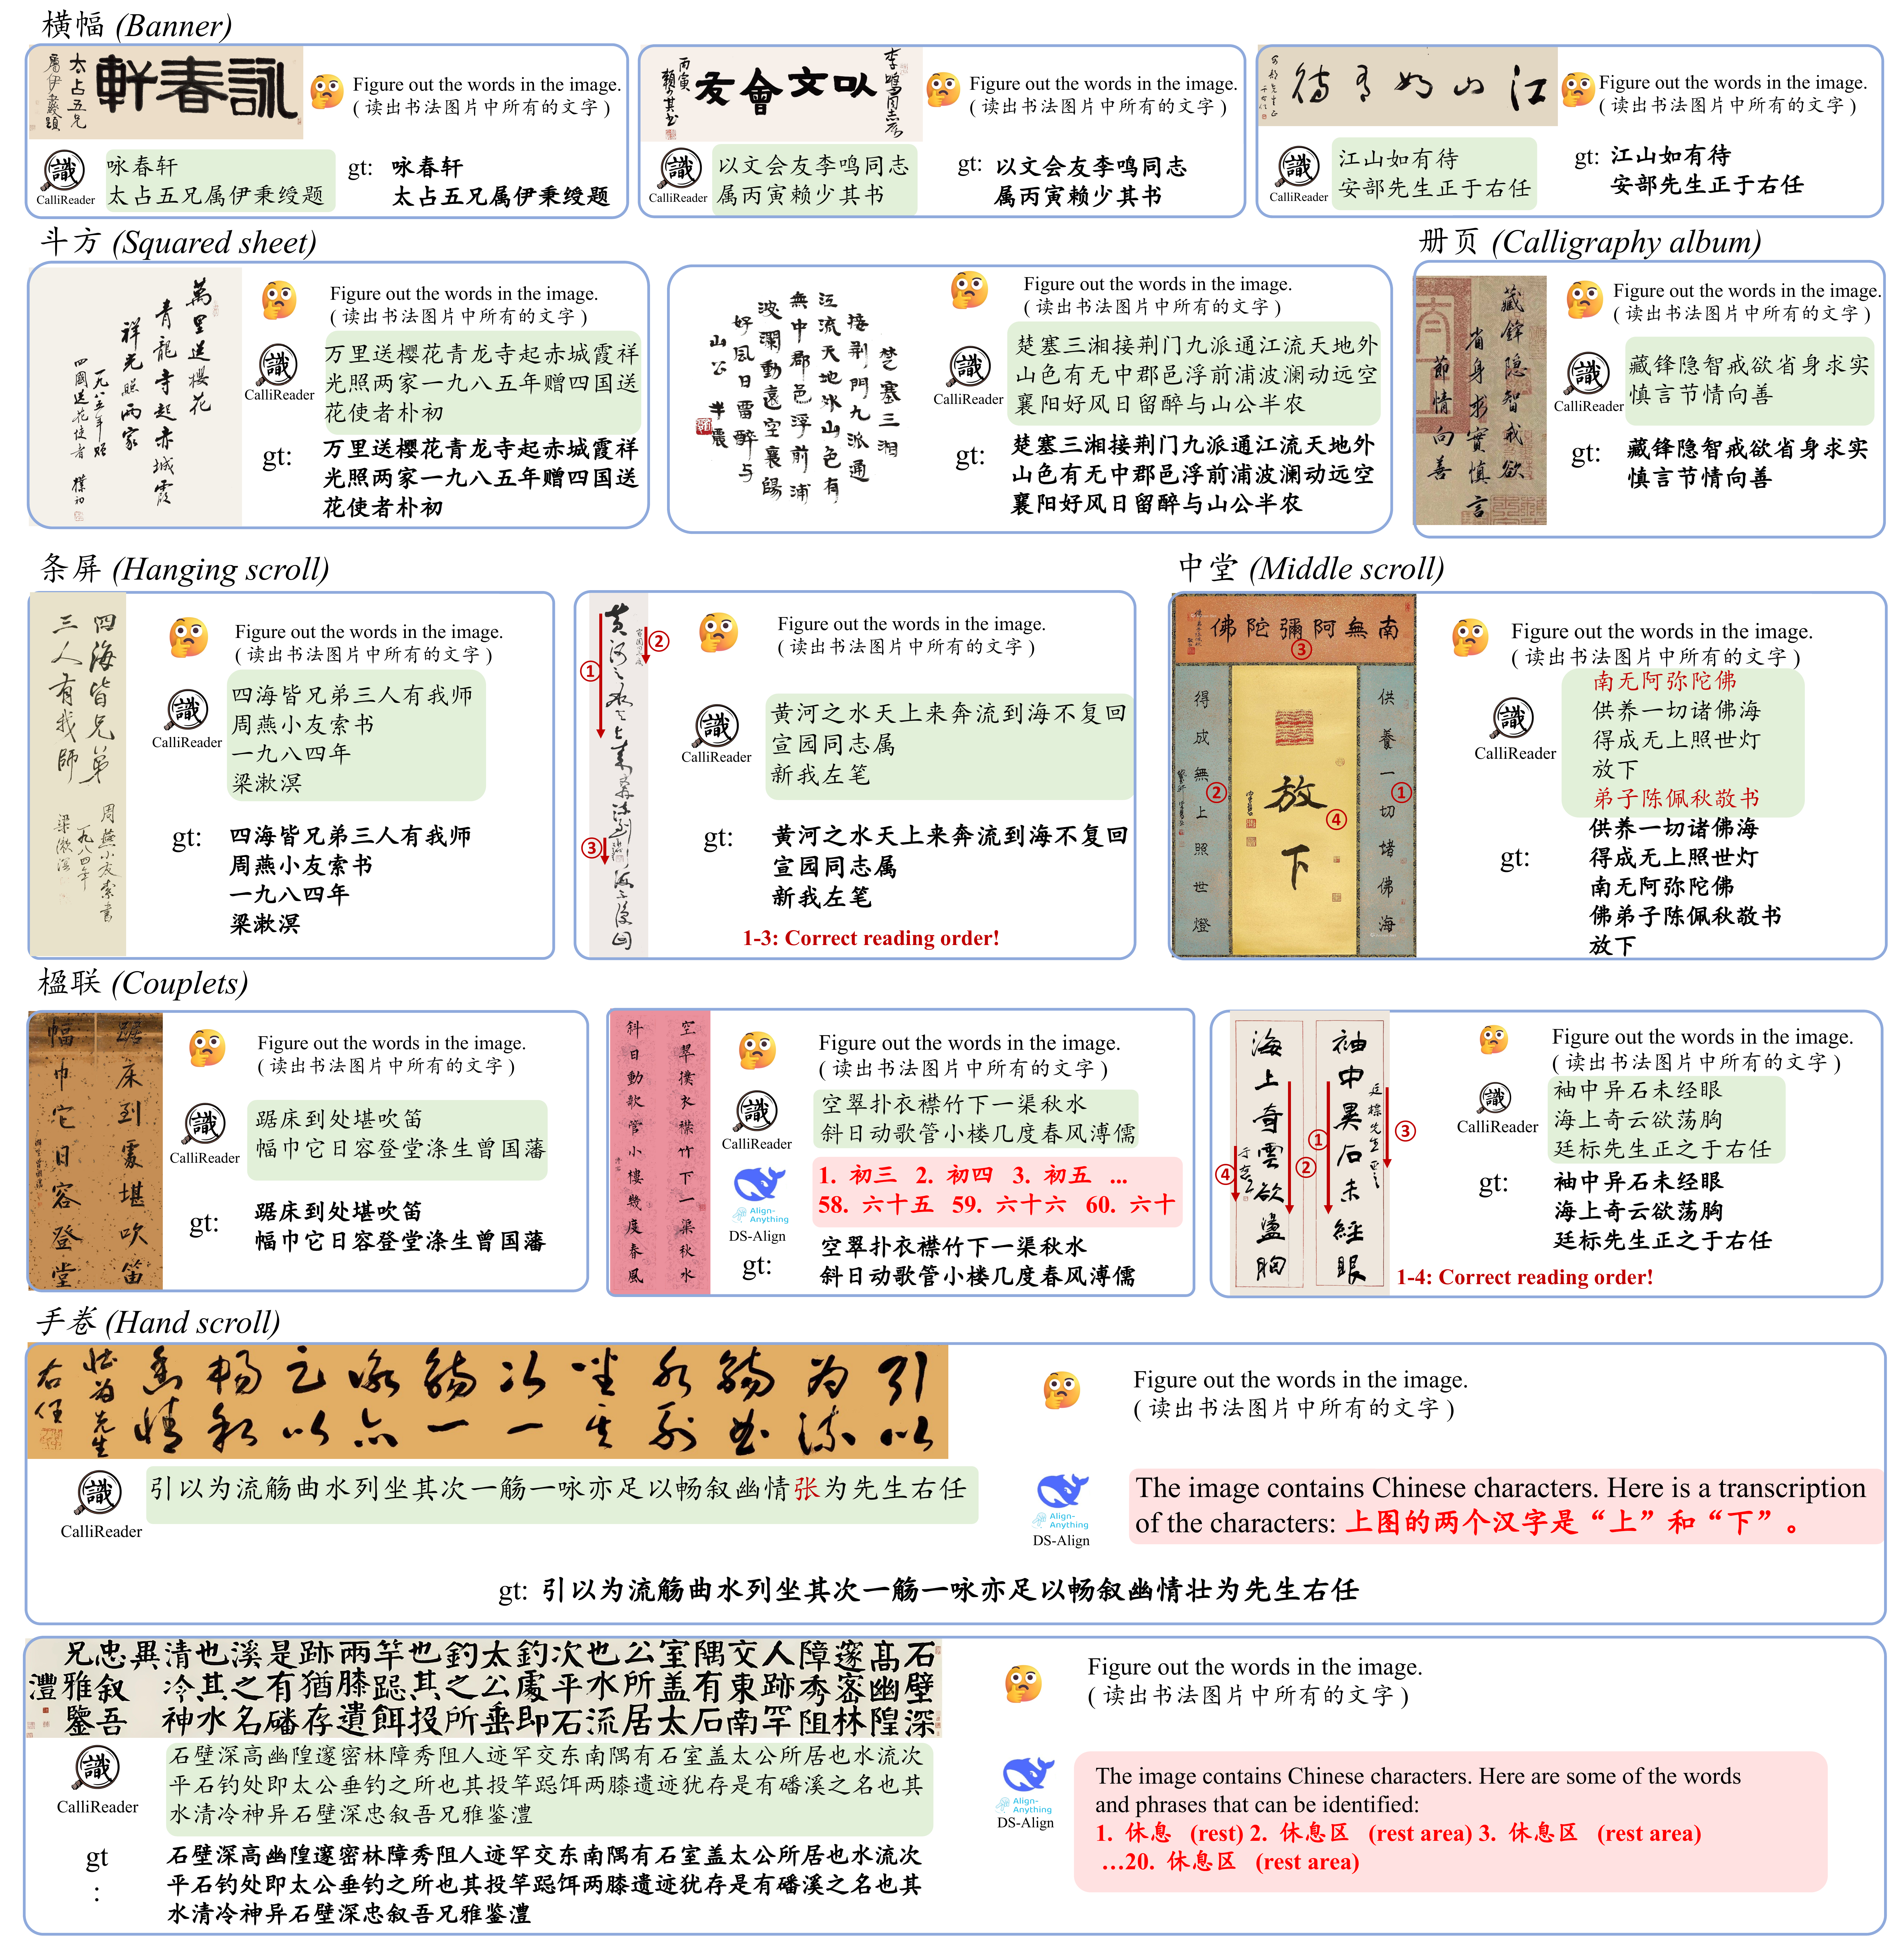}
    \vspace{-4mm}
    \caption{More full-page OCR results on diverse styles and layouts.}
    \label{fig:supp_layouts}
\end{figure*}

\begin{figure*}[t!]
    \centering
    \includegraphics[width=0.98\linewidth]{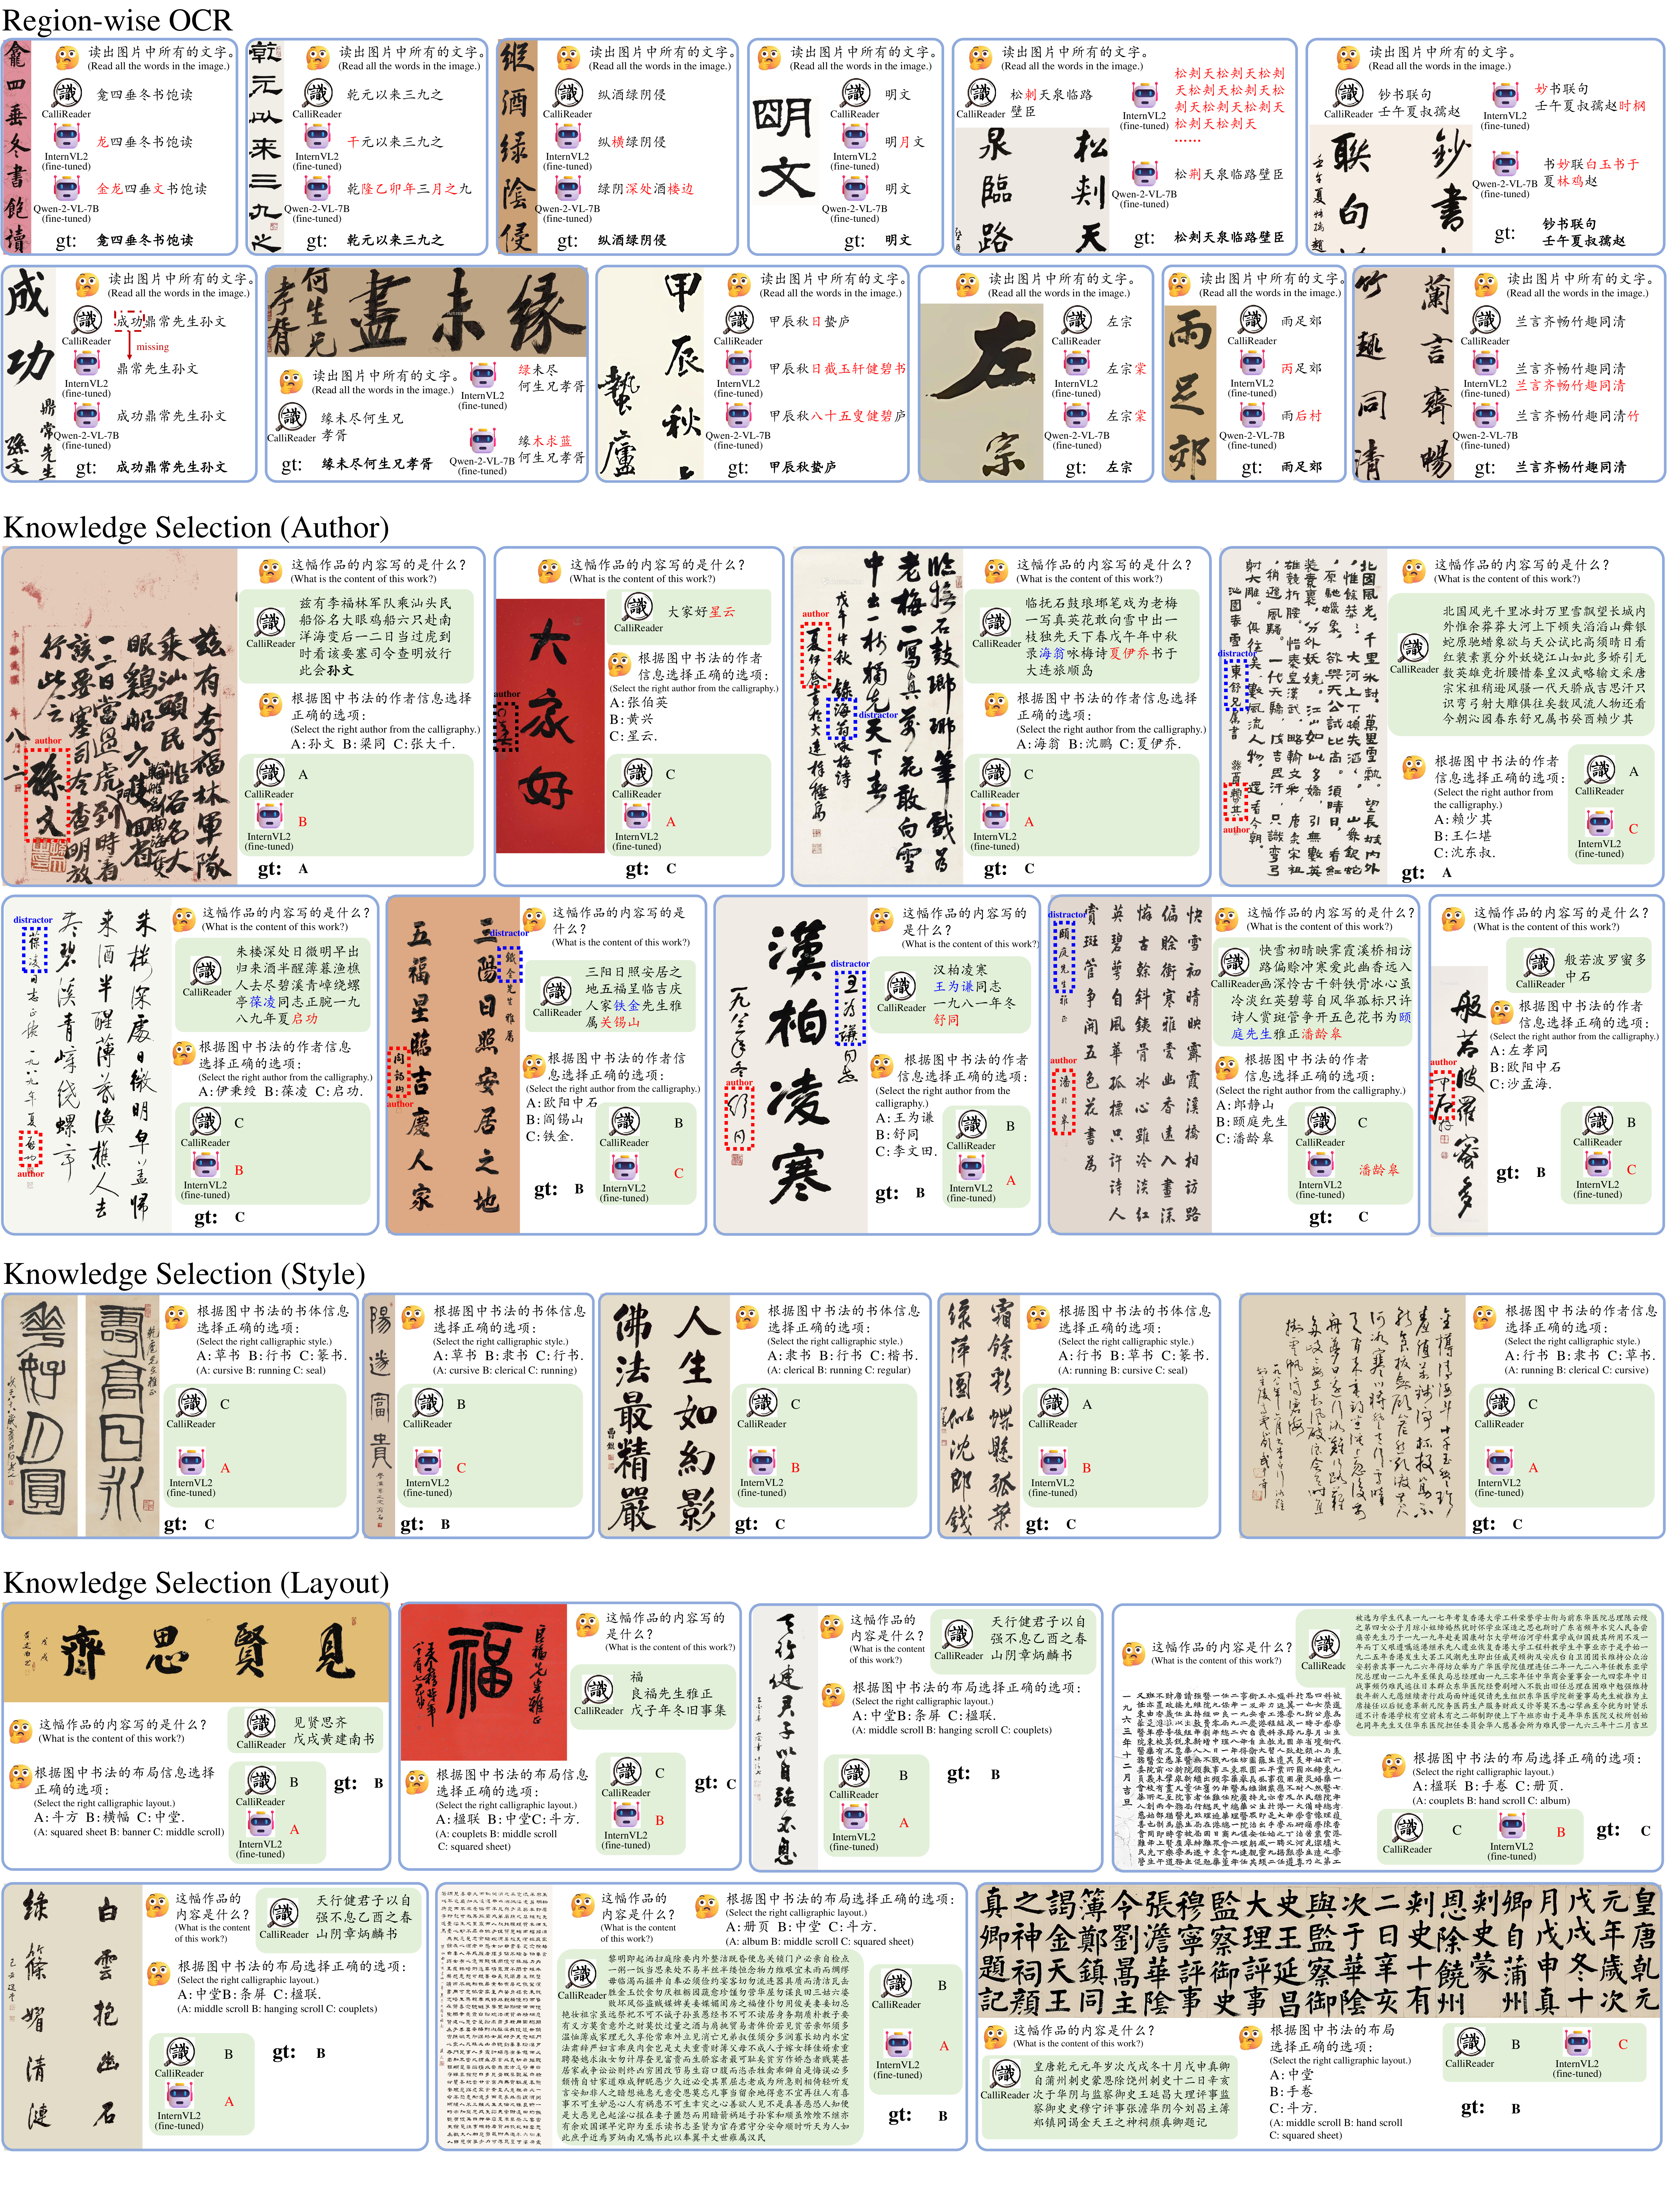}
    \vspace{-9mm}
    \caption{More results on region-wise OCR and knowledge selection.}
    \label{fig:supp_selection}
\end{figure*}
\vspace{-1.5mm}
\subsection{LLM Mitigates Misalignment}
\vspace{-1.5mm}
To evaluate how well fine-tuned \textit{CalliReader} works with pseudo-text embeddings, we conducted a targeted experiment. For calligraphic images, we calculated the cosine similarity $\mathcal{C}$ between each pseudo-text embedding from \textit{CalliAlign} and the original embedding table, identifying the nearest neighbor ID as the corresponding token for decoding. This provides a preliminary performance estimate for using \textit{CalliAlign}. We also compared these results with \textit{CalliReader}'s direct outputs.

As illustrated in Figure~\ref{fig:supp_comp}, the direct decoding of \textit{CalliAlign}, due to its character-wise slicing approach, successfully preserves the correct reading order. However, many characters exhibit ambiguous alignments with low $\mathcal{C}$ values, leading to decoding errors. In contrast, \textit{CalliReader}, boosted by its e-IT fine-tuned LLM, demonstrates enhanced performance. The outputs are semantically coherent and less of errors, leveraging the inherent capabilities of the LLM to refine and correct the pseudo-text embeddings.
\vspace{-1.5mm}
\subsection{Test on MTHv2}
\vspace{-1.5mm}
To further evaluate the generalizability of our approach, we conducted experiments on the test set of the historical document dataset MTHv2~\cite{mthv2}. This dataset comprises Buddhist scriptures and printed book pages, distinguished by their high word density and small font sizes, which introduce significant challenges for text recognition. As illustrated in Figure~\ref{fig:supp_mthv2}, \textit{CalliReader} demonstrates the capability to decipher extensive, contextually rich historical documents. Although promising results are observed, targeted fine-tuning on MTHv2 is expected to further enhance performance.
\vspace{-1mm}
\subsection{More CalliBench Results}
\vspace{-1mm}
\subsubsection{Full-page OCR on Diverse Layouts}
\vspace{-1mm}
Figure~\ref{fig:supp_layouts} showcases the full-page OCR capabilities of \textit{CalliReader} across calligraphic styles and layouts. Our collected page-level dataset encompasses seven primary layout types: banners, squared sheets, calligraphy albums, hanging scrolls, middle scrolls, couplets, and hand scrolls. These layouts feature diverse image aspect ratios, a wide range of calligraphic styles (from seal script to cursive writing), and complex backgrounds with varying colors and patterns.

For example, banners present unique challenges due to their differing writing orientations, such as left-to-right (\textbf{third column in Figure~\ref{fig:supp_layouts}}) and right-to-left (\textbf{second column in Figure~\ref{fig:supp_layouts}}). This variability often renders rule-based methods for detecting reading orders ineffective. However, \textit{CalliReader} leverages the semantic understanding capabilities of VLMs to autonomously determine the correct reading direction, accurately restoring the intended textual content.

Additionally, \textit{CalliReader} demonstrates robustness in handling other challenges, such as intricate backgrounds (e.g., calligraphy albums, \textbf{column 1}), small text (also calligraphy albums, \textbf{column 1}), and maintaining the correct reading sequence for primary content and inscriptions (e.g., couplets, \textbf{column 3}). Furthermore, it exhibits strong recognition performance for cursive writings, as evidenced by comparisons with ground truth, showcasing its adaptability to diverse and demanding calligraphic scenarios.
\vspace{-2mm}
\subsubsection{Region-wise and Knowledge-Selection}
\vspace{-2mm}
Figure~\ref{fig:supp_selection} presents additional visual results showcasing region-wise OCR and knowledge-based content selection. VLMs fine-tuned with image-text pairs often exhibit significant hallucination effects when handling incomplete text, frequently producing irrelevant phrases or repeating content. This aligns with our hypothesis that VLMs rely heavily on memorization and guesswork when performing OCR tasks.

In contrast, the e-IT approach unifies all inputs into a shared embedding space, effectively enabling the model to utilize pseudo-text embeddings during fine-tuning. This improves recognition accuracy and mitigates hallucination effects in complex Chinese calligraphy recognition tasks.

The character-wise slicing strategy further enhances CCR at varying scales, allowing \textit{CalliReader} to accurately recognize small inscription details in calligraphy artworks, such as the signatures and annotations. Performance improvements in authority can be attributed to the inclusion of pseudo-text embeddings, while enhancements in style and layout recognition are likely derived from the integration of layout-specific cues in the calligraphy content. This enables the model to draw upon prior knowledge to provide a deeper understanding of the material.
