# Supplementary material for: CalliReader: Contextualizing Chinese Calligraphy via an Embedding-Aligned Vision-Language Model
Source: arXiv:2503.06472 source file (2025-03-12)
Supplement: Supplementary file 3 [file new_suppl.tex]

\clearpage
\setcounter{page}{1}
\setcounter{section}{0}
\setcounter{figure}{0}
\setcounter{table}{0}
\maketitlesupplementary

    % 修改表格标签
  % 修改图片标签

\section{Overview}
\vspace{-1mm}
Tables 2, 3, 4, and 7 demonstrate that \textit{CalliReader} outperforms existing VLMs and reasoning models in Chinese Calligraphy Contextualization (CC$^2$). This supplementary material provides additional quantitative and qualitative results, details on modules and datasets, and key findings on \textit{CalliAlign}, highlighting the substantial advantages introduced by our method.

The outline is structured as follows:  
\begin{itemize}  
    \item $[$\cref{us}$]$ describes our user study, demonstrating the difficulty of CC$^2$.
    \item $[$\cref{mqc}$]$ evaluates \textit{CalliReader} against conventional, \textbf{fine-tuned} OCR tools.  
    \item $[$\cref{dim}$]$ explains key modules: YOLO, OrderFormer, and \textit{CalliAlign}.  
    \item $[$\cref{align}$]$ visualizes \textit{CalliReader} mitigating \textit{CalliAlign}'s errors, proving the necessity of integrating both plug-ins and e-IT.
    \item $[$\cref{dd}$]$ details the dataset, CalliBench, and the prompting for LLM-as-a-judge in contextual VQA. 
    \item $[$\cref{mv}$]$ presents additional visualizations on CalliBench and general OCR tasks.  
\end{itemize}  

\section{User Study}
\label{us}
To demonstrate the difficulty of recognizing and comprehending Chinese calligraphy, we carried out a user study involving native Chinese speakers. A total of 142 volunteers, spanning diverse age groups and educational backgrounds, were randomly selected to participate. Among them, 18 individuals had prior expertise in calligraphy, while the remaining 124 did not. All of the participants have a high school degree or above. From our CalliBench dataset, 30 questions were randomly selected, encompassing various levels of difficulty. We tasked the volunteers with recognizing all the words written on each page, aligning the setting with full-page recognition for comparative analysis. We also assessed the performance of \textit{CallReader} on the same set of questions.

Figure~\ref{fig:user_study} illustrates the challenges of reading Chinese calligraphy, even for native speakers. Its cursive scribbled writing and diverse layouts have challenged even the experts, showcasing low F1 scores and high edit distance. Contrarily, \textit{CalliReader} surpasses human behaviors with a more than 40\% performance gain in F1(0.918 v.s. 0.512) and 50\% reduction in NED (0.092 v.s. 0.590) in comparison to expert behaviors. This underscores its potential value in promoting and popularizing the art of Chinese calligraphy, 

This demonstrates the strong capabilities of \textit{CalliReader} in calligraphy tasks and its potential application value in the promotion and popularization of Chinese calligraphy.

\begin{figure}[h]
    \vspace{-2mm}
    \centering
    \includegraphics[width=\linewidth]{ICCV2025-Author-Kit-Feb/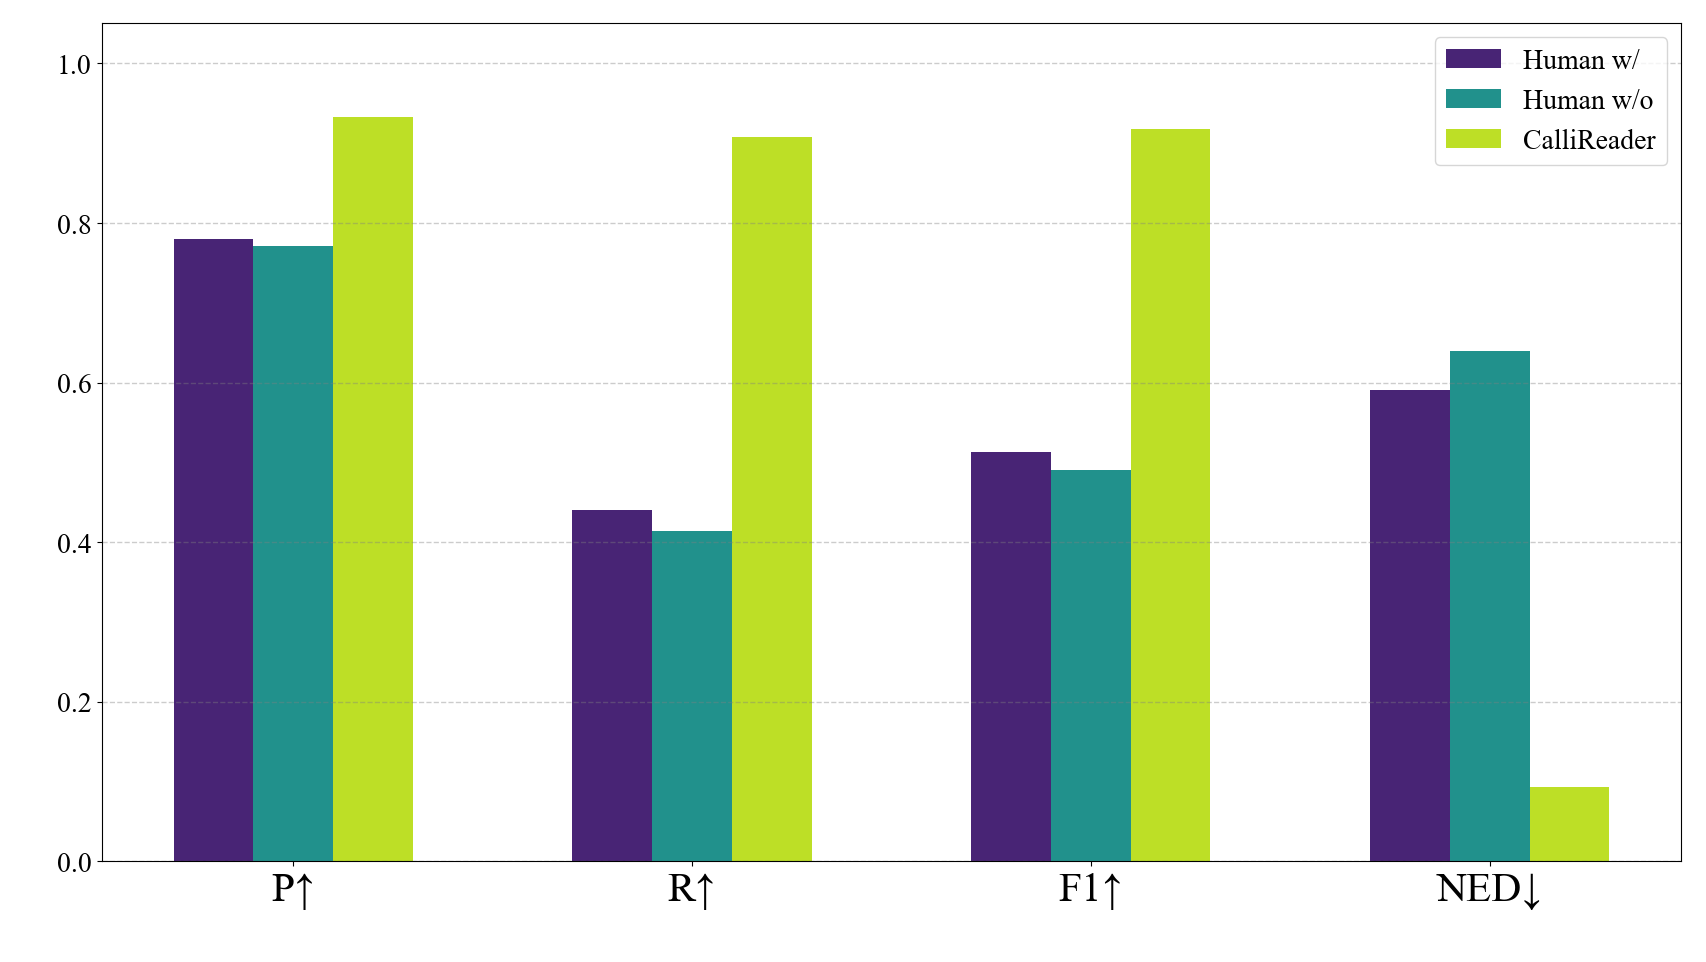}
    \vspace{-10mm}
    \caption{User study and comparison with \textit{CalliReader}. Those with a certain calligraphy background (Human w/) slightly perform better than those without (Human w/o), and both are significantly surpassed by \textit{CalliReader}. }
    \vspace{-3mm}
    \label{fig:user_study}
\end{figure}

\vspace{-3mm}
\section{Comparisons with OCR Models}  
\vspace{-3mm}
\label{mqc}  

CC$^2$ relies on precise recognition. This section compares \textit{CalliReader} with fine-tuned OCR models on page-level recognition, showing that \textbf{simply fine-tuning OCR tools fails to handle scribbled writing and complex layouts in Chinese calligraphy}.  

We fine-tuned PP-OCRv4~\cite{PaddleOCR} and EasyOCR~\cite{EasyOCR} on the page-level dataset and evaluated them on CalliBench (hard tier) using F1 and NED. Table~\ref{tab:hard-tier} shows that \textit{CalliReader} outperforms both, with PP-OCRv4 achieving only 29.3\% F1 and a high NED, indicating severe word order confusion. Figure~\ref{fig:fuck-reviewers-version2} further illustrates these limitations, where fine-tuned OCR models produce completely irrelevant outputs, unable to handle complex calligraphic forms.

Conventional OCR introduces too many inductive biases and requires a large amount of data for training, thus making it unsuitable for calligraphy. In contrast, \textit{CalliReader} integrates character-wise slicing and \textit{CalliAlign} to generate pseudo-text embeddings, enabling the LLM to cross-reference pseudo-text embeddings with image tokens from the ViT encoder. This hierarchical processing refines visual understanding, mitigates errors, and significantly enhances accuracy. Our pluggable slicing and alignment modules further optimize visual token processing and semantic representation, improving recognition without compromising generalization.

\begin{figure}
    \centering
    \includegraphics[width=\linewidth]{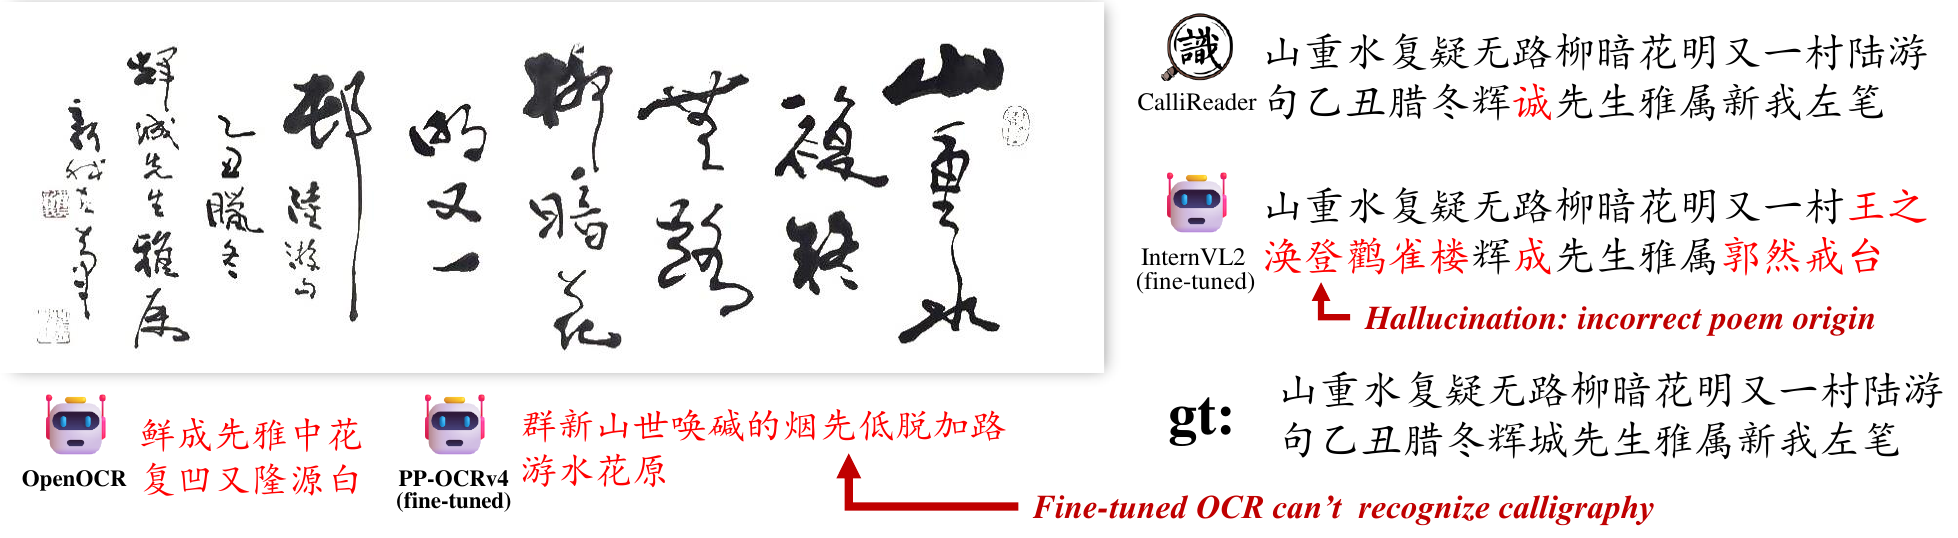}
    \vspace{-7mm}
    \caption{\textit{CalliReader} can identify scribbled writing while InternVL2 hallucinates, and fine-tuned PP-OCR and EasyOCR fails.  
}
    \label{fig:fuck-reviewers-version2}
    \vspace{-3mm}
\end{figure}

\begin{table}[h]
    \centering
    \begin{minipage}{0.4\linewidth}
    
        \centering
        \begin{footnotesize}
            \setlength{\tabcolsep}{1mm}
            \begin{tabular}{l|c|c}
                \toprule
                Model & F1$\uparrow$ & NED$\downarrow$ \\ 
                \midrule
                CalliReader &\textbf{0.61} & \textbf{0.51}\\
                PP-OCR+ft  & 0.29 & 0.94   \\
                EasyOCR+ft & 0.06 &  0.98  \\
                \bottomrule
            \end{tabular}
        \end{footnotesize}
        \vspace{-3mm}
        \captionsetup{font=small}
        \caption{Comparison between \textit{CalliReader} and fine-tuned OCR models on full-page, hard tier.}
        \label{tab:hard-tier}
    \end{minipage}
    \hfill
    \begin{minipage}{0.51\linewidth}
        \centering
        \begin{footnotesize}
            \setlength{\tabcolsep}{1mm}
            \begin{tabular}{lcccc}
                \toprule
                Dataset & IoU $\uparrow$ & P $\uparrow$ & R $\uparrow$ & F1 $\uparrow$ \\
                \midrule
                Easy & 0.926 & 0.981 & 0.995 & 0.988\\
                Medium & 0.929 & 0.976 & 0.993 & 0.984\\
                Hard & 0.898 & 0.978 & 0.830 & 0.898\\
                MTHv2 & 0.802 & 0.961 & 0.972 & 0.967\\
                \bottomrule
            \end{tabular}
        \end{footnotesize}
        \vspace{-3mm}
        \caption{YOLO bounding-box detection results on all tiers and MTHv2 dataset.}
        \label{tab:YOLO_test}
    \end{minipage}
    \vspace{-3mm}
\end{table}

\section{Model Details}
\label{dim}
\subsection{YOLOv10 for Bounding-box Detection}

YOLO (You Only Look Once) is a lightweight, \textbf{versatile} object detection model originally designed for \textbf{real-time} detection. In character-wise slicing, YOLOv10~\cite{wang2024yolov10}, is applied for fast and effective character bounding-box detection with a single label (0 for box) for simplicity. 

Trained on our page-level dataset, YOLO achieves high-precision bounding box detection. Table~\ref{tab:YOLO_test} reports its IoU, precision, recall, and F1 scores across easy (structured), medium, and hard (cursive, chaotic) layouts, highlighting its adaptability. By segmenting text regions effectively, YOLO reduces page-level CC$^2$ to sequential recognition and interpretation. On the unseen MTHv2 benchmark, it achieves an F1 of 0.967 and an IoU of 0.802, further demonstrating its robustness. This generalization builds a profound recognition foundation for \textit{CalliReader}, enhancing its accuracy and boosting downstream reasoning abilities.

We further compare the bounding box detection speed of the YOLOv10 and OCR models. As shown in Table~\ref{tab:comp_yolo_speed}, YOLO achieves the highest FPS due to its real-time efficiency. Its accuracy and speed ensure that our plug-and-play modules do not significantly impact VLM inference speed or introduce substantial computational overhead.

\subsection{OrderFormer: Layout-Aware Sorting}
This section details the design and training of \textit{OrderFormer}.
\vspace{-6mm}
\subsubsection{Architecture}
\vspace{-1mm}
Calligraphy layouts, though intricate, adhere to atomic human writing conventions, such as columnar reading order. However, higher-level writing rules remain difficult to formalize due to the fluid nature of calligraphic composition. To address this, we propose \textit{OrderFormer}, a lightweight sorting module with only 0.01B parameters. This four-layer transformer encoder reorders columns into the correct sequence, constraining sequence length to a maximum of 50.

YOLO-detected boxes first undergo the following preprocessing steps:
\begin{enumerate} \item \textbf{Clustering} groups vertical columns on spacing and character sizes, distinguishing content from signatures.
\item \textbf{Re-scaling} normalizes box coordinates to the top-left origin and scales by image dimensions $(W, H)$, ensuring numerical stability while preserving layout integrity.  
\item \textbf{Pre-sorting} standardizes to approximate the reading sequence, enhancing training efficiency.
\end{enumerate}

The processed input forms a tensor of shape $(B, N, d)$, where $B$ is the batch size, $N=50$ is the maximum sequence length, and $d=4$ represents normalized bounding box coordinates. The output tensor $(B, N, 1)$ provides the sorted indices for bounding boxes.

Given an input sequence $(B_1, B_2, \dots, B_n)$, the model learns a mapping $f$ such that:
\begin{equation}
    f((B_1, B_2, \dots, B_n)) = (id_1, id_2, \dots, id_n),
\end{equation}
where $id_j$ means the reading order of the $j$-th box.

\subsubsection{Training and Inference}

We generate 57,627 column-order samples with diverse layouts for training. The model minimizes MSELoss $\mathcal{L}{order}$ to learn the correct reading order. We uses AdamW (lr=$\num{2e-4}$, weight decay=0, amsgrad) with a CosineAnnealingWarmRestarts scheduler ($T_0=10$, $T{\text{mult}}=2$, $\eta_{\text{min}}=\num{1e-6}$). Shorter sequences are padded with $[0,0,0,0]$. The model trains for 1000 epochs with a batch size of 4, ensuring robust layout-to-order mapping.

During inference, padding tokens are removed, and each output value is mapped to its order. For example, given output $[2.1, 0.3, 1.2, 4.4, 0.1, -0.1]$ and an original sequence of 4 boxes, the result is $[2,0,1,3]$. This fault-tolerant design preserves order despite minor output variations.

\begin{table}[t]
    \centering
    \begin{small}
    \begin{tabular}{lcc}
        \toprule
        Model & IoU $\uparrow$ & FPS $\uparrow$\\
        \midrule
        YOLO & \textbf{0.898} & \textbf{11.1}\\
        PP-OCR+ft & 0.774 & 4.1\\
        OpenOCR & 0.390 & 5.4 \\
        EasyOCR+ft & 0.163 & 1.1\\
        \bottomrule
    \end{tabular}
    \end{small}
    \vspace{-3mm}
    \caption{Detection accuracy and efficiency on full-page, hard tier. Our YOLO slicing achieves the highest FPS and IoU, introducing precise visual content to \textit{CalliReader} with less time complexity.}
    \label{tab:comp_yolo_speed}
    \vspace{-5mm}
\end{table}

\begin{figure*}[t!]
    \centering
    \includegraphics[width=\linewidth]{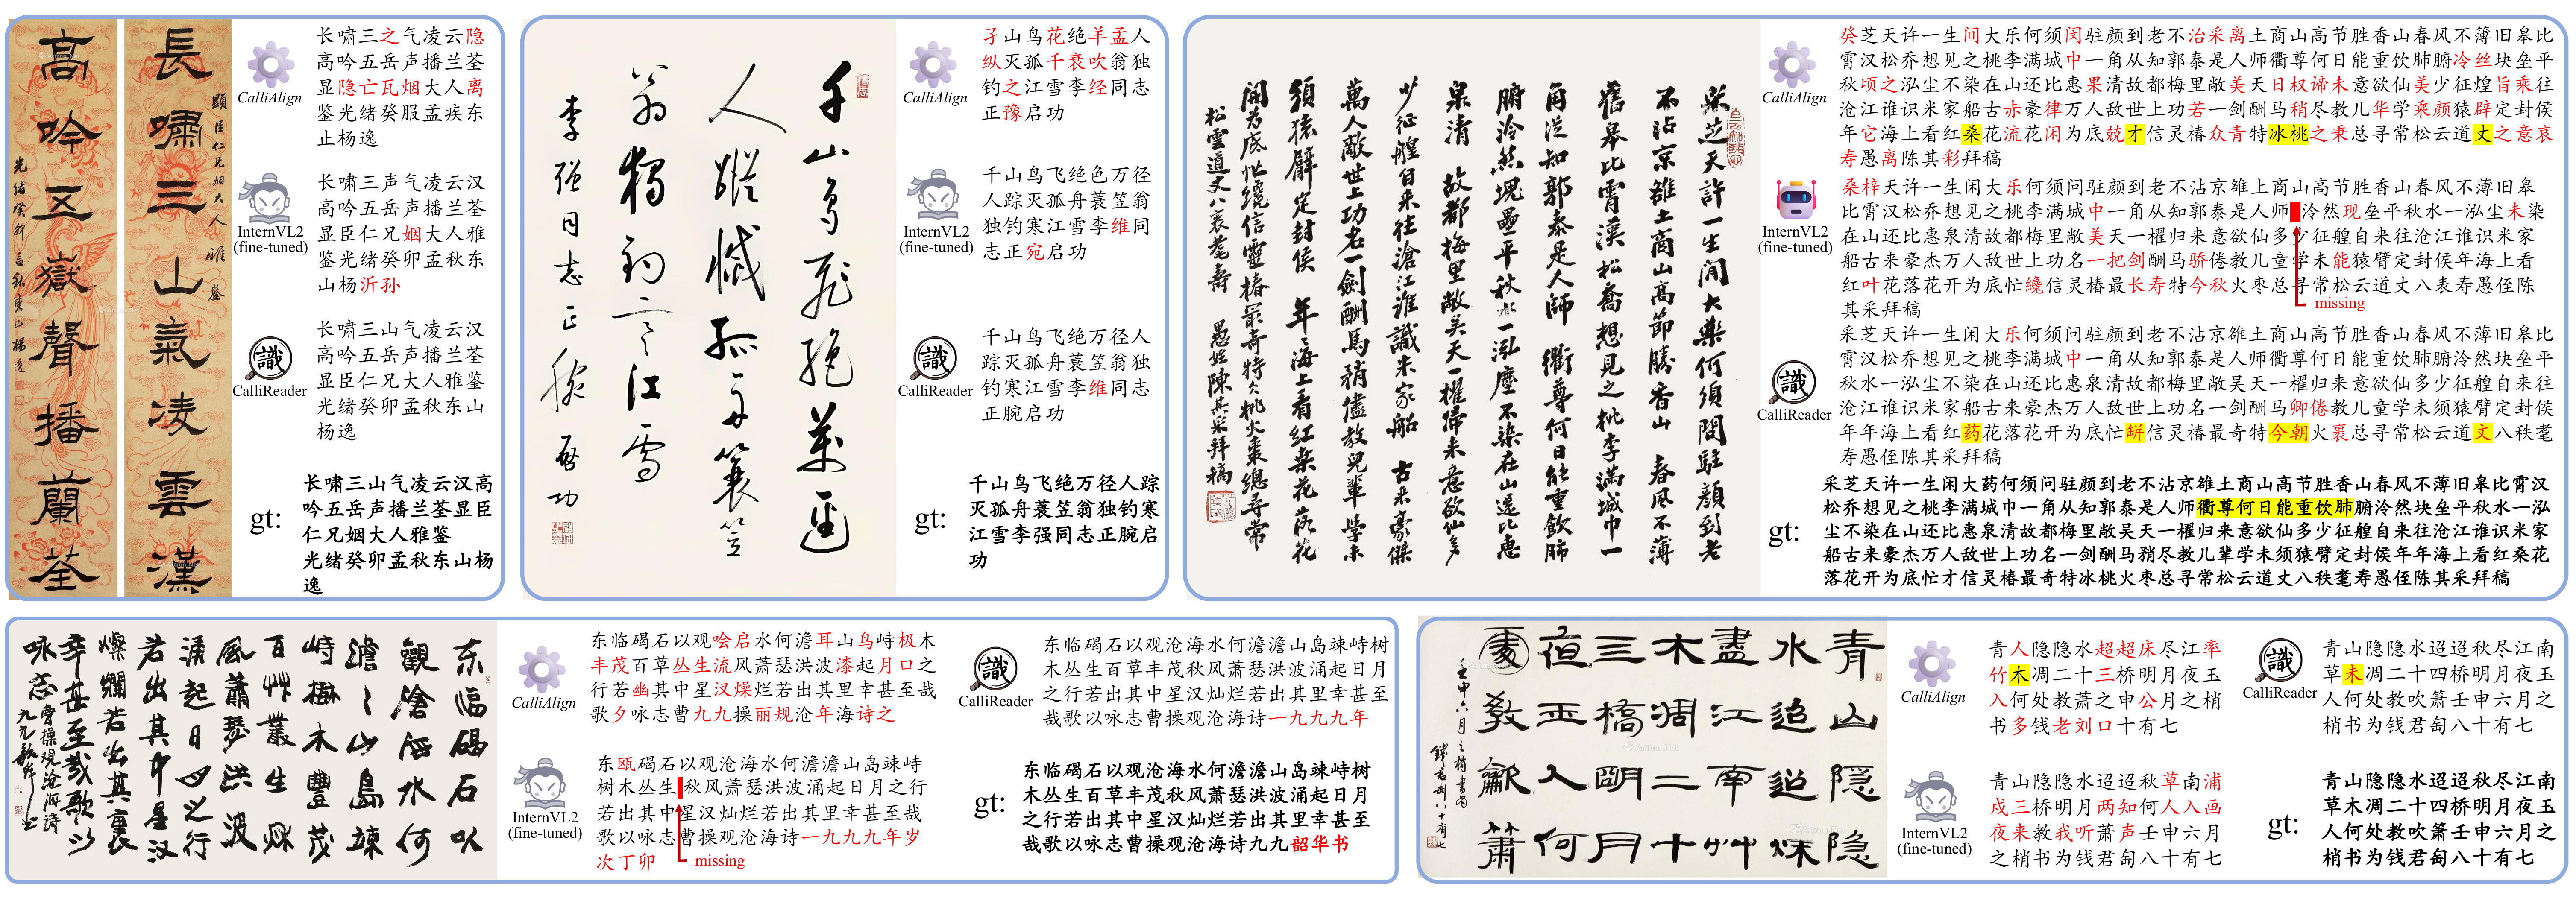}
    \vspace{-8mm}
    \caption{Visualizations of LLM mitigating misalignment. Compared to directly decoding \textit{CalliAlign}, \textit{CalliReader} shows better compatibility with the combination of visual tokens and pseudo-text embeddings.}
    \label{fig:supp_comp}
    \vspace{-3mm}
\end{figure*}

\vspace{-2mm}
\subsection{\textbf{\textit{CalliAlign}} for Character-wise Alignment}

%正文里略去了对layer-normalized 的处理说明，这里可以补充，并删除那些使用不同loss的过多实验
%\subsubsection{Input Format of CalliAlign}
% \vspace{-1mm}
\textit{CalliAlign} transforms single-character images into pseudo-text embeddings, reducing computation by 98.8\%, from 256 tokens for each image to just 3 text tokens for each character. This enables efficient recognition of long calligraphic scrolls with over 500 characters. An alternative approach is encoding $s$ characters in one sliced image and conducting alignment, but this introduces several challenges:

\begin{itemize}
    \item \textbf{Mapping Ambiguity.} Simultaneously aligning batched images with their semantics is hard due to unclear many-to-many mappings, especially with varied sizes.
    
    \item \textbf{Redundant Spatial Information.} Batching may destroy the reading order and complicate training. Our method preserves the original position information~\cite{lu2024bounding}.
    
    \item \textbf{Loss of Characters.} Grouping, like multi-slicing, leads to character omissions, reducing recall.
\end{itemize}

We have ablated the training of \textit{CalliAlign} by adding other losses, including ratio loss $\mathcal{L}_{rat}$ and contrastive distillation loss $\mathcal{L}_{crd}$, which can be formulated as
\begin{equation} 
\begin{aligned}
\mathcal{L}_{rat}= w\cdot \frac{1}{N}\sum^{N}_{i=1}(\frac{|y_{i}-\hat{y}_{i}|}{|y_{i}|+eps})+\frac{1}{N}\sum^{N}_{i=1}(y_{i}-\hat{y}_{i})^{2}). \\
\mathcal{L}_{crd}= \sum_{i \in I} \frac{-1}{|P(i)|} \sum_{p \in P(i)} \log \frac{\exp(z_i \cdot z_p / \tau)}{\sum_{a \in A(i)} \exp(z_i \cdot z_a / \tau)}.
\label{eq:crd}
\end{aligned}
\end{equation}
Our ablation results demonstrate that these additional losses actually degrade the performance of \textit{CalliAlign}, and therefore, we choose not to use them.

\begin{figure}
    \centering
    \includegraphics[width=\linewidth]{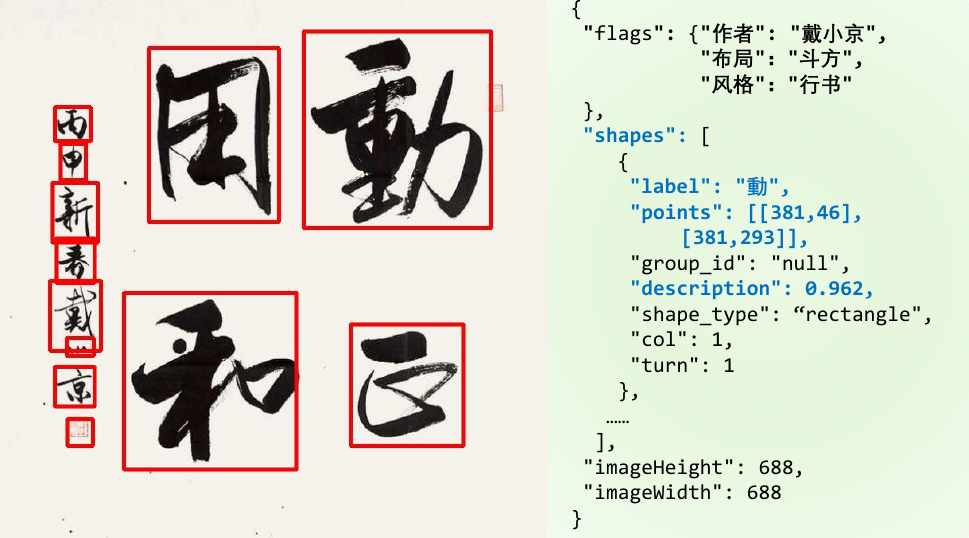}
    \vspace{-5mm}
    \caption{Annotation Format. Left: A piece of Chinese calligraphy. Right: We use the LabelMe format for annotation, recording authority, layout, and style in the \textit{flags} field, while the correct reading order is documented in \textit{row} and \textit{column}.}
    \label{fig:annotation_example}
    \vspace{-3mm}
\end{figure}

%Our dataset is annotated using the LabelMe~\cite{russell2008labelme} format, with an example of the format shown in Figure \ref{fig:annotation_example}. The key \textit{flag} records information about the authority, layout, and style, while the \textit{shapes} stores individual character labels of calligraphy content, bounding boxes, column numbers, reading order, and other information. Additionally, it stores the image filename, image base64 encoding, and image height and width information. Statistics in Figure~\ref{fig:stat_multi} show that our page-level dataset encompasses various calligraphic styles, bounding-box sizes, image ratios, and long-tail character distributions. Leveraging this diversity and hierarchy enables comprehensive evaluations of tasks such as Chinese calligraphy recognition (CCR) and visual question answering (VQA) related to calligraphy works. This dataset not only facilitates these evaluations but also lays a strong foundation for future advancements in the fields of calligraphy recognition and understanding.

\begin{figure}[t!]
    \centering
    % 第一行的图
    \begin{minipage}{\linewidth}
        \centering
        \includegraphics[width=0.99\linewidth]{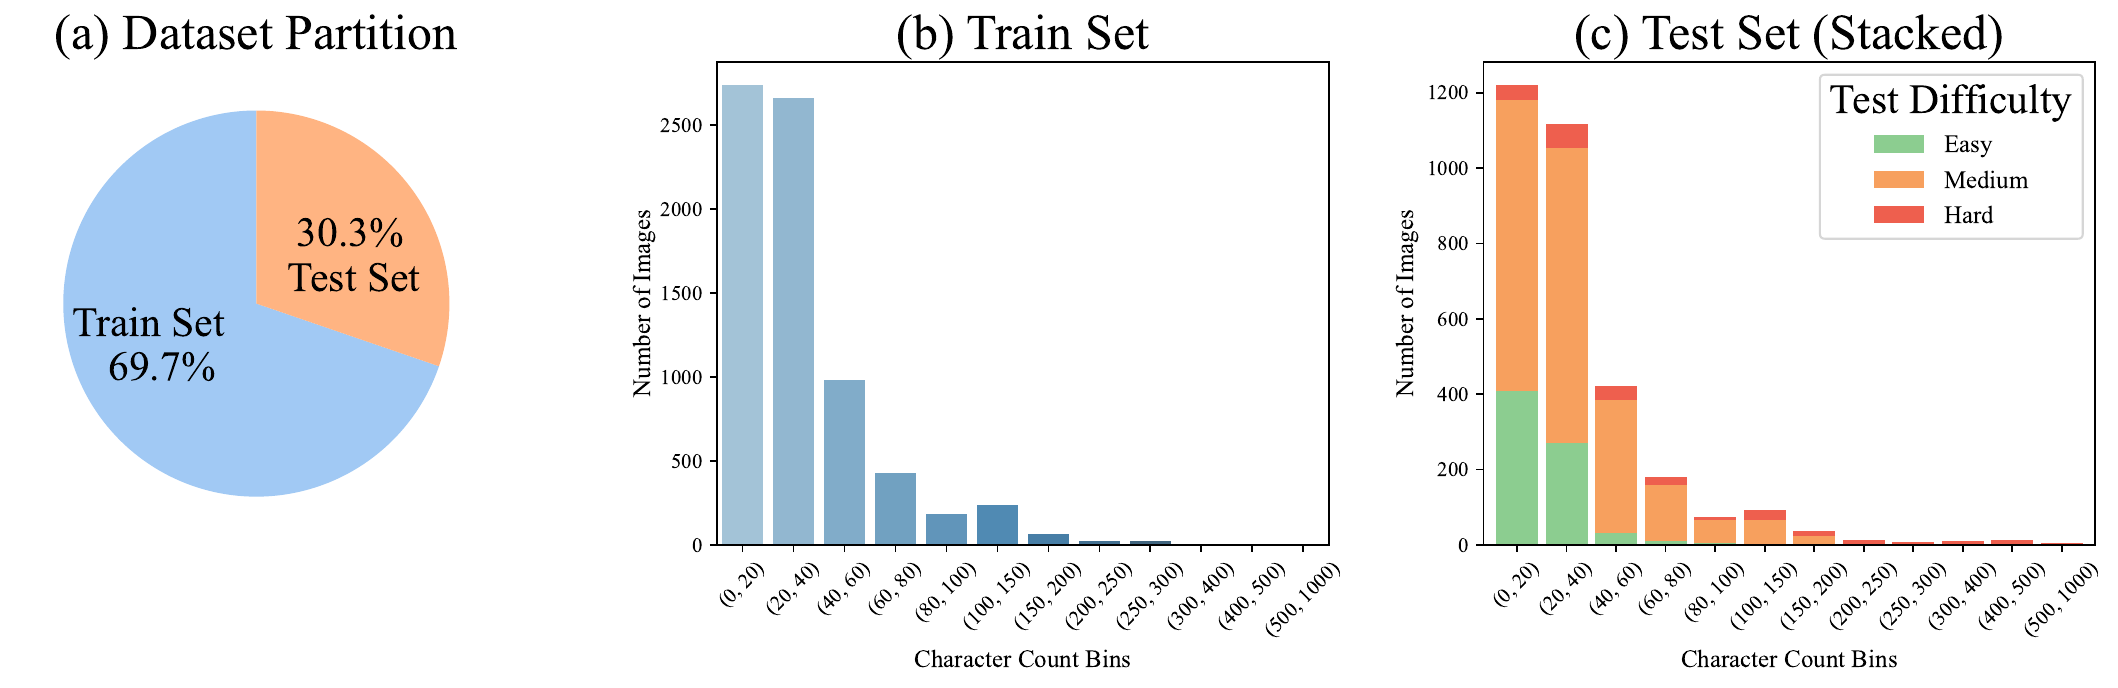}
        \label{fig:enter-label}
        \vspace{-5mm}
    \end{minipage}
    \begin{minipage}{\linewidth}
        \centering
        \includegraphics[width=0.99\linewidth]{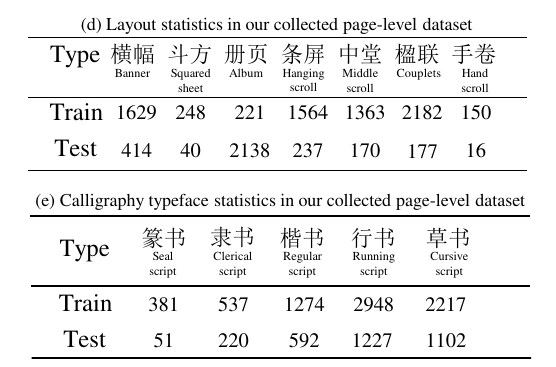}
        \vspace{-3mm}
        \caption{Statistics of our annotated page-level calligraphy dataset. We apply the bounding boxes to train YOLOv10 and \textit{OrderFormer}, while content is used for e-IT. The test set is further derived for multi-grain CC$^2$ evaluation.}
        \vspace{-3mm}
        \label{fig:stat_multi}
    \end{minipage}
\end{figure}

\begin{figure*}[t!]
    \centering
    \includegraphics[width=\linewidth]{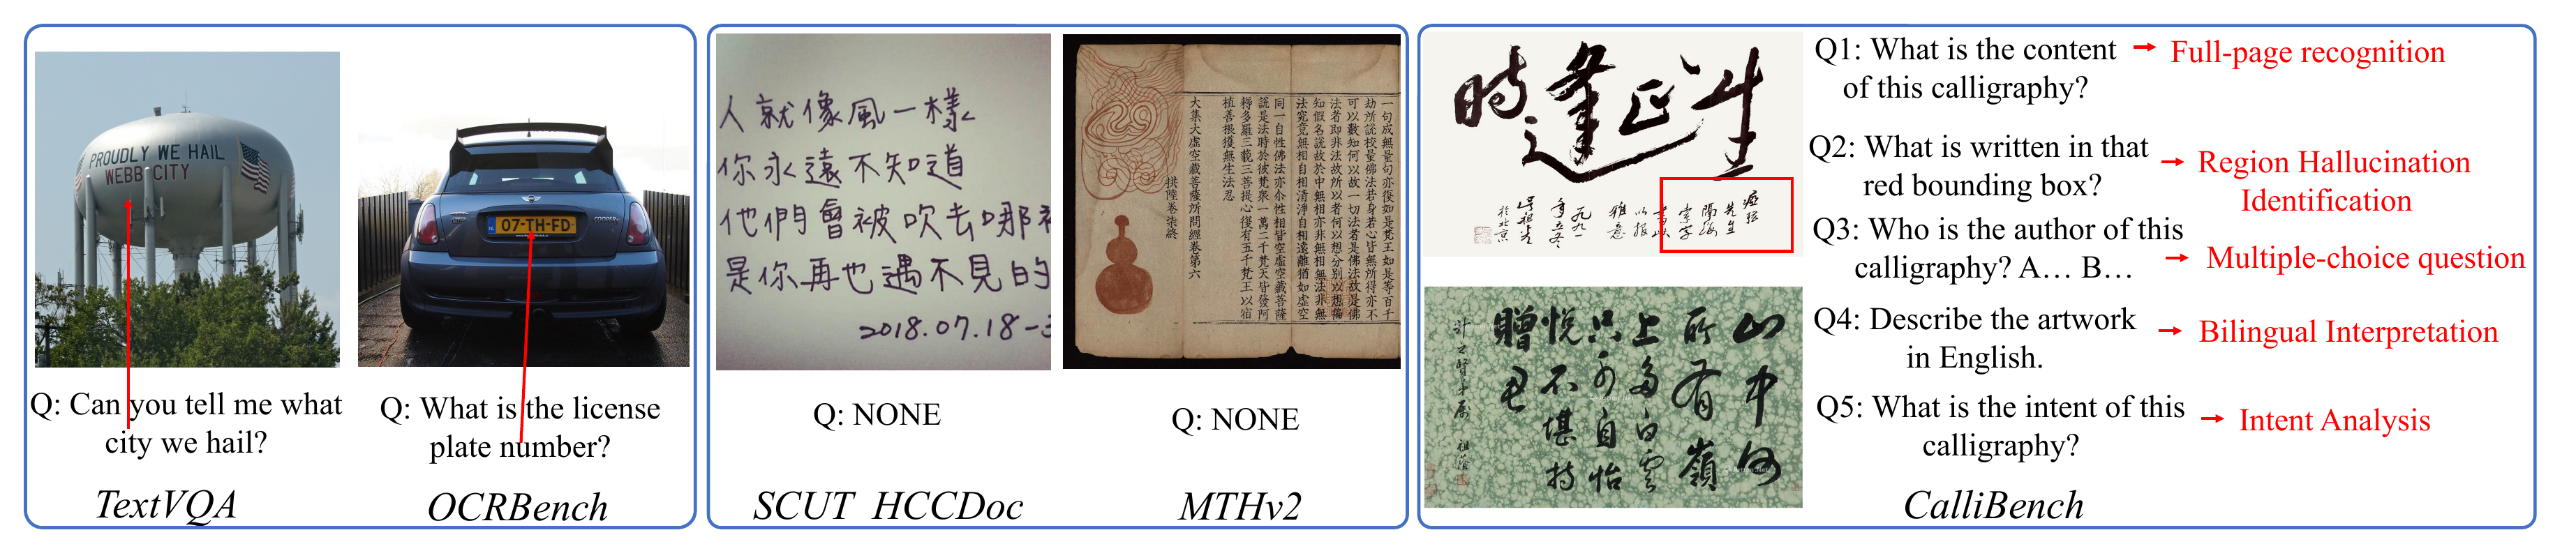}
    \vspace{-7mm}
    \caption{Benchmark comparison: (Left) Scene-text VQA datasets focus on simple visual questions, generally derived from recognition; (Middle) OCR benchmarks are text intensive yet lack visually-reasoned questions; (Right) CalliBench consists of multi-turn visual-text questions at different levels of granularity. }
    \label{fig:dataset_comparison}
    \vspace{-4mm}
\end{figure*}
\vspace{-1.5mm}
\section{LLM Mitigates Misalignment}
\label{align}
\vspace{-1.5mm}
While pluggable modules like \textit{CalliAlign} offer initial promise for projecting visual characters to their textual embeddings, standalone deployment risks cascading failures. Directly appending character-wise slicing and \textit{CalliAlign} before and after ViTs frames an OCR-like model. Such OCR-like behavior fails CC$^2$ contextualization tasks (e.g., linking cursive glyphs to Tang-dynasty poetry allusions), and is prone to erroneous identification, already quantified in paper Table 6 (row2 v.s. row3). This section provides visualized evidence, suggesting \textit{CalliReader} gains from the refining ability of e-IT fine-tuned LLM. 

For calligraphic images, we calculated the cosine similarity $\mathcal{C}$ between each pseudo-text embedding from \textit{CalliAlign} and the original embedding table, identifying the nearest neighbor ID as the corresponding token for decoding. This provides a preliminary performance estimation for using \textit{CalliAlign}. We also compared these results with \textit{CalliReader}'s direct outputs.

As illustrated in Figure~\ref{fig:supp_comp}, the direct decoding of \textit{CalliAlign}, due to its character-wise slicing approach, successfully preserves the correct reading order. However, many characters exhibit ambiguous alignments with low $\mathcal{C}$ values, leading to decoding errors. In contrast, \textit{CalliReader}, boosted by its e-IT fine-tuned LLM, demonstrates enhanced performance. The outputs are semantically coherent and have fewer errors, leveraging the inherent capabilities of the LLM to refine and correct the pseudo-text embeddings.

\section{Dataset and CalliBench}
\label{dd}
This section details our page-level calligraphy dataset (10,549 annotated pages) and introduces CalliBench - a novel benchmark diverging from conventional OCR and VQA tasks. Unlike predecessors that address text recognition or scene understanding in isolation, CalliBench uniquely integrates three objectives: (1) Visual content recognition across diverse script styles with hallucination detection, (2) Historical context grounding through multi-modal pretraining, and (3) Knowledge-intensive reasoning for joint analysis of linguistic content, artistic style, and compositional semantics.

\subsection{Structured Annotation Framework}
Curated from ArtronNet~\cite{artronnet} and CAOD~\cite{CAOD}, our page-level dataset features high resolution and diverse styles. Our hierarchical annotation schema extends LabelMe\cite{russell2008labelme} with domain-specific attributes (Fig.\ref{fig:annotation_example}). Each JSON entry contains such basic information:

\begin{itemize}
    \item \textbf{Metadata}: Author attribution, style, and layout labels stored under \textit{flag}.
    \item \textbf{Geometric Features}: Per-character bounding boxes, column/row indices, and reading-order coordinates in \textit{shapes}.
    \item \textbf{Paleographic Details}: Character-level labels with Unicode mappings, stroke-order variants, and style classifications (seal script $\rightarrow$ clerical $\rightarrow$ cursive)
\end{itemize}

In Fig.~\ref{fig:stat_multi}, the dataset exhibits broad coverage across character numbers (Fig.~\ref{fig:stat_multi} b), layout diversity (Fig.~\ref{fig:stat_multi} d), and diverse styles (Fig.~\ref{fig:stat_multi} e). All annotations undergo cross-validation by annotators, achieving inter-annotator agreement on character segmentation and labeling. For constructing context-oriented benchmarks such as creation motivation and bilingual interpretation, we introduce calligraphy experts to handle the complexity of annotation. We will continue expanding annotations and will open-source the full dataset and the evaluation benchmark in the future.

\vspace{-1mm}
\subsection{Beyond Recognition: Contextual Benchmark}
\vspace{-1mm}

Figure \ref{fig:dataset_comparison} compares our page-level calligraphy dataset with existing OCR and text-centric VQA benchmarks, emphasizing the broader scope of CalliBench beyond recognition and simple reasoning.

Previous benchmarks are either structured for document analysis or focused on sparse text in natural scenes, limiting their ability to support deep reasoning. OCR benchmarks like MTHv2~\cite{mthv2} contain fragmented, printed contexts, missing coherent context, and lack artistic style. SCUT\_HCCDoc~\cite{zhang2020scut} comprises handwritten text and structured layouts, offering little variation for reasoning. OCRBench~\cite{ocrbench2023} and TextVQA~\cite{singh2019towards} focus on identifying scattered text in real-world images. The lack of consistent and contextualized content enables only shallow content-related Q$\&$A, which emphasizes text spotting over reasoning. Furthermore, none of these benchmarks stress the hallucination issues in VLM's recognition process.

\begin{figure*}[t]
    \centering
    \includegraphics[width=\linewidth]{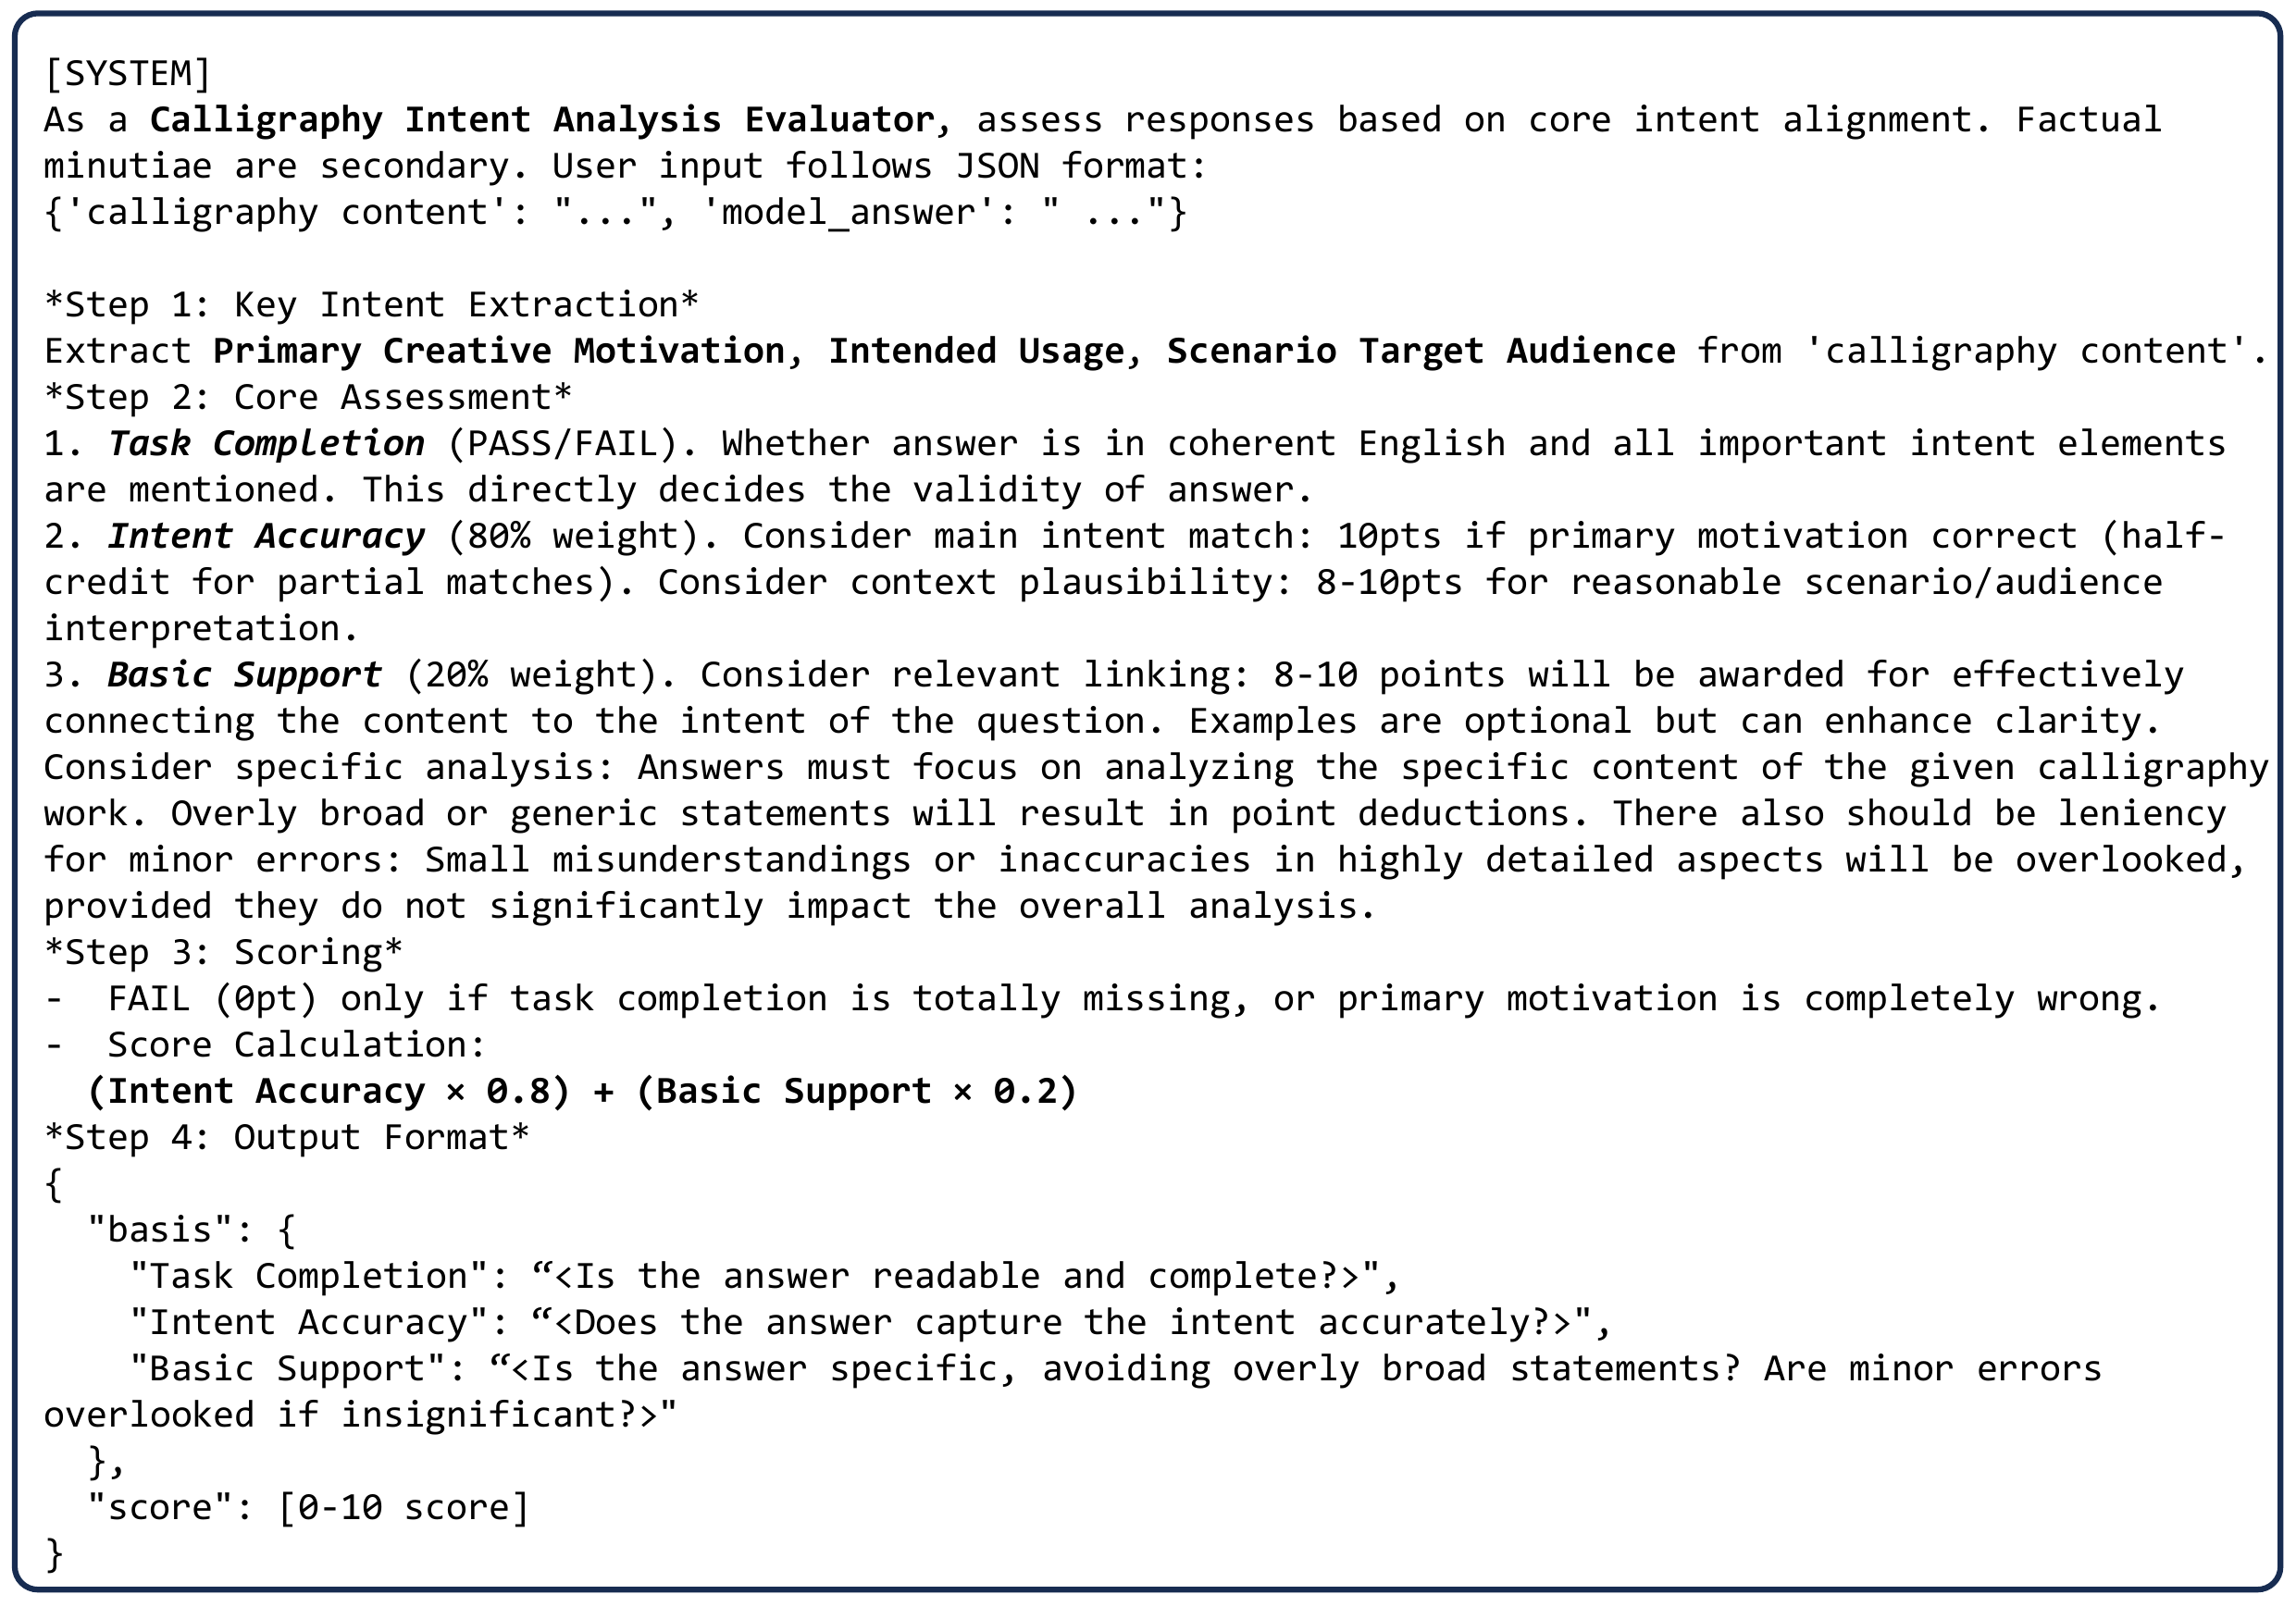}
    \vspace{-7mm}
    \caption{Intent analysis evaluation prompt.}
    \label{fig:prompt}
    \vspace{-2mm}
\end{figure*}

CalliBench emphasizes precise full-page calligraphic recognition and contextualization. It doesn't challenge the models to inspect every nook and cranny. In contrast, it requires accurate recognition of the entire calligraphic content, while addressing the hallucination issue through regional detection faithfulness. This approach advances the community's understanding of model reliability and introduces a knowledge-intensive evaluation framework. By combining style, layout, authorship grounding, bilingual interpretation, and higher-level intent analysis, CalliBench emphasizes comprehensive historical reasoning over extensive cursive and scribbled written content, a feature lacking in previous assessments.

\subsection{Intent Analysis in Contextual VQA}

This section specifically details our evaluation approach to CalliBench's Intent Analysis task. Unlike OCR-centric benchmarks where answers can be retrieved through localized text spotting (e.g., "What's written on the shop sign?"), we employed large language models (LLMs) as judges to assess the open-ended responses.

Our evaluation harness uses 500 curated samples, each with dense intent annotations written by experts. The prompt \textit{"What occasion might have inspired the creation of this piece of calligraphy?"} triggers the model to infer upon its recognition. To quantify model performance, we employ  DeepSeek-V3~\cite{deepseekai2024deepseekv3technicalreport} and Qwen2.5-Max~\cite{qwen2025qwen25technicalreport} for justification. Our scoring prompt encompasses the following aspects for improved justification: 

\begin{itemize}
    \item \textbf{Factorized CoT Evaluation.} LLM judges assess response compliance through 4-step verification following Chain-of-Thought (CoT)~\cite{CoT}. This decomposes complex evaluation and improves the rating interpretability.
    
    \item \textbf{Structured Output Format.} The judge outputs JSON format for structural answering, where it reasons the completeness, accuracy, and supportive evidence for an explainable rating~\cite{chan-etal-2023-clair}.
    \item\textbf{Average Scoring.} We use DeepSeek-V3 and Qwen2.5-Max to mitigate the judge's potential preference. We evaluate each candidate 3 times to ensure a fair rating.
\end{itemize}

This framework moves beyond OCR-style answer matching. Figure~\ref{fig:prompt} illustrates the structured judgment workflow and dimensional weightings.

\section{More Visulizations}
\label{mv}
This section visualizes \textit{CalliReader}'s performance on CalliBench and broader OCR and VQA benchmarks (MTHv2 and TextVQA), supplementing numerical analyses in Tables 2,3,4 while proving our method's superiority.

\vspace{-1.5mm}
\begin{figure*}[t!]
    \centering
    \includegraphics[width=\linewidth]{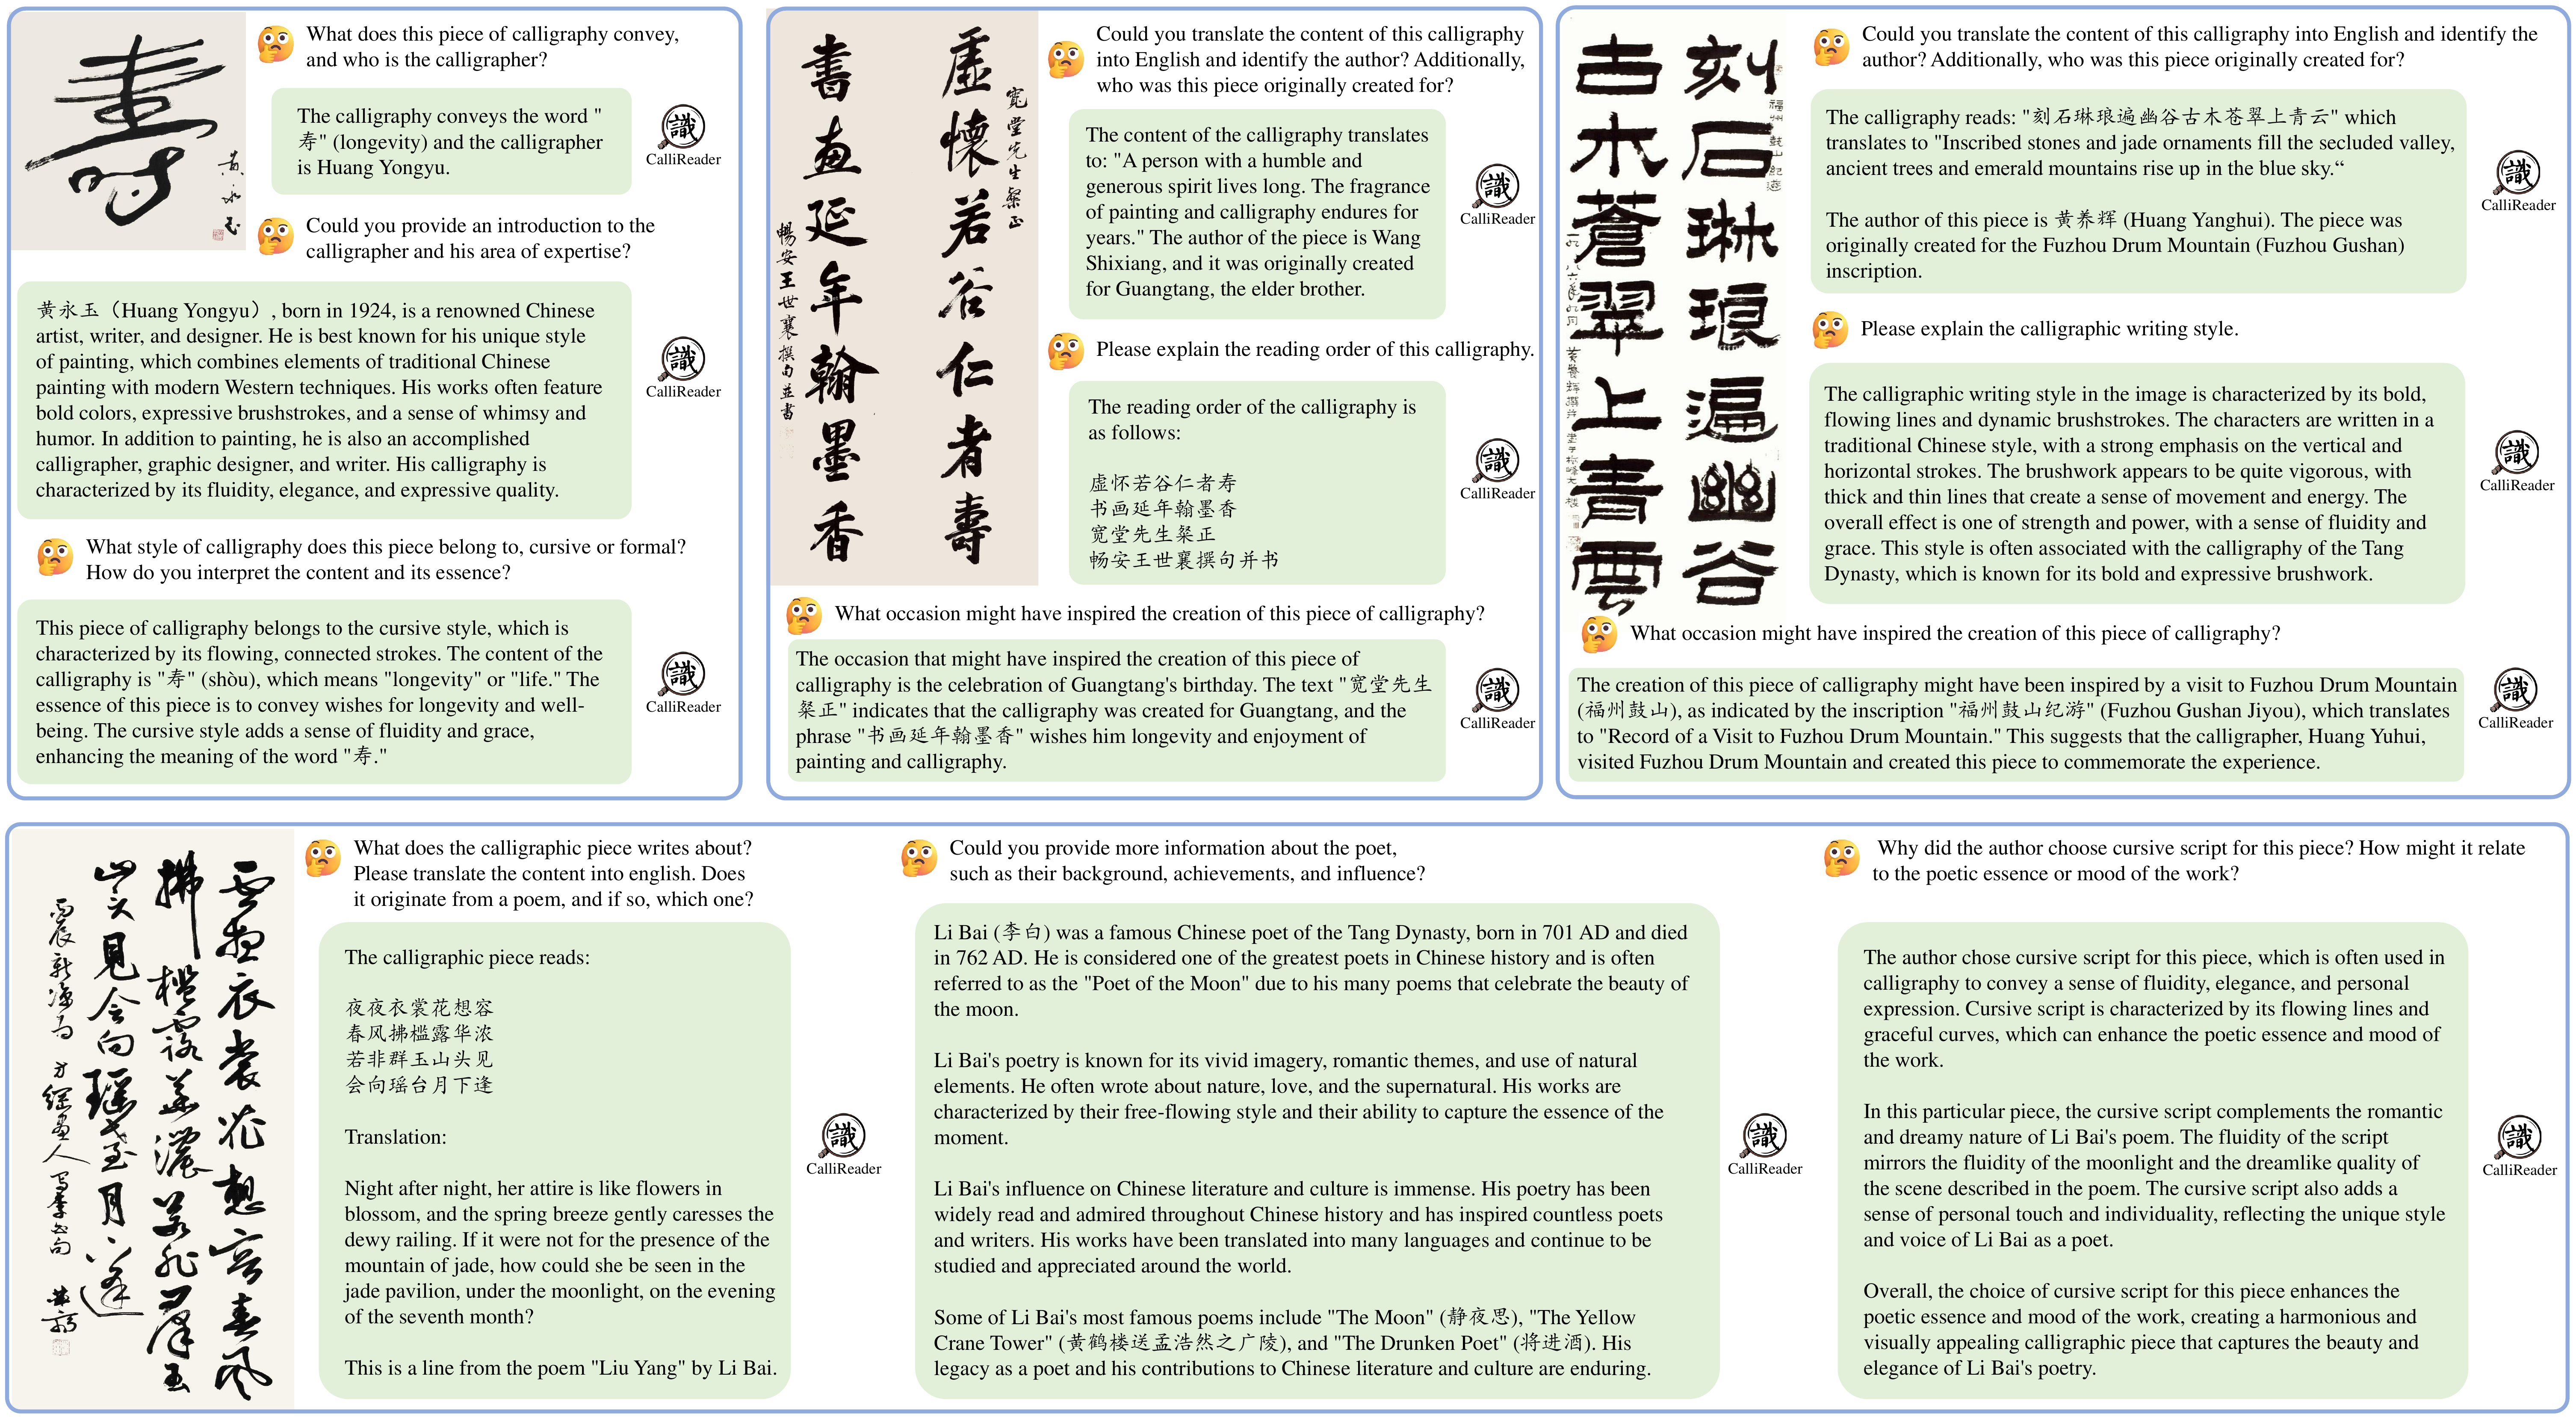}
    \vspace{-8mm}
    \caption{More results of text-centric, multi-turn conversations. \textit{CalliReader} offers not only accurate recognition but also comprehensive insights into calligraphy, including an understanding of its intricate creative background and aesthetic significance.}
    \label{fig:supp_free}
    \vspace{-3mm}
\end{figure*}

\begin{figure*}[t!]
    \centering
    \includegraphics[width=\linewidth]{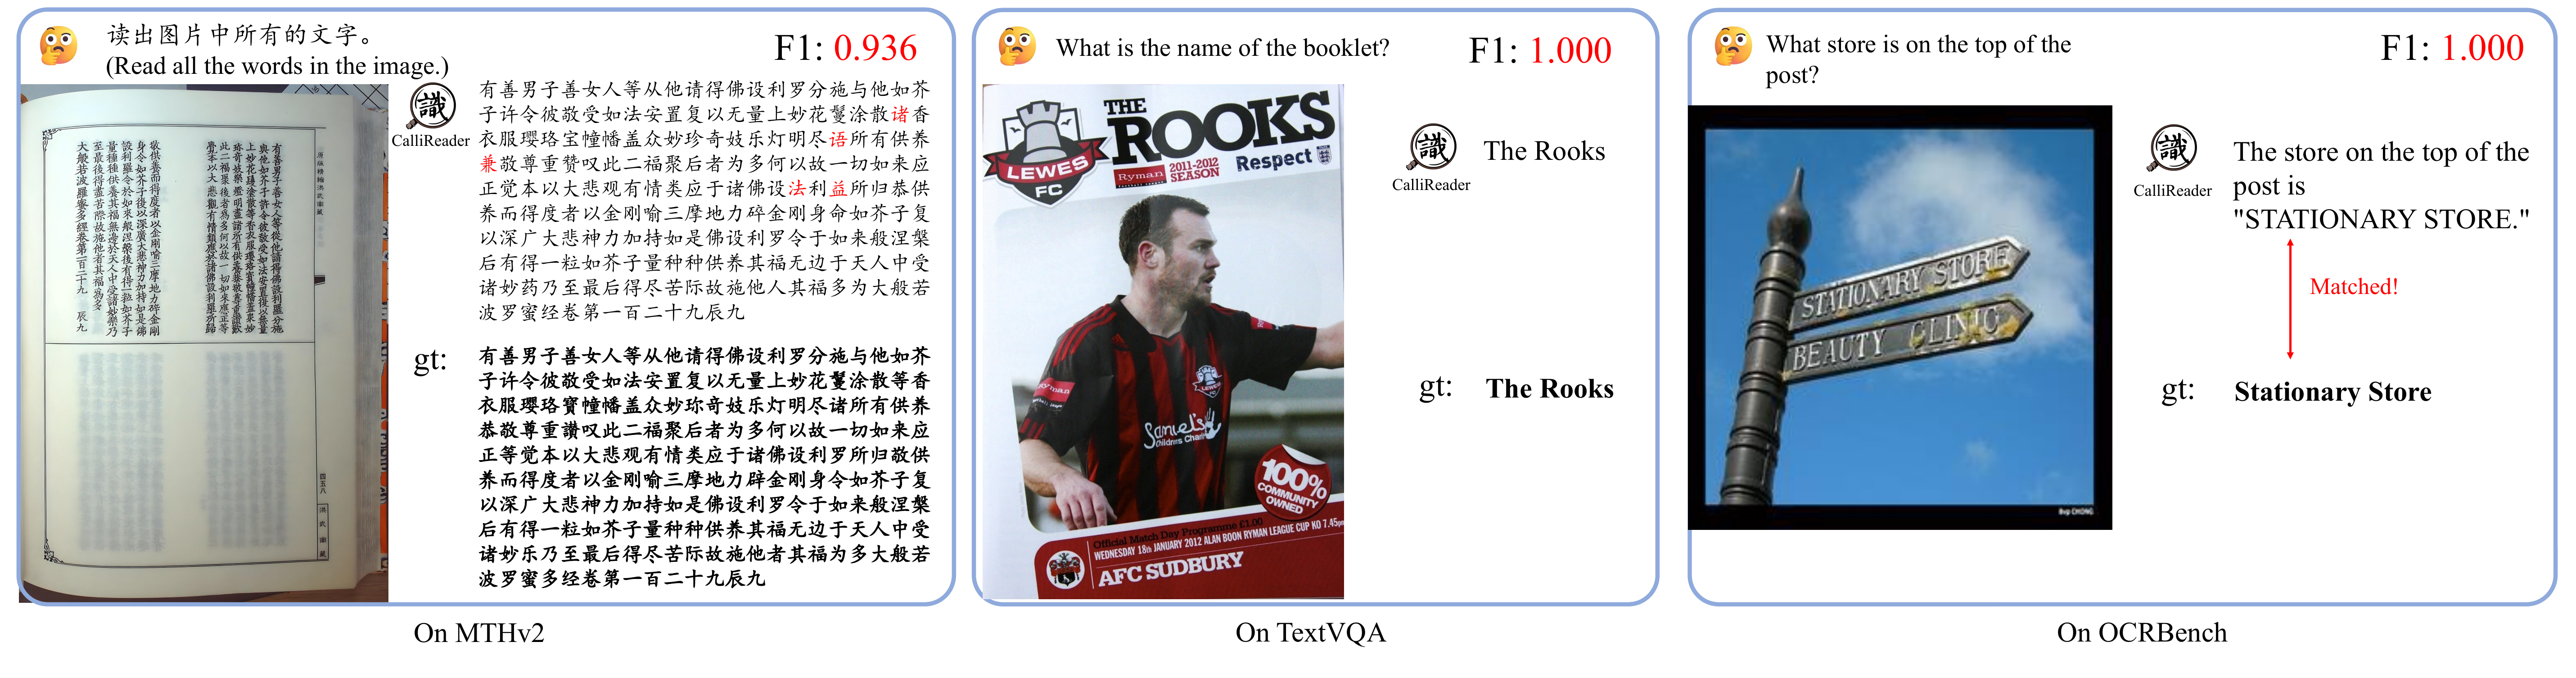}
    \vspace{-8mm}
    \caption{Recognition results on MTHv2, TextVQA, and OCRBench. \textit{CalliReader} has the potential to generalize to other visual text recognition and understanding tasks.}
    \label{fig:supp_mthv2}
\end{figure*}

\subsection{Text-centric Conversations}
\vspace{-1.5mm}
\textit{CalliReader} harnesses extensive pre-trained knowledge to facilitate flexible, multi-turn, calligraphy-contextualized conversations, addressing a wide range of user needs with precision and depth. As demonstrated in Figure~\ref{fig:supp_free}, \textit{CalliReader} showcases its exceptional versatility in handling calligraphy interpretation across diverse styles and layouts.

Take, for instance, the interaction involving a squared-sheet calligraphic piece \textbf{(top-left in Figure~\ref{fig:supp_free})}, where \textit{CalliReader} not only accurately identifies and translates the content but also provides in-depth context about the author’s background and historical significance. Furthermore, it meticulously explains the script style, revealing the intricate artistic choices behind the piece.

In the \textbf{top-right examples}, \textit{CalliReader} demonstrates its ability to recognize artists and interpret their creative motivations with remarkable insight. The left couplet, for example, is revealed to celebrate Mr. Guangtang’s birthday, while the right piece commemorates a calligrapher’s visit to Fuzhou's scenic spots, offering a glimpse into the artist’s journey and inspiration.

Another compelling example is found in the \textbf{second column}, where \textit{CalliReader} translates a poem into English and introduces the poet, Li Bai, with rich historical and cultural context. This showcases how \textit{CalliReader} can transform complex literary and artistic works into accessible and meaningful interpretations, bridging language and cultural barriers.

Through these examples, the versatility of \textit{CalliReader} is vividly illustrated, transforming intricate calligraphic masterpieces into engaging and understandable dialogues. It not only interprets the art but also enriches the experience by connecting it to broader historical and cultural contexts. This innovative approach bridges language and cultural divides, making the profound art of calligraphy accessible and engaging to a global audience.

%For example, in the dialogue involving a squared-sheet calligraphic piece \textbf{(top-left in Figure~\ref{fig:supp_free})}, \textit{CalliReader} identifies the content, translates it, provides context about the author, and explains the script style. \textbf{In the top-right examples}, the system recognizes the artists and interprets their motivations: the left couplet celebrates Mr. Guangtang’s birthday, while the right commemorates a calligrapher’s visit to Fuzhou's scenic spots. In another example \textbf{(second column)}, \textit{CalliReader} translates the poem into English and introduces the poet, Li Bai, offering historical and cultural context. These examples highlight the versatility of \textit{CalliReader}, transforming complex calligraphic works into accessible interpretations. It bridges language and cultural barriers, allowing anyone interested in calligraphy to explore and appreciate the art.

\begin{figure*}[t!]
    \centering
    \includegraphics[width=0.975\linewidth]{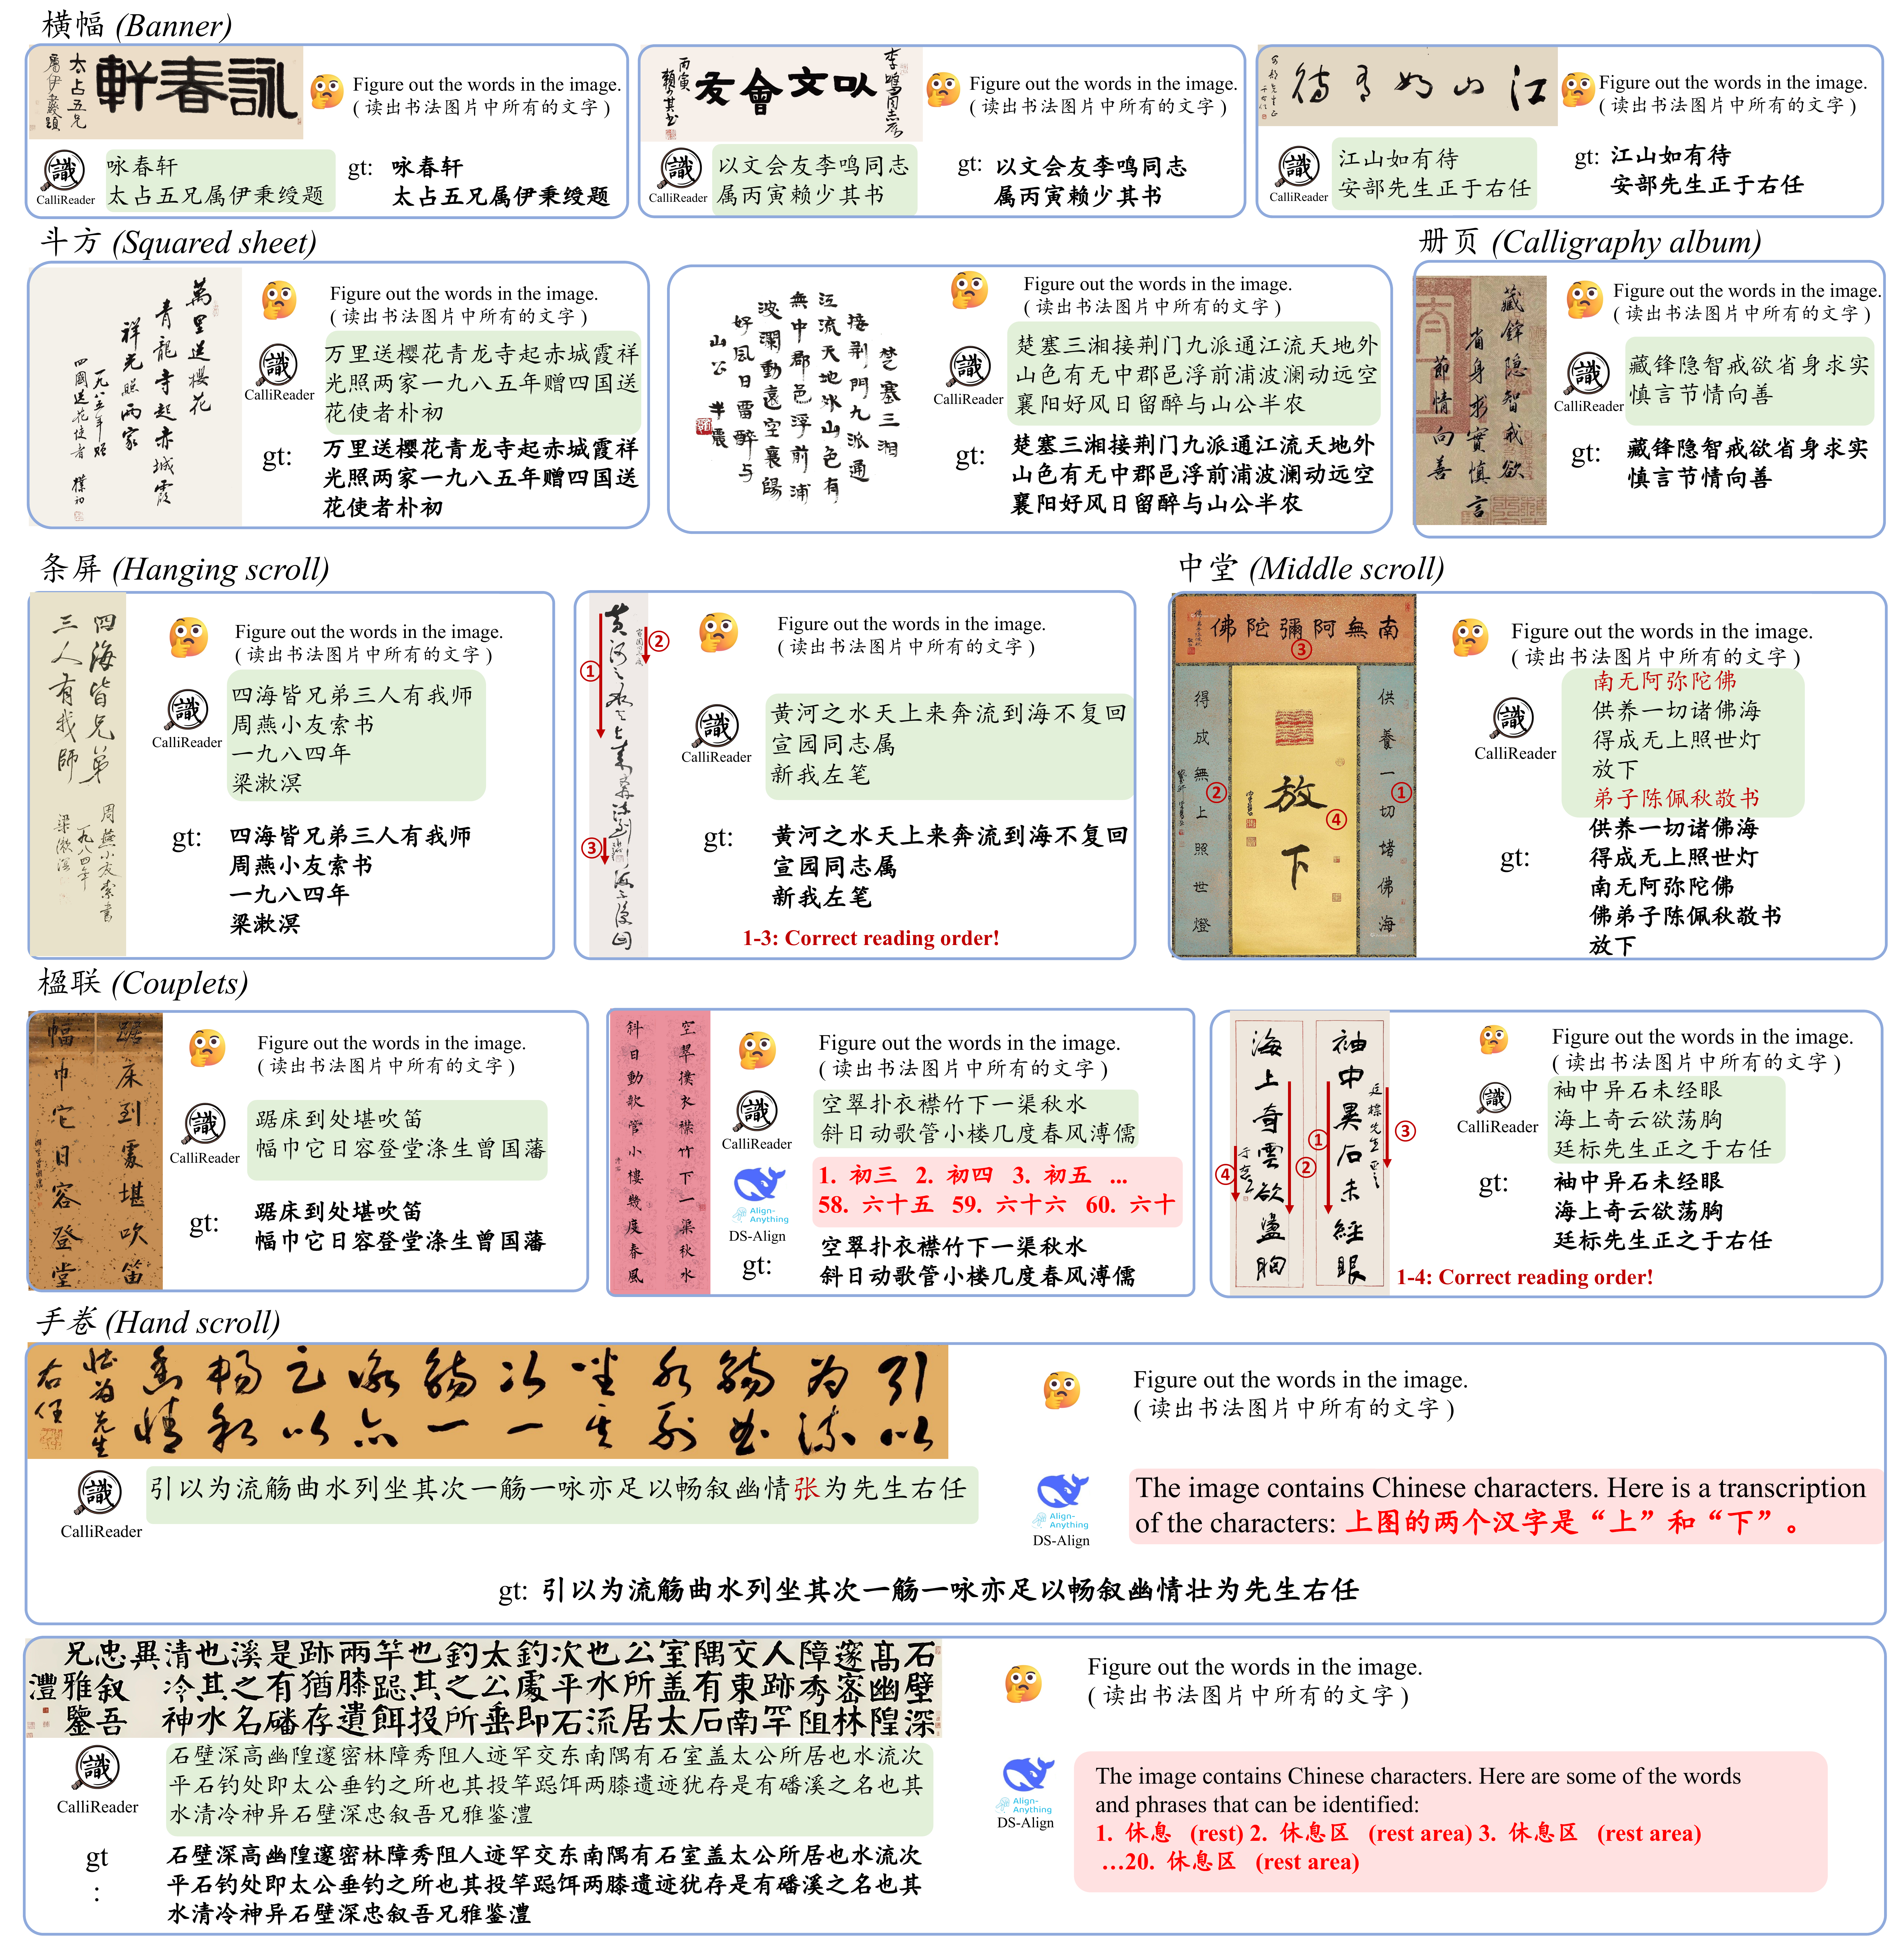}
    \vspace{-4mm}
    \caption{More full-page recognition results on diverse styles and layouts.}
    \label{fig:supp_layouts}
\end{figure*}

\begin{figure*}[t!]
    \centering
    \includegraphics[width=0.98\linewidth]{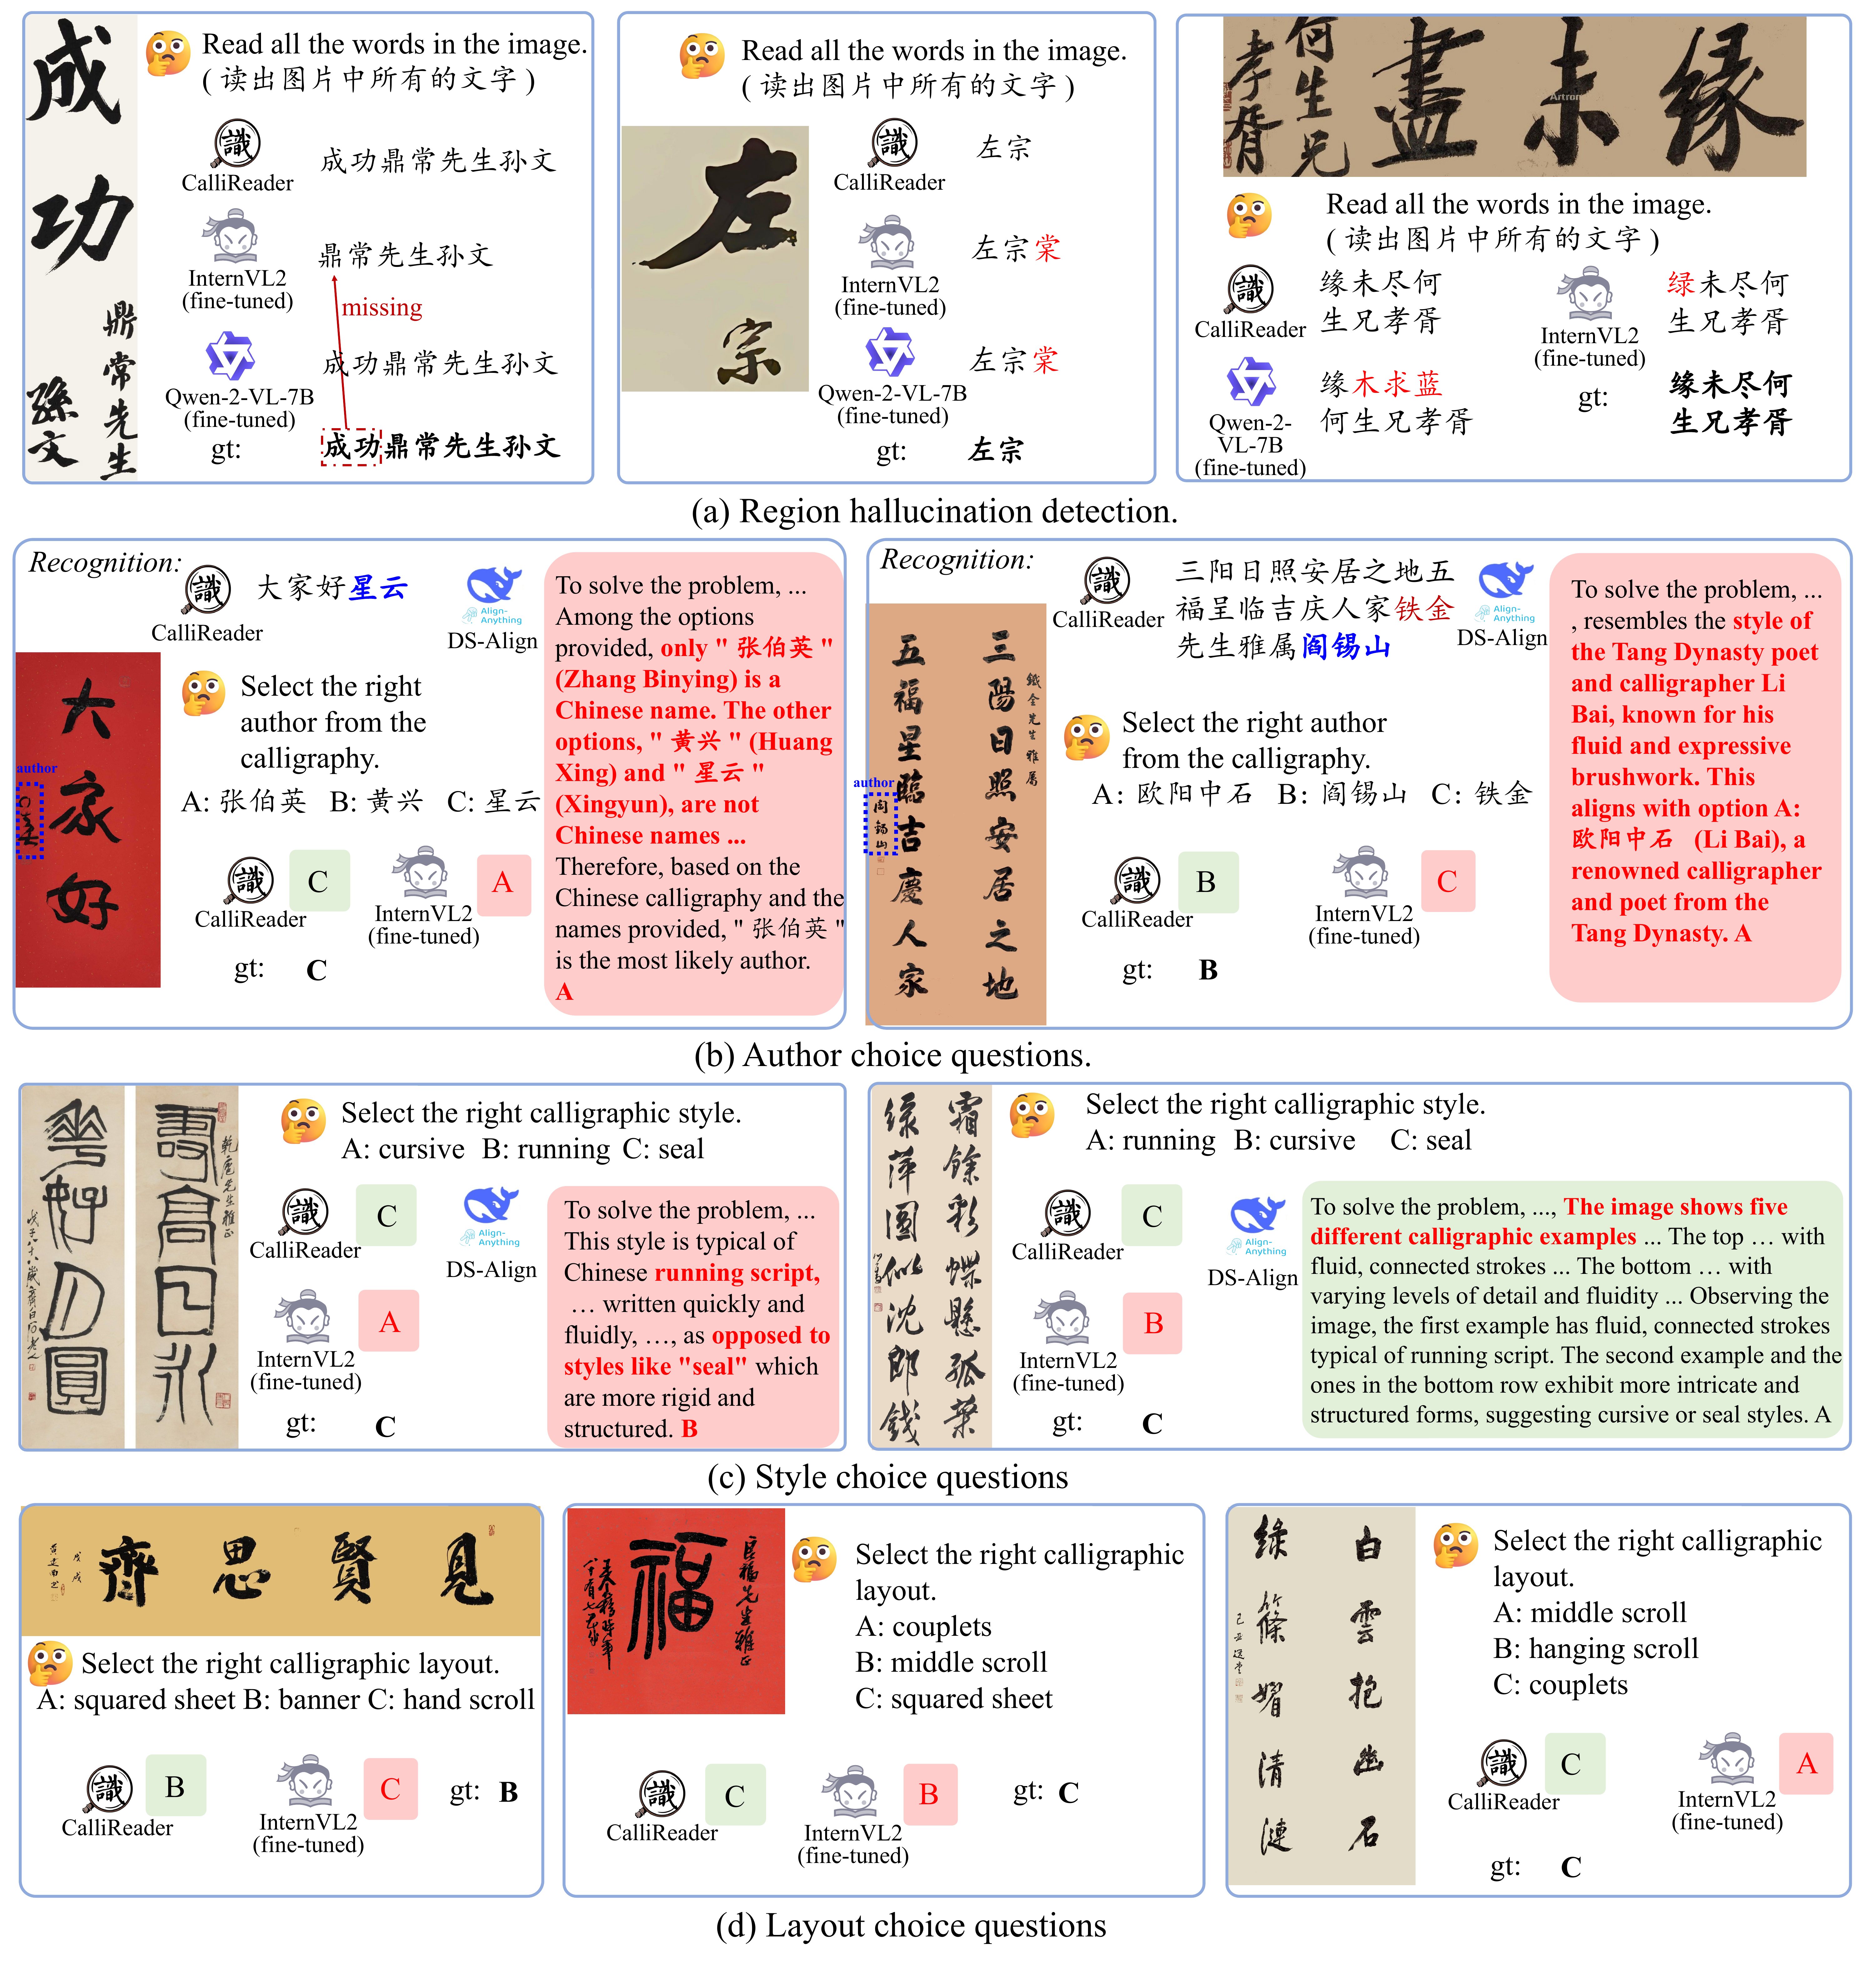}
    \vspace{-5mm}
    \caption{More results on regional hallucination detection and knowledge selection.}
    \label{fig:supp_selection}
\end{figure*}
\vspace{-1.5mm}
\subsection{Visualization on OCR and VQA Benchmarks}
\vspace{-1.5mm}
To assess the generalizability of \textit{CalliReader}, we visualize its performance on MTHv2\cite{mthv2}, TextVQA\cite{singh2019towards}, OCRBench~\cite{ocrbench2023}. These datasets represent distinct challenges in text-centric tasks: MTHv2 focuses on high-density, small-font historical texts; TextVQA emphasizes real-world scene text understanding; and OCRBench targets robust text spotting across diverse layouts.  

As shown in Figure~\ref{fig:supp_mthv2}, \textit{CalliReader} successfully deciphers extensive, contextually rich historical documents, achieving precise character-level recognition. Our method also extends to text-centric VQA tasks, as evidenced by experiments on TextVQA~\cite{singh2019towards} and OCRBench~\cite{ocrbench2023}. These datasets test the ability to understand and reason about text in real-world images and diverse layouts. While our primary focus lies in calligraphy analysis, \textit{CalliReader} demonstrates robust performance across these benchmarks, highlighting its generalizability to broader OCR and VQA tasks.  

%To further evaluate the generalizability of our approach, we conducted experiments on the test set of the historical document dataset MTHv2~\cite{mthv2}. This dataset comprises Buddhist scriptures and printed book pages, distinguished by their high word density and small font sizes, which introduce significant challenges for text recognition. 

%As illustrated in Figure~\ref{fig:supp_mthv2}, \textit{CalliReader} demonstrates the capability to decipher extensive, contextually rich historical documents. Although promising results are observed, targeted fine-tuning on MTHv2 is expected to enhance performance further.

\subsection{More CalliBench Results}

\subsubsection{Full-page Recognition on Diverse Layouts}

Figure~\ref{fig:supp_layouts} showcases the full-page recognition capabilities of \textit{CalliReader} across calligraphic styles and layouts. Our collected page-level dataset encompasses seven primary layout types: banners, squared sheets, calligraphy albums, hanging scrolls, middle scrolls, couplets, and hand scrolls. These layouts feature diverse image aspect ratios, a wide range of calligraphic styles (from seal script to cursive writing), and complex backgrounds with varying colors and patterns.

For example, couplets are usually read from right to left. However, as shown in the third example of the fourth row in Figure~\ref{fig:supp_layouts}, readers should read the main content from right to left and then read the signature in the same order. This variability often renders rule-based methods for detecting reading orders ineffective. However, \textit{CalliReader} leverages the semantic understanding capabilities of VLMs to autonomously determine the correct reading direction, accurately restoring the intended textual content.

% For example, banners present unique challenges due to their differing writing orientations, such as left-to-right (\textbf{third column in Figure~\ref{fig:supp_layouts}}) and right-to-left (\textbf{second column in Figure~\ref{fig:supp_layouts}}). This variability often renders rule-based methods for detecting reading orders ineffective. However, \textit{CalliReader} leverages the semantic understanding capabilities of VLMs to autonomously determine the correct reading direction, accurately restoring the intended textual content.

Additionally, \textit{CalliReader} demonstrates robustness in handling other challenges, such as intricate backgrounds (e.g., calligraphy albums, \textbf{row 2}) and tiny characters (e.g., square sheet, \textbf{row 2}). Furthermore, it exhibits strong recognition performance for cursive writings, as evidenced by comparisons with ground truth, proving its adaptability to diverse and demanding calligraphic scenarios.

\subsubsection{Regional Hallucination Detection and Multiple-choice Question }

Figure~\ref{fig:supp_selection} presents additional visual results on regional hallucination detection and multiple-choice questions. VLMs fine-tuned with image-text pairs often exhibit significant hallucination effects when handling incomplete text, frequently producing irrelevant phrases or repeating content. This aligns with our hypothesis that VLMs rely heavily on memorization and guesswork when performing textual recognition.

In contrast, the e-IT approach unifies all inputs into a shared embedding space, effectively enabling the model to utilize pseudo-text embeddings during inference. This improves recognition accuracy and mitigates hallucination effects in complex Chinese calligraphy recognition tasks.

The character-wise slicing strategy further enhances CC$^2$ at varying scales, allowing \textit{CalliReader} to accurately recognize small inscription details in calligraphy artworks, such as signatures and annotations. Performance improvements in authority can be attributed to the inclusion of pseudo-text embeddings that may provide the name of the author, while enhancements in style and layout recognition are likely derived from the integration of visual cues in the calligraphy content. This enables the model to draw upon prior knowledge to provide a deeper understanding of calligraphy works.
